# Supplementary material for: A predictive machine learning force field framework for liquid electrolyte development
Source: arXiv:2404.07181 source file (2025-04-01)
Supplement: Supplementary file 1 [file ablation.tex]

\section{Ablation Study of Model Architecture}
\label{si:ablation}
In this section, we provide the detailed results of the ablation study in Table \ref{tab:ablation}, and description of the variants of GET (GIT, GE, and GET-no-charge). For GIT, we simply replace the equivariant relative vector $r_{ij} = (x_{ij},y_{ij},z_{ij})$ with an invariant feature $(
(||r_{ij}||,||r_{ij}||,||r_{ij}||)$, which keeps the model architecture. For GE, we skip the transformer architecture as in equation~\eqref{attention} and equation~\eqref{y}, and compute $y_{i}^{n}$ as below: 

\begin{equation}
y_{i}^{n}=\sum_{j}v_{j}^{n}\odot d_{ij}.
\label{bamboo_e}
\end{equation}

In the process of modifying the GET model, when the transformer architecture in the GE is omitted, the dimension of \(x_{i}^{n}\) within GE is increased from 64 to 76. 
Regarding the GET-no-charge variant, all components associated with the charge \(q_{i}\) are eliminated. This includes removing the MLPs that interact with \(q_{i}\). To compensate for the reduction in complexity and to maintain a similar parameter count as the original GET, the number of layers in the \(\text{MLP}^{\text{energy}}\) is increased from 2 to 4. These adjustments ensure that the modified models retain a comparable level of complexity, parameter count, and inference speed to the standard GET.

As shown in Table~\ref{tab:ablation}, GET exhibits superior predictive efficacy for both energy and forces derived from DFT when compared with GE and GIT. This observation intimates that equivariance might play a pivotal role, surpassing that of the transformer, as evidenced by GE's reduced error margins relative to GIT. In the case of GET-no-charge, a significantly elevated error in forecasting DFT energy is noted in comparison to GET. This discrepancy can be ascribed to the intrinsic long-range dependence characteristic of electrostatic energy, which is inversely proportional to distance ($1/r$), coupled with the relatively diminished capacity of GNN to encapsulate long-range interactions as opposed to short-range dynamics~\cite{gnnlongrange}. Pertaining to the prediction of forces, GET-no-charge registers a marginally lower error than GET. This anomaly could potentially be attributed to the inherent limitations associated with the CHELPG method of labelling partial charges~\cite{chelpg}. While electrostatic force exhibits lower sensitivity to long-range information compared with energy ($1/r^{2}$ for force and $1/r$ for energy), CHELPG is calibrated against the electrostatic potential at a considerable distance away from the cluster. Consequently, CHELPG is not optimally designed to capture short-range electrostatic forces. The employment of CHELPG for computing short-range electrostatic forces may inadvertently introduce non-physical biases into the neural network (NN)-facilitated force learning process, thereby exacerbating the learning challenge for the NN with an increase in error. This finding underscores the imperative for the development of more advanced abstract representations of electron density that can accurately and efficiently compute electrostatic forces. Finally, GET is distinguished by its minimal error in modeling density from MD simulations in contrast to GE, GIT, and GET-no-charge, a testament to its overarching superior capability in the precise prediction of DFT-calculated quantities. 

\begin{table}[t]
\caption{Results of ablation study of models trained on DFT data without ensemble knowledge distillation and density alignment. Here, ``number of parameters" is the total number of degree of freedom of each MLFF that can be optimized in the training. ``Density MAE" is based on the 13 systems included in density alignment as in Figure \ref{fig:impact_of_alignment}. Units: Energy: kcal/(mol*atom); Forces: kcal/(mol*\AA); Virial: kcal/mol; density: g/cm$^3$}
\label{tab:ablation}
\vskip 0.1in
\begin{center}
\begin{tabular}{lcccc}
\toprule
 &GET&GIT&GE&GET-no-charge\\
\midrule
Number of parameters & 103,620 & 103,620 & 108,900 & 107,649 \\
Energy RMSE & \textbf{0.245$\pm$0.003} & 0.278$\pm$0.002 & 0.269$\pm$0.003 & 0.812$\pm$0.003 \\
Forces RMSE & 2.19$\pm$0.02& 2.96$\pm$0.02 & 2.32$\pm$0.01 & \textbf{2.01$\pm$0.02} \\
Virial RMSE & \textbf{7.54$\pm$0.05} & 9.41$\pm$0.09 & 7.95$\pm$0.05 & 7.69$\pm$0.09 \\
Density MAE before distillation& \textbf{0.049$\pm$0.007} & 0.114$\pm$0.028 & 0.065$\pm$0.020 & 0.082$\pm$0.033 \\
\bottomrule
\end{tabular}
\end{center}
\vskip -0.1in
\end{table}

To further investigate the difference between GET and GE after density alignment, we perform the same density alignment operation on the GE model as that of the GET model. After alignment, the density MAE of GE decreases from 0.065 g/cm$^3$ to 0.018 g/cm$^3$ for systems in Table S5. Although the density alignment algorithm can significantly decrease the density MAE of GE by 72\%, the MAE of 0.018 g/cm$^3$ of GE is still much higher than that of GET after alignment (0.011 g/cm$^3$). Here, we attribute the difference to the initial density error and the convergence of model finetuning. In density alignment, we use the target pressure change $\Delta P$ to align density from MD and experiment. According to equation~\eqref{linear}, larger density difference $\Delta \ln(\rho)$, larger $\Delta P$. Since GET has smaller density MAE than GE before alignment, the mean absolute $\Delta P$ for GET (477 kcal/(mol*\AA$^3$)) is also smaller than that of GE (832 kcal/(mol*\AA$^3$)). In density alignment, we try to simultaneously change the pressure from MLFF, and confine the MLFF to still approximate DFT by including the initial DFT training loss $L_{\text{training}}$ in the finetuning loss as in equation~\eqref{alignmentloss}. Intuitively, if the target pressure change $\Delta P$ becomes larger, then the finetune process will be harder to converge. After finetune, GE has a larger difference between the target pressure change and the actual change than GET (80 kcal/(mol*\AA$^3$) versus 56 kcal/(mol*\AA$^3$)). Moreover, for GE there is an 28\% energy prediction RMSE increase compared with DFT, 1\% force RMSE increase, and 8\% virial RMSE increase. Compared with that of GET (8\% energy RMSE increase, 1\% forces RMSE increase, and 4\% virial RMSE increase), we can see that the density alignment algorithm deviates GE further away from DFT than GET. These two observations suggest that GE with higher initial density error is harder to be aligned than GET, which might explain why GE performs worse than GET after alignment. The comparison between GE and GET also suggests that density alignment cannot solve everything, and one should make the MLFF before density alignment as accurate as possible for better performance after alignment.

In addition to the significant modifications of model architecture (GIT, GE, and GET-no-charge), we also try GET models with different dimensions of node embedding. When the dimension is decreased to 32, the validation energy RMSE raises 32.3\%, force RMSE 8.6\%, and virial RMSE 15.6\%, and when the dimension is increased to 128, the validation energy RMSE only decreases 2.8\%, force RMSE 8.5\%, and virial RMSE 5.9\%. As a result, we choose the 64 dimensional node embedding in this work for the balance between prediction accuracy and cost. We suggest that, for tasks with higher computational demand, such as MD simulation of polymers, one could choose the GET architecture with smaller model sizes or simplified models such as GE, while for tasks where computational cost is not considerable, such as direct prediction of molecular/materials properties, one could consider the GET model with larger model sizes and cutoff radius, or even more complicated architectures such as the L = 8 EquiformerV2~\cite{equiformerv2} model with millions of parameters. 

As mentioned in the main text, the GET model in this work is inspired by TorchMD-Net~\cite{torchmdnet}. In the following, we introduce the sequential stages of modifications of TorchMD-Net to the final GET model. The first modification of GET in this work compared with TorchMD-Net is the way to compute attention scores. In this work, we connect atoms (nodes in the graph) within the cutoff radius, and when we compute the attention scores $a_{ij}^{n}$, we only consider atom pairs that are connected by edges in the graph. Therefore, we claim that we use an ``attention mechanism on graph'' such that the attention mechanism is applied only on pairs of nodes that are connected in the graph. In TorchMD-Net~\cite{torchmdnet}, the attention scores are computed for all pairs of atoms in the graph. Therefore, we claim that TorchMD-Net uses the ``global attention'' that computes attentions of all pairs of nodes as in the original transformer architecture~\cite{vaswani2017attention}. The main reason for us to use ``attention mechanism on graph'' instead of ``global attention'' is the scaling of computational cost with respect to number of atoms in the graph: for ``attention mechanism on graph'' the scaling is $\mathcal{O}(N)$, while for ``global attention'' the scaling is $\mathcal{O}(N^2)$. The reason behind the use of ``global attention'' in TorchMD-Net might be that it was mainly used in the corresponding paper~\cite{torchmdnet} to predict properties of single molecules where the inference speed is not largely affected by the $\mathcal{O}(N^2)$ scaling, and the reason for us to choose the ``attention mechanism on graph'' is that we primarily use the GET model to perform MD simulations with thousands of atoms, where the $\mathcal{O}(N^2)$ scaling is not affordable.    

Moreover, in this work we use an intermediate vector representation $\Vec{u}_{i}^{ n}$ to incorporate edge vector representation as in equation~\eqref{u}. In TorchMD-Net, $\Vec{u}_{i}^{ n}$ is constructed as below: 

\begin{equation}
\vec u_{i}^{n}=\sum_{j} v_{j}^{n} * \Vec{e}_{ij} + \sum_{j} v_{j}^{n,\text{res}} * \Vec{V}_{j}^{n-1}.
\label{u_torchmd}
\end{equation} Comparing equation~\eqref{u} and~\eqref{u_torchmd}, we can see that equation~\eqref{u_torchmd} has an additional operation $\sum_{j} v_{j}^{n,\text{res}} * \Vec{V}_{j}^{n-1}$, which is essentially a residual connection that adds the node vector representation of the previous layer $\Vec{V}_{j}^{n-1}$ to the intermediate vector representation $\Vec{u}_{i}^{ n}$. This operation is time consuming as it requires additional neural network parameters to generate the second ``value" tensor $v_{j}^{n,\text{res}}$ from the node scalar representation $x^{n}_{i}$, and it sums over all edges in the graph. On the other hand, since the main role of $\vec u_{i}^{n}$ is to introduce the equivariant edge information into the network, we think that the second term in equation~\eqref{u_torchmd} might downplay the importance of the first term, similar to the situation of over-squashing of GNN~\cite{oversquashing}. After we replace equation~\eqref{u_torchmd} with~\eqref{u}, we find that the inference speed increases 24\% for systems with 10,000 atoms, and the energy prediction RMSE decreases 2.9\%, force RMSE increases 4.5\%, and virial RMSE increases 6.9\%. Therefore, we use equation~\eqref{u} to construct $\Vec{u}_{i}^{ n}$ in the GET model in this work to achieve a noticeable acceleration with a moderate drop of prediction accuracy. 

Another modification is about the construction of the edge scalar representation $d_{ij}$. In GET, $d_{ij}$ is computed as in equation~\eqref{edge scalar representations initialization}, while in TorchMD-Net the edge scalar representation is computed separately in each layer as in equation~\eqref{edge_torchmd}:

\begin{equation}
d_{ij}^{n}= \text{SiLU} (W^{d,n}\text{RBF} (\cos{\frac{\pi||r_{ij}||}{r_{\text{cut}}}+1})).
\label{edge_torchmd}
\end{equation} Since the input to compute $d_{ij}^{n}$ is the same ($\text{RBF} (\cos{\frac{\pi||r_{ij}||}{r_{\text{cut}}}+1})$) for each layer $n$, we think that using a single $d_{ij}$ for all layers instead of multiple $\{d_{ij}^{n}\}$s might not significantly degrade prediction performance while achieves considerable acceleration. After replacing equation~\eqref{edge_torchmd} with~\eqref{edge scalar representations initialization}, we find that the inference speed increases 13.1\% for 10,000 atoms while the energy prediction RMSE decreases 0.9\%, force RMSE increases 1.6\%, and virial RMSE increases 4.1\%. Therefore, we use equation~\eqref{edge scalar representations initialization} in the GET model.

The last change is about the input of distance into computing the attention score $a_{ij}^{n}$. In GET, the interatomic distance $||r_{ij}||$ is directly used to compute the attention score as in equation~\eqref{attention}, while in TorchMD-Net, another edge scalar representation $d_{ij}^{\text{a}}$ is constructed as in equation~\eqref{edge scalar attention} to compute the attention score as in equation~\eqref{attention d}:

\begin{equation}
d_{ij}^{\text{a}}= \text{SiLU} (W^{d,\text{a}}\text{RBF} (\cos{\frac{\pi||r_{ij}||}{r_{\text{cut}}}+1})),
\label{edge scalar attention}
\end{equation}

\begin{equation}
a_{ij}^{n}=\text{SiLU}(\langle q_{i}^{n}, k_{j}^{n}\odot d_{ij}^{\text{a}}\rangle).
\label{attention d}
\end{equation} Here, we think that the introduction of $W^{d,\text{a}}$ could not largely increase the capacity of the network, because on the one hand, $W^{d,\text{a}}$ is right before two consecutive SiLU~\cite{silu} non-linear activation functions without any residual connection, which could cause the effect of vanishing gradient~\cite{vanishing} to $W^{d,\text{a}}$ and make the network parameters hard to optimize. On the other hand, when computing the intermediate node scalar representation $y_{i}^{n}$ as in equation~\eqref{y}, $W^{d}$ already serves the role of transforming distance information to compute $y_{i}^{n}$. After we replace equation~\eqref{attention d} with~\eqref{attention}, we find that the inference speed increases 18\% for systems with 10,000 atoms, and the energy prediction RMSE decreases 1.4\%, force RMSE decreases 2.6\%, and virial RMSE decreases 3.1\%. Therefore, we switch to equation~\eqref{attention} to compute the attention score.
