# Supplementary material for: A predictive machine learning force field framework for liquid electrolyte development
Source: arXiv:2404.07181 source file (2025-04-01)
Supplement: Supplementary file 2 [file alignment.tex]

\section{Density Alignment}
\label{si:alignment}
\subsection{Theory}
In this work, we propose a physics-inspired approach to align the density predictions from MD simulations to experimentally measured density of liquids. The alignment is based on the isothermal compressibility of liquids:

\begin{equation}
    \beta = \frac{1}{\rho}(\frac{d\rho}{dP})_{T},
    \label{compressibility}
\end{equation} where $\beta$ is the isothermal compressibility of a given liquid, $\rho$ is the density of the liquid, and $P$ is the pressure of the system. If we assume $\beta$ of a condensed liquid does not depend on $P$ when $P$ is not extremely high, which is a reasonable assumption in thermodynamics~\cite{constant_compressibility}, then we have:

\begin{equation}
    \Delta \ln(\rho) = \beta \Delta P.
    \label{linear}
\end{equation} 

Equation~\eqref{linear} suggests a linear correlation between $\Delta \ln(\rho)$ and $\Delta P$. This relationship is substantiated in Figure \ref{fig:linear_density}a-m, where the linearity holds across all examined liquids in the density alignment, evidenced by R$^2$ scores equal to or exceeding 0.98. This linear correlation implies that knowing the experimental density of a liquid and its corresponding density from an MD simulation allows us to determine the $\Delta \ln(\rho)$ between the two. Consequently, we can ascertain the $\Delta P$ required to adjust in the MD simulation to align the densities with experimental observations. Moreover, pressure in MD simulation is related to forces:

\begin{equation}
    P = \frac{N_{\text{atoms}}k_{B}T}{V} + \frac{1}{3V}\sum_{1\leq i < j }^{N_{\text{atoms}}}  \langle\Vec{f}_{ij}, \Vec{r}_{ij}\rangle,
    \label{pressureandforce}
\end{equation} where $k_{B}$ is the Boltzmann constant, $T$ is the temperature, and $V$ is the volume of the simulation box. Therefore, we find a bridge between the macroscopic observable density $\rho$ and microscopic quantity pairwise forces $\Vec{f}_{ij}$:

\begin{equation}
    \begin{split}
        \Delta \ln(\rho) &= \beta \Delta P = \beta (\Delta(\frac{N_{\text{atoms}}k_{B}T}{V}) + \Delta(\frac{1}{3V}\sum_{1\leq i < j }^{N_{\text{atoms}}} \langle\Vec{f}_{ij}, \Vec{r}_{ij}\rangle)).
    \end{split}
    \label{alignmentequation}
\end{equation} Since $\Vec{f}_{ij}$ is predicted by neural networks, equation~\eqref{alignmentequation} provides a way to calculate the derivative of density to weights of neural networks, which enables us to align BAMBOO with experimentally measured density.

\begin{figure}
    \centering
    \includegraphics[height=0.92\textheight]{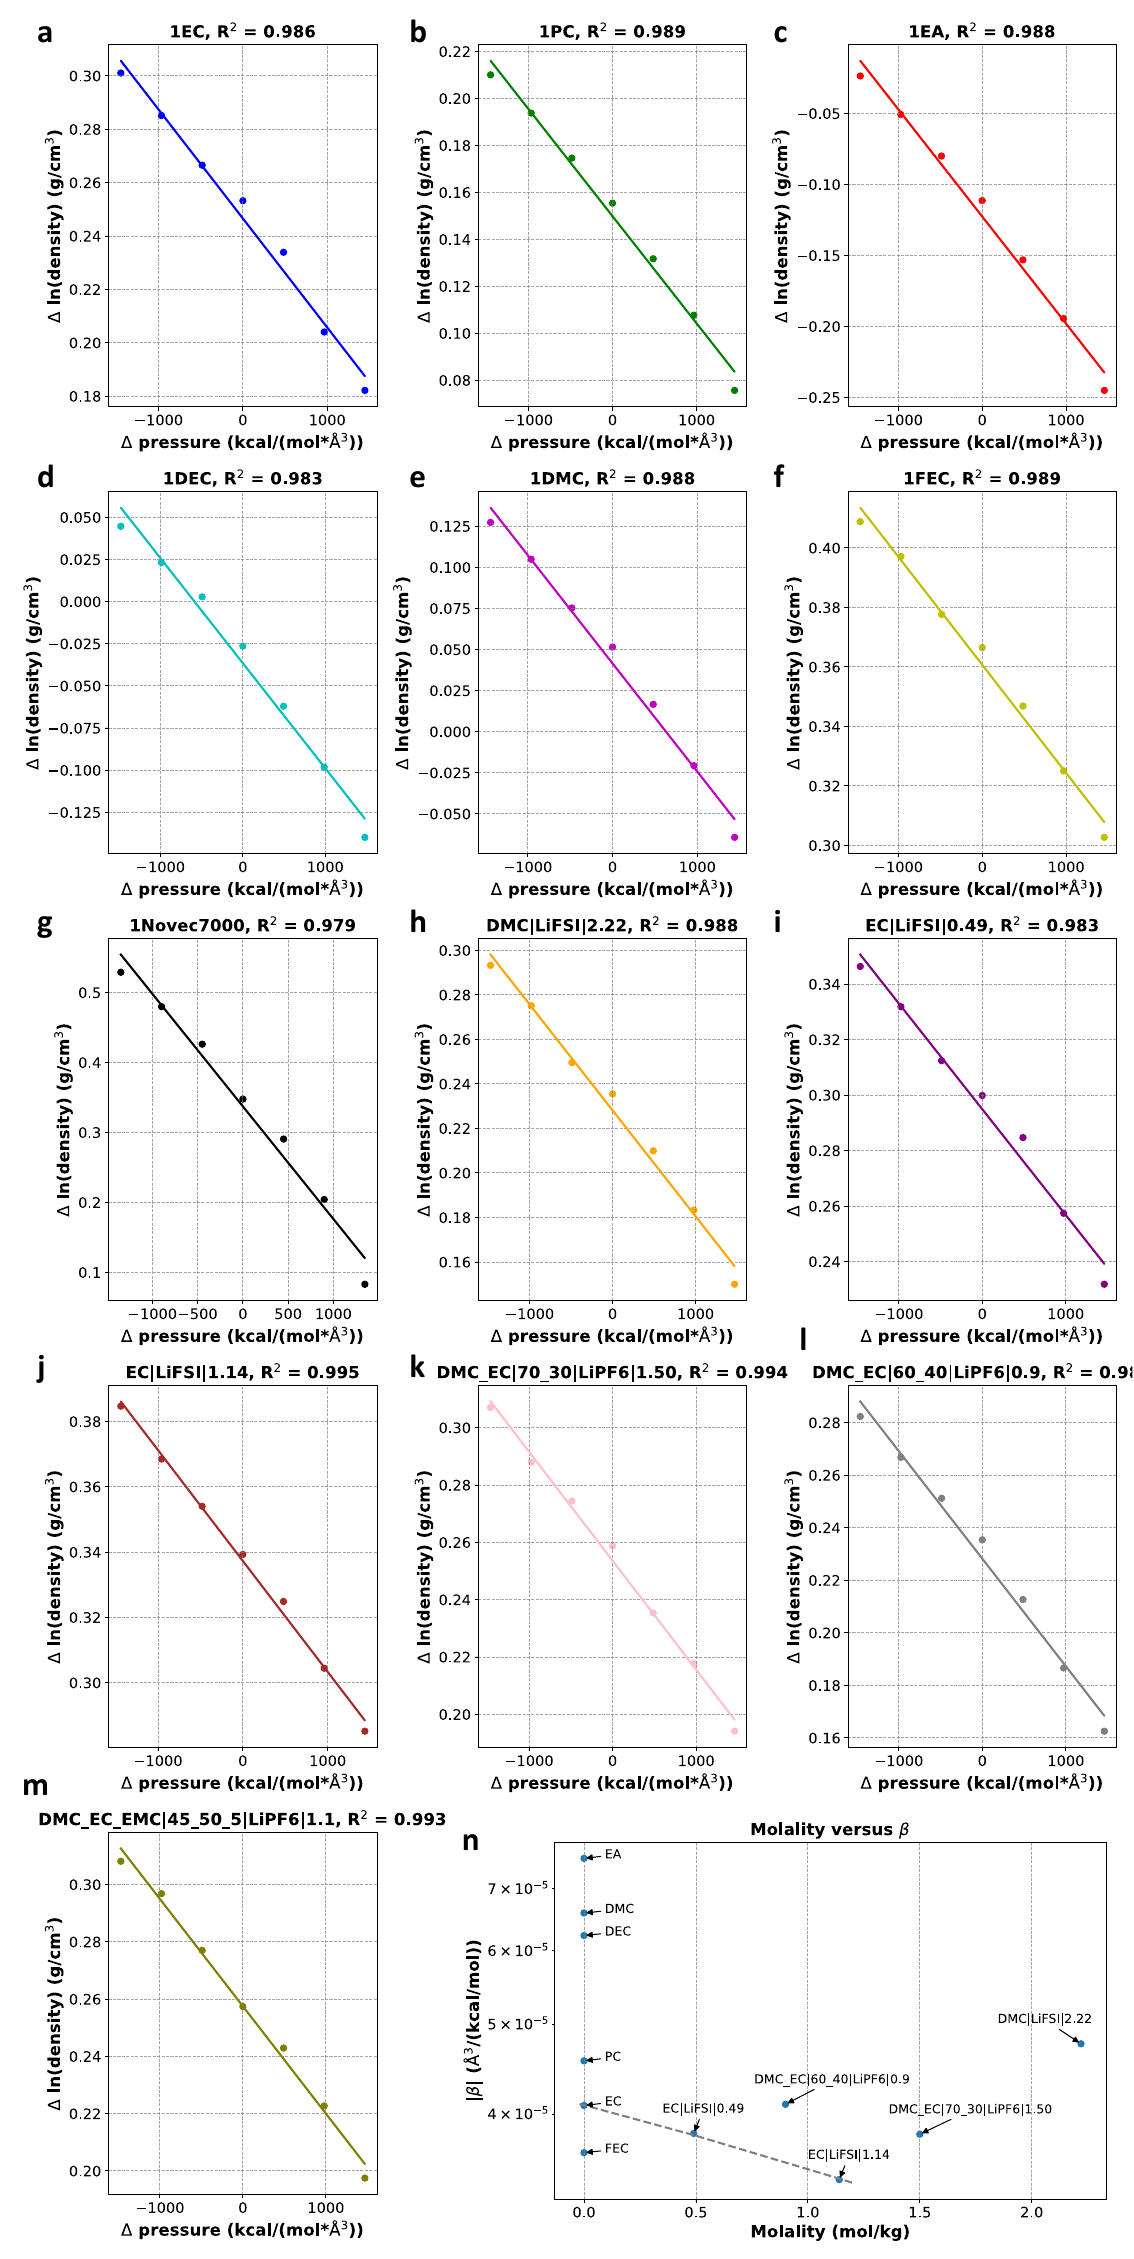}
    \caption{\textbf{\textbf{a}} to \textbf{\textbf{m}} $\Delta$ln(density) versus $\Delta P$ of the 7 molecular liquids and 6 solutions included in density alignment, respectively. \textbf{\textbf{n}} Compressibility $\beta$ derived from the linear relation versus weight of salts.}
    \label{fig:linear_density}
\end{figure}

\subsection{Performance}
As illustrated in Figure \ref{Figure 1}a, we employ the ensemble distilled model as the foundational base model for performing density alignment. This alignment process encompasses 7 molecular liquids and 6 solutions, including 3 with LiPF$_6$ and 3 with LiFSI. To initiate the alignment, we first calculate the coefficient $\beta$ for each liquid. This is achieved by training the distilled BAMBOO to adapt to various $\Delta P$s, utilizing the subsequent loss function:

\begin{equation}
    \begin{split}
         L_{\text{align}} = L_{\text{training}} + \frac{1}{N_{\text{frame}}}\sum_{k}^{N_{\text{frame}}}&(\Delta P - \frac{1}{3V}\sum_{1\leq i < j }^{N_{\text{atoms}}}\langle\Vec{f}_{ij}^{\text{ align}}-\Vec{f}_{ij}^{ \text{ distill}}, \Vec{r}_{ij}\rangle)^{2} \\
         &+ \alpha_{\text{energy}}^{\text{align}} (E_{k}^{\text{align}} - E_{k}^{\text{distill}})^{2} \\
         &+ \sum_{i}^{N_{\text{atoms}}} \alpha_{\text{force}}^{ \text{align}} ||\Vec{f}_{ki}^{ \text{align}} - \Vec{f}_{ki}^{ \text{distill}}||^{2} \\
         &+ \alpha_{\text{virial}}^{\text{align}} ||\textbf{T}_{k}^{ \text{align}} - \textbf{T}_{k}^{ \text{distill}}||^{2}.
    \end{split}
    \label{alignmentloss}
\end{equation} Here, $\Delta P$ is the assigned pressure change as in the x-axes in Figure \ref{fig:linear_density}a-m, $\sum\langle\Vec{f}_{ij}^{\text{ align}}-\Vec{f}_{ij}^{\text{ distill}}, \Vec{r}_{ij}\rangle/(3V)$ is the pressure change of aligned MLFF compared with the base MLFF (we omit the $\Delta(N_{\text{atoms}}k_{B}T/V)$ term in equation~\eqref{alignmentequation} as here we change pressure of the same frames without volume change, and the temperature change should also be negligible if $N_{\text{frame}}$ is large enough). We also include the terms of $(E_{k}^{\text{align}} - E_{k}^{\text{distill}})^{2}$, $||\Vec{f}_{ki}^{ \text{align}} - \Vec{f}_{ki}^{ \text{distill}}||^{2}$, $||\textbf{T}_{k}^{ \text{align}} - \textbf{T}_{k}^{ \text{distill}}||^{2}$, and $L_{\text{training}}$ to ensure that the aligned model would not drastically deviate from the initially trained model and the distilled model. In this work, we reuse the frames generated during the ensemble knowledge distillation for the alignment process as follows.

\begin{enumerate}

\item In the first round of alignment, we apply a uniform $\Delta P$ to each liquid for every model. This approach mirrors the ensemble knowledge distillation methodology, where we specifically adjust the weights of $\text{MLP}^{\text{energy}}$ within the MLFF for optimization. To enhance numerical stability, our focus is solely on the pressure changes stemming from inter-molecular interactions. Consequently, in equation~\eqref{alignmentloss}, we only include $\langle\Vec{f}_{ij}^{ \text{align}} - \Vec{f}_{ij}^{ \text{distill}}, \Vec{r}_{ij}\rangle$, where atoms $i$ and $j$ do not belong to the same molecule or anion.

\item Following the initial alignment phase, we obtain a collection of aligned MLFFs, each corresponding to a distinct $\Delta P$. Utilizing these varied aligned MLFFs, we conduct 600 ps NPT simulations to gather the resulting densities ($\rho$). Consequently, as depicted in Figure \ref{fig:linear_density}a-m, we establish a linear correlation between $\Delta \ln(\rho)$ and the assigned $\Delta P$ for each liquid. Leveraging this linearity, we can determine the $\beta$ value for each liquid. This enables us to identify the specific $\Delta P$ that should be incorporated into the base MLFF for each liquid to align the $\Delta \ln(\rho)$ accurately.

\item In the final step, we employ the loss function specified in equation~\eqref{alignmentloss}, applying the unique $\Delta P$ identified for each liquid, to align the base MLFF with experimental data. This process fine-tunes the MLFF to ensure that its predictions for density closely match the experimental observations, thus enhancing the accuracy and reliability of the model's simulations in reflecting real-world phenomena.
\end{enumerate}

In Figure \ref{fig:linear_density}n, we delve into the examination of the $\beta$ values derived from the linear relationships. It's observed that molecules with similar structures exhibit comparable $\beta$ values. For instance, cyclic carbonates like EC, PC, and FEC share similar $\beta$s, as do linear molecules such as DMC, DEC, and EA. Generally, there is a trend where higher viscosity correlates with lower compressibility, aligning with the intuition that liquids more resistant to shear stress are also more resistant to compression~\cite{compressibity_vs_viscosity}. Additionally, an increase in salt concentration leads to a decrease in $\beta$. For instance, in the case of EC and its solutions with LiFSI at different concentrations, there is a clear linear relationship with an R$^2$ score of 0.998, corroborating the empirical law that a solution's compressibility linearly decreases with an increase in salt molality (more salts result in less compressibility)~\cite{beta_salts}. The consistent compressibility trends, as deduced from density alignment, further confirm the validity of the density alignment approach.

Upon completing the second round of density alignment, the final MLFF is established. Figure \ref{dft_parity} illustrates a slight decrease in the model's predictive accuracy for energy, forces, and virial compared with DFT calculations post-density alignment. Specifically, there is an 8\% increase in the root mean square error (RMSE) for energy predictions, a 1\% rise in forces RMSE, and a 4\% uptick in virial RMSE. Despite these increases, the adjustments are made to enhance the model's accuracy in density predictions, which can be critical for certain applications. Detailed documentation of the training process for density alignment is accessible in the publicly available source code \cite{BAMBOOGITHUB}.

\begin{figure}
    \centering
    \includegraphics[height=0.93\textheight]{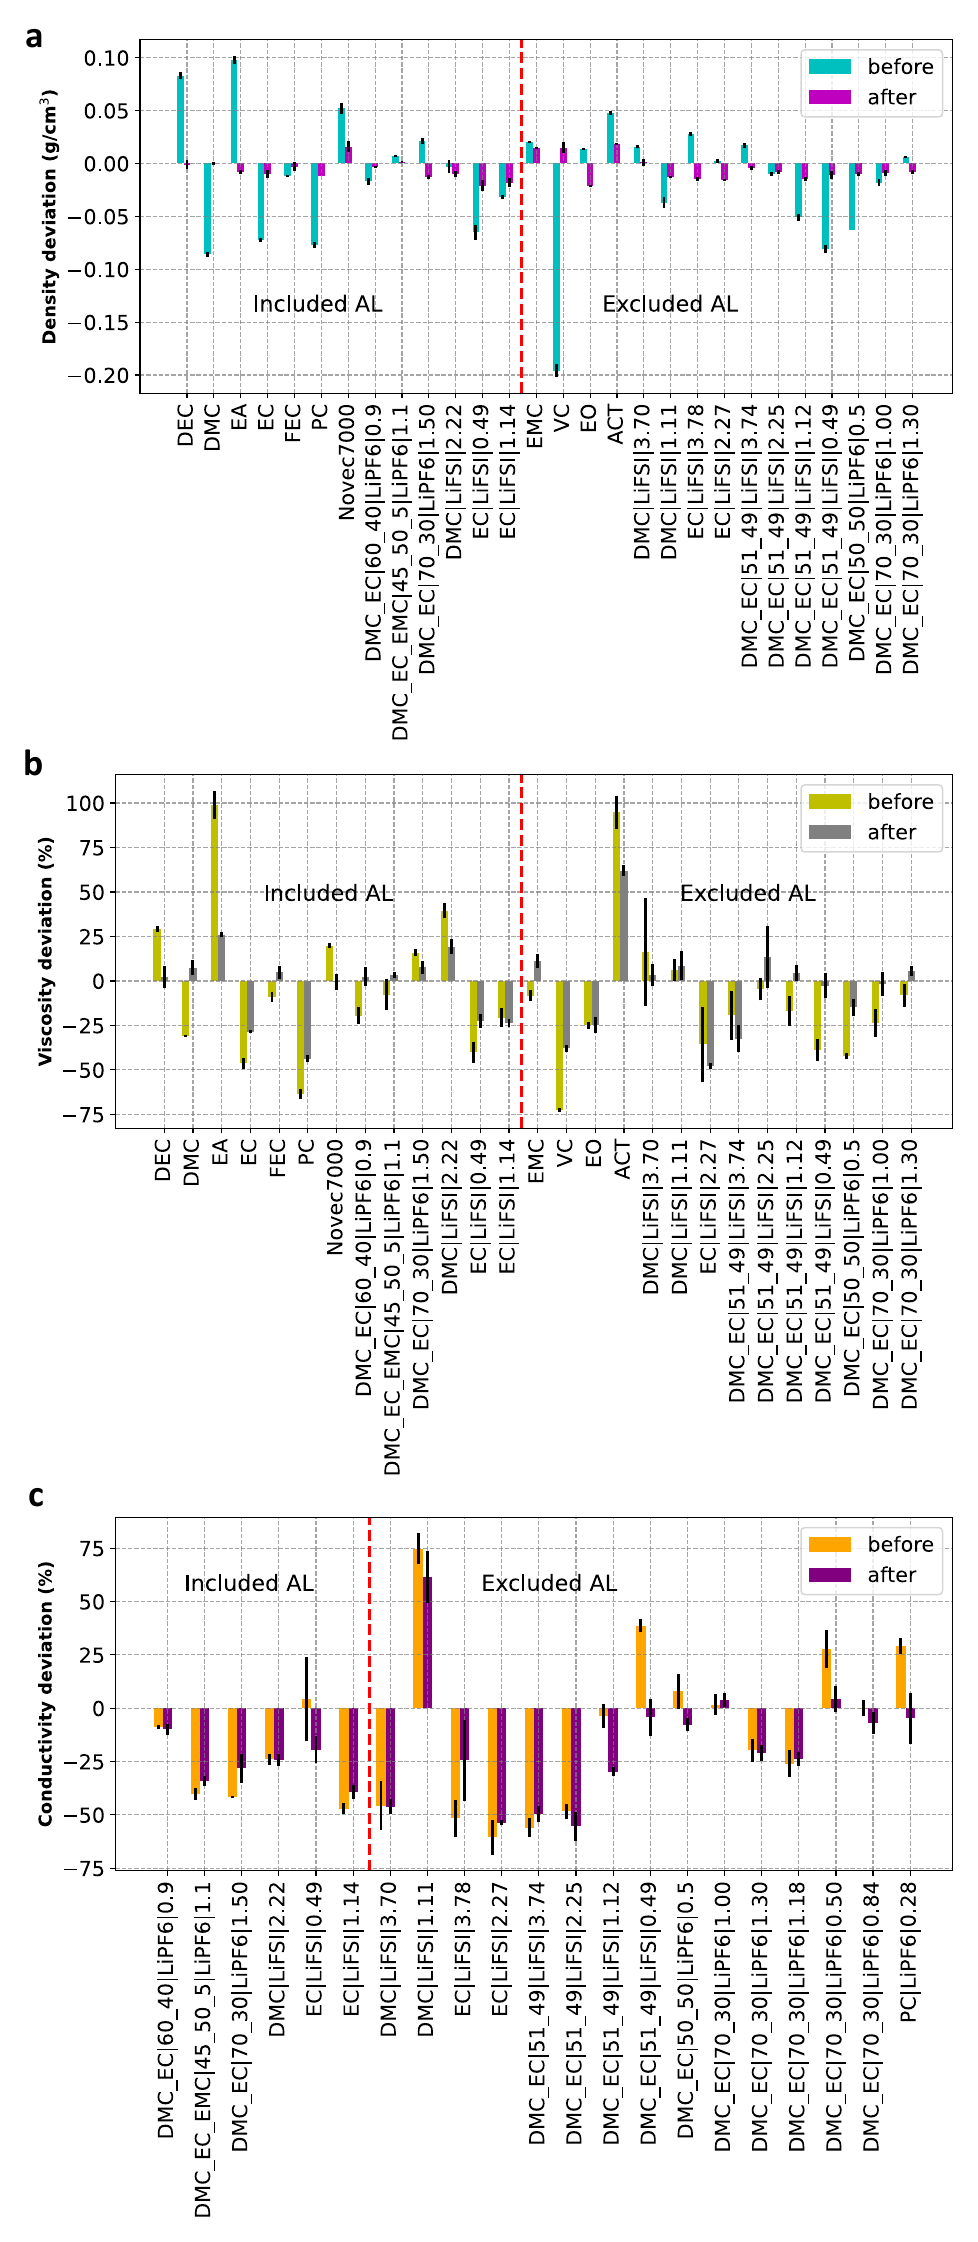}
    \caption{\textbf{\textbf{a}} to \textbf{\textbf{c}} Density, viscosity, and conductivity of molecular liquid and solutions before and after density alignment, respectively.}
    \label{fig:impact_of_alignment}
\end{figure}

Figures \ref{fig:impact_of_alignment} and \ref{Figure 2} highlight the significant impact of density alignment on the physical properties of density, viscosity, and conductivity. The alignment process notably reduces the density error from 0.05 g/cm$^3$ to approximately 0.01 g/cm$^3$ for both the systems included in the alignment and those not directly aligned. This improvement suggests that density alignment, which adjusts the strength of inter-molecular interactions, has a degree of transferability to molecules with similar structures or solutions with varying salt concentrations not explicitly included in the alignment.
For example, before alignment, cyclic carbonates like EC, FEC, and PC exhibit densities lower than experimental values. The alignment process increases inter-molecular interaction strength, thereby raising the predicted densities. Consequently, VC, another cyclic carbonate not included in the alignment, also shows an improved density prediction due to enhanced inter-molecular interactions among cyclic carbonates.

The effect of density alignment extends to solutions with EC and DMC as solvents and varying amounts of LiFSI salt. Prior to alignment, the MLFF tends to underestimate the densities of pure EC and DMC solvents. For aligned solutions at different molalities (0.49, 1.14, and 2.22 mol/kg), a pattern emerges: higher molality correlates with a lesser extent of density underestimation. This indicates that, initially, the MLFF underestimates solvent-solvent interactions while overestimating solvent-ion and/or ion-ion interactions. Through density alignment, these interactions are recalibrated—strengthening solvent-solvent and weakening solvent-ion/ion-ion interactions—leading to more accurate density predictions. Thus, for solutions with even higher molalities (3.70, 3.74, and 3.78 mol/kg) not included in the alignment, where the pre-alignment MLFF overestimated densities, the post-alignment MLFF, with adjusted interaction strengths, offers more accurate density predictions with smaller degree of (or even no) overestimation.

\begin{figure}
    \centering
    \includegraphics[width=\textwidth]{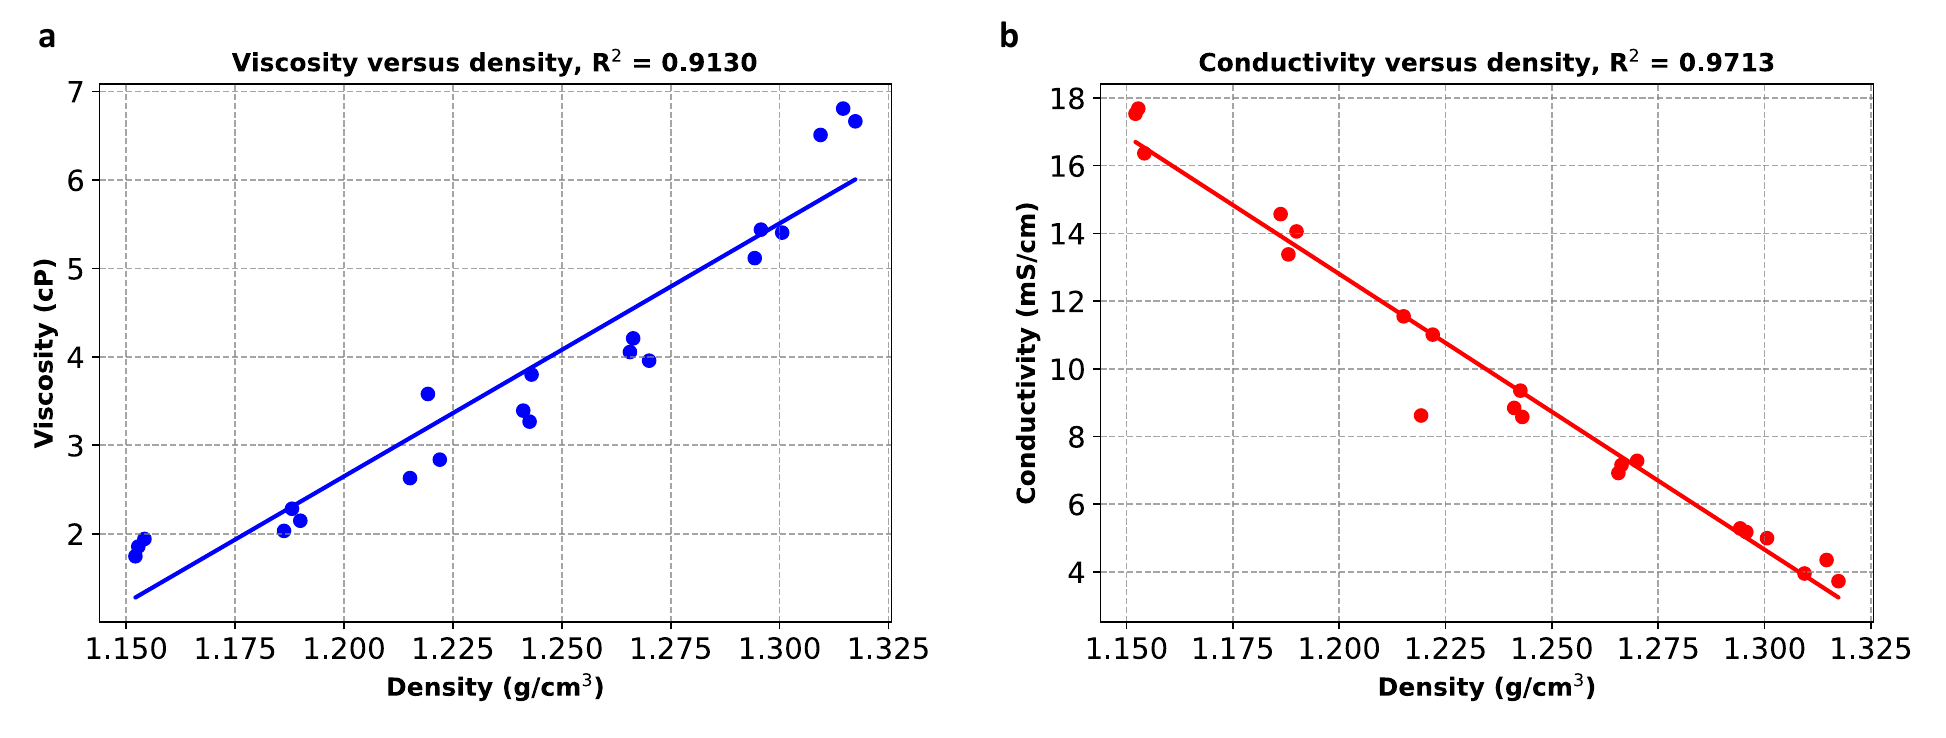}
    \caption{\textbf{\textbf{a}} and \textbf{\textbf{b}} Density versus viscosity, and density versus conductivity for the system of DMC$\_$EC$|$70$\_$30$|$LiPF6$|$1.0, respectively. The models leading to different densities are from the first round of density alignment.}
    \label{fig:density_versus_vis_cond}
\end{figure}

In Figure \ref{fig:density_versus_vis_cond}, the observed strong dependence of viscosity and ionic conductivity on density aligns with expectations: a denser liquid typically exhibits stronger inter-molecular interactions, resulting in higher viscosity and lower conductivity. Thus, a post-alignment increase in density generally leads to a corresponding increase in viscosity and a decrease in conductivity. Figure \ref{fig:impact_of_alignment}b and c confirm this relationship for most liquids post-alignment.
From Figure \ref{fig:impact_of_alignment}b and Figure \ref{Figure 2}g, it's evident that the discrepancy in viscosity between MLFF MD simulations and experimental observations narrows significantly—from a 32\% to a 17\% deviation post-alignment. This improvement in viscosity accuracy is also seen in liquids not in the alignment, indicating the transferability of the alignment's effects.

However, the situation is more complex with ionic conductivity. In certain cases, aligning MD density to experimental data inadvertently moves the ionic conductivity further from the experimental values. For instance, the systems EC$|$LiFSI$|$0.49 and DMC\_EC$|$0.51\_0.49$|$LiFSI$|$1.12 show underestimations in density and viscosity but have conductivities close to experimental values before alignment. Post-alignment, while their densities and viscosities adjust closer to experimental figures, their conductivities decrease, diverging from the experimental data. Consequently, the overall deviation in ionic conductivity decreases only modestly from 31\% to 26\% after density alignment. This suggests that while density alignment effectively narrows the gap in density and viscosity predictions, a more targeted alignment strategy might be needed to align ionic conductivity predictions more closely with experimental results. In Section~\ref{si:simpe_system}, we provide more in-depth analysis about the predictions of individual systems of interest.

In Wang $et$ $al.$~\cite{dmff}, the gradient $\partial O / \partial \theta$, where $O$ denotes a observable from MD simulations and $\theta$ parameters of force field, is computed by the differentiable MD platform (DMFF) to optimize the observable from MD simulations. In this sense, both DMFF and the density alignment algorithm in this work can be used to finetune the force field by experimentally measured observables. However, to the best of the authors' knowledge, DMFF has been mostly used to optimize classic force fields and less applied to train deep learning-based MLFF. There are two possible reasons for this phenomenon. The first is that, DMFF requires multiple sequential MD simulations by the force fields to iteratively align the force field and the experimentally measured observables. For example, in Wang $et$ $al.$\cite{dmff}, 40 to 60 sequential loops of MD simulations are conducted to align the radial distribution function (RDF) of one system. Since the inference speed of MLFF is still limited, DMFF and similar optimization methods are very expansive and time-consuming to optimize MLFF in practice. Instead, in the density alignment algorithm, for each system only one round of parallel MD simulations (7 in this work) are conducted to compute the required change of pressure to align the MLFF and the experiment, which makes the optimization more affordable in terms of computational cost. The other possible reason is that, experimental datasets typically contain limited number of data points, which might make the MLFF overfit to the training data by the purely data-driven gradient-based optimization~\cite{expfusion}. Since the density alignment algorithm is based on the compressibility of liquids and only optimizes inter-molecular interactions, the alignment demonstrates considerable transferability to liquids not initially included in the alignment process.
