# Supplementary material for: A predictive machine learning force field framework for liquid electrolyte development
Source: arXiv:2404.07181 source file (2025-04-01)
Supplement: Supplementary file 3 [file comparison.tex]

\section{Comparison with Other Force Fields}
\label{si:comparison}

In this section, we compare the performance between BAMBOO and APPLE\&P~\cite{borodinapplep}, QRNN~\cite{qrnnliquidelectrolyte}, and OPLS-AA~\cite{oplsaa, liparameter, anionparameter} as in Table~\ref{tab:applepbenchmark},~\ref{tab:qrnnbenchmark}, and~\ref{tab:oplsaabenchmark}. Here, the properties from APPLE\&P and QRNN are collected from the corresponding references listed in the tables, and those from OPLS-AA are computed by ourselves. For OPLS-AA, the force field parameters for solvent molecules are taken from Ref.~\cite{oplsaa}, that for Li from Ref.~\cite{liparameter}, and that for anions from Ref.~\cite{anionparameter}. Here, the system size of OPLS-AA-based MD simulation increases from 4,000 atoms (the size for BAMBOO MLFF) to 10,000 atoms, and all other settings for the OPLS-AA simulations are the same as that for BAMBOO-based simulations. 

From Table~\ref{tab:applepbenchmark}, we can see that, for both density of pure EC, DMC, PC, and conductivities of liquid electrolytes with DMC and EC as solvents and LiPF$_{6}$ or LiTFSI as salts, BAMBOO predicts more closely to the experimental values than APPLE\&P. We can also see that, for systems in Table~\ref{tab:oplsaabenchmark} and~\ref{tab:zhushang} which are included in the DFT dataset, BAMBOO achieves lower prediction error for density (MAE 0.011 g/cm$^3$), viscosity (mean deviation 17.3\%), and conductivity (mean deviation 24.2\%) than OPLS-AA (0.020 g/cm$^3$, 140.4\%, and 54.9\% for density, viscosity, and conductivity error, respectively). The two observations show the superior ability of BAMBOO on simulating bulk properties of organic liquids and electrolytes compared with classic force fields with and without polarizable terms. In Table~\ref{tab:qrnnbenchmark}, we compare density and viscosity from BAMBOO and QRNN, from which we can see that BAMBOO outperforms QRNN in terms of density and viscosity prediction, which demonstrates the state-of-the-art performance of BAMBOO among existing machine learning force fields.

\begin{table}[hbt!]
\caption{The simulated density ($\rho$, in g/cm$^{3}$), and ionic conductivity ($\sigma$, in mS/cm) of solvents and liquid electrolytes from APPLP\&P~\cite{borodinapplep} and BAMBOO. For conductivities reported in referred literature that have multiple records from different post-processing methods, the value closest to the experimental is shown here. The uncertainty for the density calculated using BAMBOO ranges from 0.001 to 0.005 g/cm$^{3}$. The uncertainty for the conductivities calculated using BAMBOO ranges from 0.089 to 0.425 mS/cm. Except the last row where the temperature is specified as 333 K, all other BAMBOO simulations are conducted at 298 K. For clarity, we do not show simulated properties which do not have corresponding experimental/simulated values to compare.}
\label{tab:applepbenchmark}
\vskip 0.15in
\begin{center}
\begin{tabular}{lccccccr}
\toprule
\small

Compositions&$\rho_{\text{APPLP\&P}}$&$\rho_{\text{BAMBOO}}$&$\rho_{\text{Exp}}$&$\sigma_{\text{APPLP\&P}}$&$\sigma_{\text{BAMBOO}}$&$\sigma_{\text{Exp}}$\\

\midrule
DMC& 1.040~\cite{borodinapplep} & 1.060 & 1.057~\cite{borodinapplep} & NA & NA & NA \\
EC & 1.302~\cite{borodinapplep} & 1.310 & 1.321~\cite{borodinapplep} & NA & NA & NA \\
PC & 1.209~\cite{borodinapplep} & 1.188 & 1.194~\cite{borodinapplep} & NA & NA & NA \\
%EC$|$LiPF$_{6}$$|$0.87 & NA & 1.382 & NA & 8.5 & 5.811 & 6.8 \\
DMC\_EC$|$51\_49$|$LiPF$_{6}|$0.86 & NA & NA & NA & 13.5~\cite{oldiges2018understanding} & 11.740 & 12~\cite{oldiges2018understanding} \\
DMC\_EC$|$51\_49$|$LiTFSI$|$0.86 & NA & NA & NA & 12~\cite{oldiges2018understanding} & 6.359 & 9~\cite{oldiges2018understanding} \\
DMC\_EC$|$51\_49$|$LiPF$_{6}|$1.12 & NA & NA & NA & 15.9~\cite{applepliquidelectrolyte} & 10.269 & 11.7~\cite{berhaut2019ionic} \\
DMC\_EC$|$51\_49$|$LiPF$_{6}|$1.12$|$333K & NA & NA & NA & 25.9~\cite{applepliquidelectrolyte} & 20.490 & 19.5~\cite{berhaut2019ionic} \\
\bottomrule

\end{tabular}
\end{center}
\vskip -0.1in
\end{table}

\begin{table}[hbt!]
\caption{The simulated density ($\rho$, in g/cm$^{3}$), and viscosity ($\eta$, in cP) of solvents and liquid electrolytes from QRNN~\cite{qrnnliquidelectrolyte} and BAMBOO. The uncertainty for the density calculated using BAMBOO ranges from 0.001 to 0.005 g/cm$^{3}$. The uncertainty for the viscosity calculated using BAMBOO ranges from 0.018 to 0.275 cP, while that from QRNN ranges from 0.05 to 3.77 cP. The BAMBOO simulations for pure solvents are conducted at 298 K, and that for DMC, EC, LiPF$_{6}$ mixtures are conducted at 313 K. For clarity, we do not show simulated properties which do not have corresponding experimental/simulated values to compare.}
\label{tab:qrnnbenchmark}
\vskip 0.15in
\begin{center}
\begin{tabular}{lccccccr}
\toprule
\small

Compositions&$\rho_{\text{QRNN}}$&$\rho_{\text{BAMBOO}}$&$\rho_{\text{Exp}}$&$\eta_{\text{QRNN}}$&$\eta_{\text{BAMBOO}}$&$\eta_{\text{Exp}}$\\

\midrule
DMC& 1.07~\cite{qrnnliquidelectrolyte} & 1.060 & 1.057~\cite{borodinapplep} & 0.79~\cite{qrnnliquidelectrolyte} & 0.629 & 0.585, 0.706 \cite{xu2004nonaqueous,sasaki2005physical} \\
EC & 1.35~\cite{qrnnliquidelectrolyte} & 1.310 & 1.321~\cite{borodinapplep} & 2.27~\cite{qrnnliquidelectrolyte} & 1.381 & 1.60-1.90 \cite{xu2004nonaqueous, hagiyama2008physical,sasaki2005physical} \\
PC & 1.22~\cite{qrnnliquidelectrolyte} & 1.188 & 1.194~\cite{borodinapplep} & 2.6~\cite{qrnnliquidelectrolyte} & 1.426 & 2.53~\cite{xu2004nonaqueous} \\
EMC & 0.99~\cite{qrnnliquidelectrolyte} & 1.015 & 1.0~\cite{xu2004nonaqueous} & 0.65~\cite{qrnnliquidelectrolyte} & 0.724 & 0.65~\cite{xu2004nonaqueous} \\
DEC & 0.92~\cite{qrnnliquidelectrolyte} & 0.969 & 0.97~\cite{xu2004nonaqueous} & 0.43~\cite{qrnnliquidelectrolyte} & 0.766 & 0.749~\cite{xu2004nonaqueous} \\
VC & 1.31~\cite{qrnnliquidelectrolyte} & 1.370 & 1.355~\cite{xu2004nonaqueous} & 1.26~\cite{qrnnliquidelectrolyte} & 1.104 & 1.5, 1.78~\cite{qrnnliquidelectrolyte, VC_visco} \\
FEC & 1.47~\cite{qrnnliquidelectrolyte} & 1.474 & 1.477~\cite{hagiyama2008physical} & 3.02~\cite{qrnnliquidelectrolyte} & 2.349 & 2.24-4.1~\cite{hagiyama2008physical, janes2014fluoroethylen, sasaki2005physical} \\
%EC$|$LiPF$_{6}$$|$0.87 & NA & 1.382 & NA & 8.5 & 5.811 & 6.8 \\
DMC\_EC$|$70\_30 & NA & NA & NA & 0.83~\cite{qrnnliquidelectrolyte} & 0.756 & 0.73~\cite{logan2018study} \\
DMC\_EC$|$70\_30$|$LiPF$_{6}|$0.51 & NA & NA & NA & 1.65~\cite{qrnnliquidelectrolyte} & 1.448 & 1.18~\cite{logan2018study} \\
DMC\_EC$|$70\_30$|$LiPF$_{6}|$1.02 & NA & NA & NA & 2.02~\cite{qrnnliquidelectrolyte} & 2.398 & 1.92~\cite{logan2018study} \\
DMC\_EC$|$70\_30$|$LiPF$_{6}|$1.63 & NA & NA & NA & 6.98~\cite{qrnnliquidelectrolyte} & 4.328 & 3.21~\cite{logan2018study} \\
DMC\_EC$|$70\_30$|$LiPF$_{6}|$2.14 & NA & NA & NA & 22.38~\cite{qrnnliquidelectrolyte} & 6.351 & 5.1~\cite{logan2018study} \\
\bottomrule

\end{tabular}
\end{center}
\vskip -0.1in
\end{table}

\begin{table}[hbt!]
\caption{The simulated density ($\rho$, in g/cm$^{3}$), viscosity ($\eta$, in cP), and ionic conductivity ($\sigma$, in mS/cm) of solvents and liquid electrolytes from OPLS-AA~\cite{oplsaa, liparameter, anionparameter}. For simplicity, systems shown in Table~\ref{tab:zhushang},~\ref{tab:highentropy},~\ref{tab:newmolecules} are not repeated here, and the experimental values shown in Tables listing BAMBOO predictions in section~\ref{si:others} are not repeated here. The uncertainty for the density calculated using OPLS-AA ranges from 0.001 to 0.004 g/cm$^{3}$, that of viscosity from 0.002 to 9.972 cP, and that of conductivity from 0.037 to 0.736 mS/cm. For clarity, we do not show simulated properties which do not have corresponding experimental values to compare. All simulations are conducted at 298K unless specified.}
\label{tab:oplsaabenchmark}
\vskip 0.15in
\begin{center}
\begin{tabular}{lcccr}
\toprule
\small

Compositions&$\rho_{\text{OPLS-AA}}$&$\eta_{\text{OPLS-AA}}$&$\sigma_{\text{OPLS-AA}}$ \\

\midrule
DEC & 0.995 & 1.146 & NA \\
DMC & 1.081 & 0.892 & NA \\
EA & 0.924 & 0.709 & NA \\
EC & 1.273 & 1.073 & NA \\
FEC & 1.458 & 1.264 & NA \\
PC & 1.194 & 1.426 & NA \\
Novec7000 & 1.492 & 0.449 & NA \\
DMC\_EC$|$60\_40$|$LiPF$_{6}|$0.9 & 1.250 & 6.534 & 5.808 \\
DMC\_EC\_EMC$|$45\_50\_5$|$LiPF$_{6}|$1.1 & 1.283 & 9.266 & 4.703 \\
DMC\_EC$|$70\_30$|$LiPF6$|$1.5 & 1.283 & 15.899 & 3.294 \\
DMC$|$LiFSI$|$2.22 & 1.285 & 21.700 & 2.498 \\
EC$|$LiFSI$|$0.49 & 1.334 & 4.241 & 4.328 \\
EC$|$LiFSI$|$1.14 & 1.389 & 10.689 & 2.971 \\
EMC & 1.031 & 0.999 & NA \\
VC & 1.340 & 0.704 & NA \\
EO & 0.773 & 0.513 & NA \\
ACT & 0.788 & 0.375 & NA \\
EP & 0.898 & 0.699 & NA \\
DMC$|$LiFSI$|$3.70 & 1.382 & 138.552 & 0.489 \\
DMC$|$LiFSI$|$1.11 & 1.190 & 5.645 & 5.047 \\
EC$|$LiFSI$|$3.78 & 1.557 & 136.279 & 0.538 \\
EC$|$LiFSI$|$2.27 & 1.472 & 34.459 & 1.458 \\
DMC\_EC$|$51\_49$|$LiFSI$|$3.74 & 1.465 & 211.159 & 0.369 \\
DMC\_EC$|$51\_49$|$LiFSI$|$2.25 & 1.374 & 33.181 & 1.529 \\
DMC\_EC$|$51\_49$|$LiFSI$|$1.12 & 1.287 & 7.56 & 4.474 \\
DMC\_EC$|$51\_49$|$LiFSI$|$0.49 & 1.229 & 3.291 & 5.487 \\
DMC\_EC$|$50\_50$|$LiPF$_{6}|$0.5 & 1.231 & 3.851 & 5.621 \\
DMC\_EC$|$70\_30$|$LiPF$_{6}|$1.0 & 1.239 & 7.051 & 5.371 \\
DMC\_EC$|$70\_30$|$LiPF$_{6}|$1.3 & 1.267 & 11.429 & 4.018 \\
DMC\_EC$|$70\_30$|$LiPF$_{6}|$0.5 & NA & NA & 5.921 \\
DMC\_EC$|$70\_30$|$LiPF$_{6}|$0.84 & NA & NA & 7.887 \\
PC$|$LiPF$_{6}$$|$0.28 & NA & NA & 3.345 \\
EC$|$LiPF$_{6}$$|$0.87 & NA & NA & 5.606 \\
DMC\_EC$|$51\_49$|$LiPF$_{6}|$0.86 & NA & NA & 6.236 \\
DMC\_EC$|$51\_49$|$LiTFSI$|$0.86 & NA & NA & 5.133 \\
DMC\_EC$|$51\_49$|$LiPF$_{6}|$1.12 & NA & NA & 6.236 \\
DMC\_EC$|$51\_49$|$LiPF$_{6}|$1.12$|$333K & NA & NA & 14.455 \\
DMC\_EC$|$70\_30$|$313K & NA & 1.23~\cite{qrnnliquidelectrolyte} & NA \\
DMC\_EC$|$70\_30$|$LiPF$_{6}|$0.51$|$313K & NA & 2.15~\cite{qrnnliquidelectrolyte} & NA \\
DMC\_EC$|$70\_30$|$LiPF$_{6}|$1.02$|$313K & NA & 3.62~\cite{qrnnliquidelectrolyte} & NA \\
DMC\_EC$|$70\_30$|$LiPF$_{6}|$1.63$|$313K & NA & 7.80~\cite{qrnnliquidelectrolyte} & NA \\
DMC\_EC$|$70\_30$|$LiPF$_{6}|$2.14$|$313K & NA & 15.26~\cite{qrnnliquidelectrolyte} & NA \\
\bottomrule

\end{tabular}
\end{center}
\vskip -0.1in
\end{table}
