# Supplementary material for: A predictive machine learning force field framework for liquid electrolyte development
Source: arXiv:2404.07181 source file (2025-04-01)
Supplement: Supplementary file 4 [file dft.tex]

\subsection{DFT Dataset Construction}
\label{si:dft}
In this work, we use 720,000 clusters with the DFT calculated energy, atomic forces, virial tensor, dipole moment, and partial charge (CHELPG) to train BAMBOO. The calculations are performed utilizing the B3LYP~\cite{b3lyp} functional alongside the def2-svpd~\cite{svpd} basis set, supplemented by density fitting techniques based on the def2-universal-jkfit auxiliary basis~\cite{weigend2008hartree}. Throughout the computational process, the convergence threshold for the self-consistent field is set to $1.0\times10^{-10}$ a.u., with a maximum allowance of 100 iterations. Here, we use the open-source GPU4PySCF package~\cite{GPU4PySCFGITHUB, gpu4pyscf} developed by ByteDance Inc. for the DFT calculations. Compared with QChem~\cite{qchem} on 32 CPUs, GPU4PySCF on a single V100 GPU can reduce cost by 97\% in terms of computation time and 95\% in terms of cost. 

The procedure of collecting cluster structures is described below: first we take clusters in Ref.~\cite{qrnnliquidelectrolyte} as the starting point, which contains species including EC, PC, VC, FEC, DMC, EMC, DEC, PF$_{6}^{-}$, and Li$^{+}$. Then, we train five BAMBOO models by the DFT labels of the initial cluster structures calculated by GPU4PySCF, and run MD simulations using one randomly picked model at 300K for 1 ns with the NPT ensemble on pure solvents of EA, EP, EO, ACT, and Novec7000, and solutions with EC:DMC:EMC:PC:LiPF$_{6}$ = 3:3:1:1:1, EC:DMC:EMC:VC:LiFSI = 3:3:1:1:1, and EC:DMC:LiFSI:LiTFSI = 10:10:1:1 by moles. In the first round of MD simulations, we observe that spurious reactions (mainly bond breaking) would occur in most simulations with new molecules and anions, which is expected as the initial structures do not cover the chemistry of the new species, especially FSI$^{-}$ and TFSI$^{-}$. Then, we sample clusters from the MD trajectories until the first spurious reaction happens, and we use the following active learning scheme to sample clusters from the MD trajectories.
\begin{enumerate}
\item Instead of focusing on the uncertainty of the energy of the cluster as discussed in Ref.~\cite{qrnnliquidelectrolyte}, our attention shifts to the uncertainty of predictions concerning atomic properties $\Vec{f}_{i}$ and $q_{i}$. First, we employ five models to compute the standard deviation of predictions of charge $\sigma_{q}$ and magnitude of force $\sigma_{||\Vec{f}||}$ on each atom. We then select all atoms for which $\sigma_{q} > 0.015$ a.u. and $\sigma_{||\Vec{f}||} > 3$ kcal/(mol$\cdot$\AA). For hydrogen atoms, we lower the criteria to $\sigma_{q} > 0.01$ a.u. and $\sigma_{||\Vec{f}||} > 2$ kcal/(mol$\cdot$\AA) as hydrogen is significantly lighter than other elements and typically exhibits smaller magnitudes of $q$ and $\Vec{f}$.
\item When encountering uncertain atoms (expect Li$^{+}$), we first determine the molecule/anion to which the uncertain atom belongs, and consider the molecule/anion as a cluster.
\item Next, we search for molecules, anions, and cations that have at least one atom within a 5 \AA~radius of the uncertain atom. This search includes the molecule/anion to which the uncertain atom belongs. We consider all the neighboring molecules/anions/cations found in this search as a cluster. It's worth noting that if multiple atoms within a single molecule are identified as uncertain, we perform the search for neighboring molecules only once to minimize redundancy.
\item We input clusters containing no more than 110 atoms into GPU4PySCF for labelling, and incorporate the newly labeled clusters and DFT labels into the dataset for training.
\item We repeat steps 1-4 iteratively. Once a system demonstrates stability without spurious reactions during the 1 ns MD simulation, we terminate the procedure for that particular system.
\end{enumerate}

We achieve stable MD simulations for all the pure solvents within two iterations, and for solutions within three iterations. In Figure \ref{dataset}, we present the distribution of number of atoms in clusters and the number of molecules in the datasets. We observe two peaks in cluster sizes: one with fewer atoms corresponding to single molecules/anions, and another with more atoms representing the complete cluster within 5 \AA~of the central uncertain atoms. Regarding the distribution of molecules, EC, Novec7000, VC, and DMC are the four most frequently sampled molecules. Among these, EC and DMC are the two main solvents of interest in this study, while VC and Novec7000 possess unique structural features compared with other molecules (such as a carbon-carbon double bond in VC and a high ratio of fluorination in Novec7000).

After each iteration of data collection, we randomly choose 90\% data as the training set, and 10\% as the validation set to evaluate the performance of the training process. Therefore, the validation set has the same distribution as the training set where there are considerable number of high energy structures such as distorted molecules, decomposed molecules, and even clusters with only Li. Although these off-equilibrium structures are necessary to stabilize the MD simulations driven by the MLFFs, such high energy states might boost the prediction RMSE. Since Figure~\ref{dft_parity}a to f are all based on the validation set, the RMSE values reported at those figures can be further lowered if we only consider near-equilibrium structures that would appear in production MD simulations. Similar to Dajnowicz $et$ $al.$~\cite{qrnnliquidelectrolyte} where the test set is separately sampled from production MD simulations, we construct a separate test set sampling 10,000 clusters from production MD simulations, and we use the MLFF used for production (the one after density alignment) to predict the energy, force, and virial of the test set. As in Figure~\ref{dft_parity}g, h and i, we can see that the RMSE of energy, force, and virial predictions on the test set decrease 78\%, 41\%, and 49\% compared with the validation set, which more closely reflect the degree of prediction errors in the production MD simulations.

\begin{figure}
    \centering
    \includegraphics[width=\textwidth]{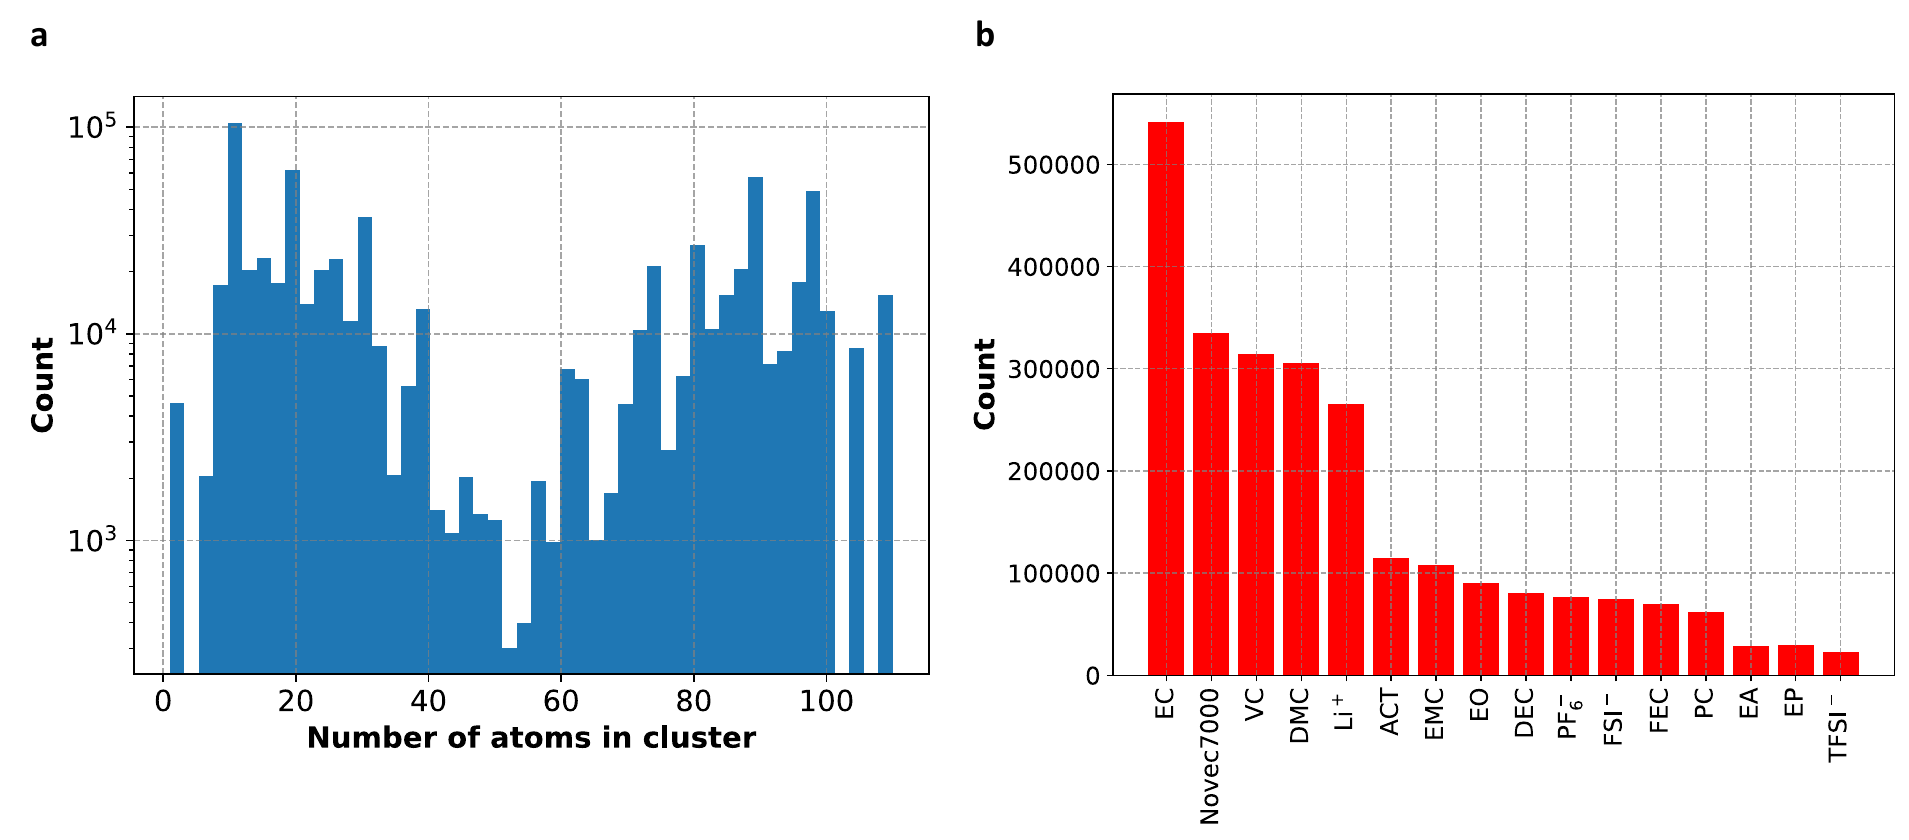}
    \caption{\textbf{\textbf{a}} and \textbf{\textbf{b}} Count of number of atoms in a cluster and number of molecules/ions in the dataset, respectively.}
    \label{dataset}
\end{figure}
