# Supplementary material for: A predictive machine learning force field framework for liquid electrolyte development
Source: arXiv:2404.07181 source file (2025-04-01)
Supplement: Supplementary file 5 [file electrolyte.tex]

\section{Liquid Electrolyte Data}
\label{si:others}
In this section, we show all the simulated and experimental properties of solvents and solutions for readers' reference.

\begin{table}[hbt!]
\caption{The simulated densities in g/cm$^3$ of pure solvents and mixtures that are used in the density alignment process. The salt concentrations (``m'') of mixtures are in molality, defined as the mole of salt in kilograms of solvent. The compositions of the LiFSI-containing mixtures are converted based on their molar ratios as used in the original literature. The electrolytes are presented in ``solvents$|$solvent weight $\%$$|$salt$|$salt molality'' format. The uncertainty associated with the density prediction ranges from 0.001-0.003 g/cm$^3$. All simulations are performed at 298K, except for EC and FEC, which were conducted at 313K.}

\label{tab:den_finetune}
\vskip 0.15in
\begin{center}
\begin{tabular}{lccccr}
\toprule
Mixtures & Compositions & BAMBOO  & Exp & Exp. Ref. \\

\midrule
DMC & DMC 100 wt\% & 1.060 & 1.06 & \cite{xu2004nonaqueous} \\
DEC & DEC 100 wt\% & 0.969 & 0.97 & \cite{xu2004nonaqueous} \\
PC & PC 100 wt\% & 1.188 & 1.20, 1.194 & \cite{vali2016vinylene, borodinapplep} \\
EC & EC 100 wt\% & 1.310 & 1.32 &  \cite{xu2004nonaqueous} \\
FEC & FEC 100 wt\% & 1.474 & 1.48 & \cite{hagiyama2008physical} \\
EA & EA 100 wt\% & 0.892 & 0.90 & \cite{guard1999chemical} \\
Novec7000 & Novec7000 100 wt\% & 1.416 & 1.41 & \cite{novec7000} \\
P5 & DMC\_EC$|$60\_40$|$LiPF$_{6}|$0.9
 & 1.236 & 1.239 & Acquired from \cite{dave2022autonomous} \\
P6 & DMC\_EC\_EMC$|$45\_50\_5$|$LiPF$_{6}|$1.1
& 1.274 & 1.273 & Acquired from \cite{dave2022autonomous} \\
P7 & DMC\_EC$|$70\_30$|$LiPF$_{6}|$1.5 & 1.255 & 1.268 & Acquired from \cite{dave2022autonomous} \\
F4 & DMC$|$LiFSI$|$2.22
& 1.260 & 1.27 &DMC:LiFSI 5:1\cite{wang2016superconcentrated} \\
F5 & EC$|$LiFSI$|$0.49
 & 1.359 & 1.38 & EC:LiFSI 23:1 \cite{wang2016superconcentrated} \\
F6 & EC$|$LiFSI$|$1.14
& 1.412 & 1.43 & EC:LiFSI 10:1 \cite{wang2016superconcentrated} \\
\bottomrule
\end{tabular}
\end{center}
\vskip -0.1in
\end{table}

\begin{table}[hbt!]
\caption{The simulated densities in g/cm$^3$ of pure solvents and mixtures that are \textbf{not} used in the density alignment process. The salt concentrations (``m") of mixtures are in molality, defined as the mole of salt in kilograms of solvent. The compositions of the LiFSI-containing mixtures are converted based on their molar ratios as used in the original literature. The electrolytes are presented in ``solvents$|$solvent weight $\%$$|$salt$|$salt molality'' format. The uncertainty associated with the density prediction ranges from 0.001-0.003 g/cm$^3$. The simulations are conducted at 298K.}
\label{tab:den_no_finetune}
\vskip 0.15in
\begin{center}
\begin{tabular}{lccccr}
\toprule
 Mixtures & Compositions & BAMBOO  & Exp & Exp. Ref. \\

\midrule
EMC & EMC 100 wt\% & 1.015 & 1.0 & \cite{xu2004nonaqueous} \\
VC & VC 100 wt \% & 1.370 & 1.355 &\cite{xu2004nonaqueous} \\
EO & EO 100 wt \% & 0.769 & 0.79 &~\cite{crchandbook} \\
ACT & ACT 100 wt \% & 0.808 & 0.79 &~\cite{crchandbook} \\
EP & EP 100 wt \% & 0.919 & 0.884 &~\cite{EP} \\
S1 & DMC\_EC$|$70\_30& 1.131 & 1.13 & SI of \cite{dave2022autonomous} \\
S2 & DMC\_EC$|$50\_50 & 1.183 & 1.18 & SI of \cite{dave2022autonomous} \\
S3 & EMC\_EC$|$70\_30 & 1.100 & 1.095 & SI of \cite{dave2022autonomous} \\
S4 & EMC\_EC$|$50\_50 & 1.160 & 1.156 & SI of \cite{dave2022autonomous} \\
P1 & DMC\_EC$|$50\_50$|$LiPF$_{6}|$0.5 & 1.224 & 1.235 & Acquired from \cite{dave2022autonomous} \\
P4 & DMC\_EC$|$70\_30$|$LiPF$_{6}|$1.0  & 1.221 & 1.228 & Acquired from \cite{dave2022autonomous} \\
P8 & DMC\_EC$|$70\_30$|$LiPF$_{6}|$1.3 & 1.243 & 1.252 & Acquired from \cite{dave2022autonomous} \\

F7 & DMC$|$LiFSI$|$3.70
 & 1.361 & 1.36 & DMC:LiFSI 3:1 \cite{wang2016superconcentrated} \\
F8 & DMC$|$LiFSI$|$1.11
 & 1.167 & 1.18 & DMC:LiFSI 10:1 \cite{wang2016superconcentrated} \\

F9 & EC$|$LiFSI$|$3.78
 & 1.555 & 1.57 & EC:LiFSI 3:1 \cite{wang2016superconcentrated} \\
F10 & EC$|$LiFSI$|$2.27
 & 1.484 & 1.50  & EC:LiFSI 5:1 \cite{wang2016superconcentrated} \\

F3 & DMC\_EC$|$51\_49$|$LiFSI$|$3.74
 & 1.456 & 1.46 &DMC:EC:LiFSI 3:3:2 \cite{wang2016superconcentrated} \\
F2 & DMC\_EC$|$51\_49$|$LiFSI$|$2.25
 & 1.372 & 1.38 & DMC:EC:LiFSI 5:5:2 \cite{wang2016superconcentrated} \\
F1 & DMC\_EC$|$51\_49$|$LiFSI$|$1.12
 & 1.285 & 1.30 & DMC:EC:LiFSI 10:10:2 \cite{wang2016superconcentrated} \\
F11 & DMC\_EC$|$51\_49$|$LiFSI$|$0.49
 & 1.229 & 1.24 &DMC:EC:LiFSI 23:23:2 \cite{wang2016superconcentrated} \\

\bottomrule
\end{tabular}
\end{center}
\vskip -0.1in
\end{table}

\begin{table}[hbt!]
\caption{The simulated viscosities in cP of solvents}
\label{tab:visco_solv}
\vskip 0.15in
\begin{center}
\begin{tabular}{lccccr}
\toprule
Mixtures & Compositions & Temperature, K & BAMBOO  & Exp \\

\midrule
DMC & DMC 100 wt\% & 298 & 0.629$\pm$0.0290 & 0.585, 0.706 \cite{xu2004nonaqueous,sasaki2005physical} \\
DEC & DEC 100 wt\% & 298 & 0.766$\pm$0.0243 & 0.75 \cite{xu2004nonaqueous} \\
EMC & EMC 100 wt\% & 298 & 0.724$\pm$0.0204 & 0.65 \cite{xu2004nonaqueous} \\
VC & VC 100 wt\% & 298 & 1.104$\pm$0.0540 & 1.78 \cite{VC_visco} \\
EC & EC 100 wt\% & 313 & 1.381$\pm$0.0386 & 1.60-1.90 \cite{xu2004nonaqueous, hagiyama2008physical,sasaki2005physical} \\
FEC & FEC 100 wt\% & 313 & 2.349$\pm$0.0941 & 2.24-4.1~\cite{hagiyama2008physical, janes2014fluoroethylen, sasaki2005physical} \\
Novec7000 & Novec7000 100 wt\% & 298 & 0.447$\pm$0.0211 & 0.45~\cite{novec7000} \\
EA & EA 100 wt\% & 298 & 0.542$\pm$0.0071 & 0.43~\cite{lange} \\
PC & PC 100 wt\% & 298 & 1.426$\pm$0.0452 & 2.53~\cite{xu2004nonaqueous} \\
EO & EO 100 wt\% & 298 & 0.829$\pm$0.0500 & 1.1~\cite{crchandbook} \\
ACT & ACT 100 wt\% & 298 & 0.502$\pm$0.0101 & 0.31~\cite{crchandbook} \\
EP & EP 100 wt\% & 298 & 0.728$\pm$0.040 & 0.63~\cite{EP} \\

S1 & DMC\_EC$|$70\_30 & 293 & 0.720$\pm$0.0136 & 0.95 \cite{logan2018study} \\
S1 & DMC\_EC$|$70\_30 & 300 & 0.673$\pm$0.0171 & NA \\
S1 & DMC\_EC$|$70\_30 & 303 & 0.644$\pm$0.0197 & 0.83 \cite{logan2018study} \\
S1 & DMC\_EC$|$70\_30 & 313 & 0.602$\pm$0.0129 & 0.73 \cite{logan2018study} \\

S3 & EMC\_EC$|$70\_30 & 293 & 0.842$\pm$0.0126 & 1.11 \cite{logan2018study} \\
S3 & EMC\_EC$|$70\_30 & 300 & 0.820$\pm$0.0163 & NA \\
S3 & EMC\_EC$|$70\_30 & 303 & 0.835$\pm$0.0253 & 0.97 \cite{logan2018study} \\
S3 & EMC\_EC$|$70\_30 & 313 & 0.734$\pm$0.0161 & 0.87 \cite{logan2018study} \\

\bottomrule
\end{tabular}
\end{center}
\vskip -0.1in
\end{table}

\begin{table}[hbt!]
\caption{The simulated viscosities ($\eta$, in cP), ionic conductivities ($\sigma$, in mS/cm) of cation of LiFSI and LiPF$_6$ based electrolytes at 298K. The uncertainty for the conductivities calculated using Mistry's method ranges from 0.35 to 1.38 mS/cm, while the values calculated using NE method ranges from 0.11 to 2.20 mS/cm. The uncertainty for the predicted viscosity for medium and low concentrated electrolytes (P1-P9, and F1, F5-6, F8, F11) are below 0.1 cP, while the uncertainty for the remaining highly concentrated electrolytes are generally from 0.3 cP to 0.6 cP with the maximum of 3 cP for F9, respectively. The viscosity values for the carbonate based electrolytes are acquired from authors of ref\cite{dave2022autonomous} by private communications.}
\label{tab:visco_cond_elyt}
\vskip 0.15in
\begin{center}
\begin{tabular}{lcccccr}
\toprule
\small
Mixtures & Compositions & $\eta_{\text{simu}}$ & $\eta_{\text{Exp}}$ & $\sigma_{\text{Mistry}}$& $\sigma_{\text{NE}}$ & $\sigma_{\text{Exp}}$ \\

\midrule
P1 & DMC\_EC$|$50\_50$|$LiPF$_{6}$$|$0.5 & 1.891 &2.219 \cite{dave2022autonomous} & 11.201 & 12.420 & 12.14 \cite{dave2022autonomous} \\
P2 & DMC\_EC$|$70\_30$|$LiPF$_{6}$$|$0.5 & 1.656 & NA & 11.361 & 13.133 & 10.89 \cite{dave2022autonomous} \\
P3 & DMC\_EC$|$70\_30$|$LiPF$_{6}$$|$0.84 & 2.413 & NA & 11.990 & 15.106 & 12.91 \cite{dave2022autonomous}\\
P4 & DMC\_EC$|$70\_30$|$LiPF$_{6}$$|$1.0 & 2.683 & 2.734 \cite{dave2022autonomous} & 12.881 & 15.451 & 12.43 \cite{dave2022autonomous}\\

P5 & DMC\_EC$|$60\_40$|$LiPF$_{6}$$|$0.9 & 2.847 & 2.778 \cite{dave2022autonomous} & 11.531 & 14.860 & 12.793 \cite{dave2022autonomous}\\
P6 & DMC\_EC\_EMC$|$45\_50\_5$|$LiPF$_{6}$$|$1.1 & 4.716 & 4.566 \cite{dave2022autonomous} & 8.021 & 10.669 & 12.175 \cite{dave2022autonomous}\\
P7 & DMC\_EC$|$70\_30$|$LiPF$_{6}$$|$1.5 & 4.810 & 4.472 \cite{dave2022autonomous} & 8.713 & 12.241 & 12.144 \cite{dave2022autonomous}\\
P8 & DMC\_EC$|$70\_30$|$LiPF$_{6}$$|$1.3 & 3.984 & 3.767 \cite{dave2022autonomous} & 9.573 & 13.171 & 12.118 \cite{dave2022autonomous}\\
P9 & PC$|$LiPF$_{6}$$|$0.28 & 2.517 & NA & 4.735 & 5.053 & 4.967 \cite{ding2003conductivity}\\

F1 & DMC\_EC$|$51\_49$|$LiFSI$|$1.12
 & 3.548 & 3.4 \cite{wang2016superconcentrated} & 9.828 & 13.069 & 14~\cite{wang2016superconcentrated}\\
F2 & DMC\_EC$|$51\_49$|$LiFSI$|$2.25
 & 11.121 &9.8 \cite{wang2016superconcentrated} & 4.369 & 6.592 & 9.8~\cite{wang2016superconcentrated}\\
F3 & DMC\_EC$|$51\_49$|$LiFSI$|$3.74
 & 24.946 & 36.9 \cite{wang2016superconcentrated} & 2.266 & 3.527 & 4.5~\cite{wang2016superconcentrated}\\
F4 & DMC$|$LiFSI$|$2.22
 & 4.653 & 3.9 \cite{wang2016superconcentrated} & 9.237 & 13.142 & 12.2~\cite{wang2016superconcentrated}\\
F5 & EC$|$LiFSI$|$0.49
 & 3.184 & 4.1 \cite{wang2016superconcentrated} & 7.013 & 8.099 & 8.7~\cite{wang2016superconcentrated}\\
F6 & EC$|$LiFSI$|$1.14
 & 6.179 & 8.1 \cite{wang2016superconcentrated} & 5.907 & 7.672 & 9.7 \cite{wang2016superconcentrated}\\
F7 & DMC$|$LiFSI$|$3.70
 & 13.304 & 12.9 \cite{wang2016superconcentrated} & 4.363 & 6.739 & 8.1 \cite{wang2016superconcentrated}\\
F8 & DMC$|$LiFSI$|$1.11
 & 1.629 & 1.5 \cite{wang2016superconcentrated} & 15.984 & 20.209 & 9.9 \cite{wang2016superconcentrated}\\
F9 & EC$|$LiFSI$|$3.78
 & 34.183 & NA & 1.738 & 2.472 & 2.3 \cite{wang2016superconcentrated}\\
F10 & EC$|$LiFSI$|$2.27
 & 17.283 & 33.1 \cite{wang2016superconcentrated} & 2.597 & 3.063 & 5.6 \cite{wang2016superconcentrated}\\
F11 & DMC\_EC$|$51\_49$|$LiFSI$|$0.49
 & 1.85 & 1.9 \cite{wang2016superconcentrated} & 11.015 & 12.771 & 11.5~\cite{wang2016superconcentrated}\\

\bottomrule
\end{tabular}
\end{center}
\vskip -0.1in
\end{table}

\begin{table}[hbt!]
\caption{The simulated diffusion coefficients ($10^{-10}$ m$^2$/s) of cations and anions, and the calculated transference numbers in LiPF$_6$ and LiFSI-based electrolytes at 298K. }
\label{tab:diff_trans_elyt}
\vskip 0.15in
\begin{center}
\begin{tabular}{lcccccr}
\toprule
Mixtures & Compositions & D$_{+, \text{self}}$ & D$_{-,\text{self}}$ &  t$_+$ \\

\midrule
P1 & DMC\_EC$|$50\_50$|$LiPF6$|$0.5 & 2.898 & 4.298 & 0.403$\pm$0.031\\
P2 & DMC\_EC$|$70\_30$|$LiPF6$|$0.5 &3.256 & 4.651 & 0.412$\pm$0.028 \\
P3 & DMC\_EC$|$70\_30$|$LiPF6$|$0.84 & 2.587 & 3.493 & 0.425$\pm$0.027\\
P4 & DMC\_EC$|$70\_30$|$LiPF6$|$1.0 & 2.435 &3.307 & 0.424$\pm$0.035 \\

F1 & DMC\_EC$|$51\_49$|$LiFSI$|$1.12
 & 1.919 & 2.412 & 0.443$\pm$0.046 \\
F2 & DMC\_EC$|$51\_49$|$LiFSI$|$2.25
 & 0.875 & 0.952 & 0.479$\pm$0.055\\
F3 & DMC\_EC$|$51\_49$|$LiFSI$|$3.74
 & 0.548 & 0.550 & 0.499$\pm$0.056\\
 
\bottomrule
\end{tabular}
\end{center}
\vskip -0.1in
\end{table}
