# Supplementary material for: A predictive machine learning force field framework for liquid electrolyte development
Source: arXiv:2404.07181 source file (2025-04-01)
Supplement: Supplementary file 6 [file ensemble.tex]

\section{Ensemble Knowledge Distillation for MLFF}
\label{si:ensemble}
\subsection{Theory}
As noted in Ref.~\cite{fu2022forces}, MLFFs trained by different random seeds often lead to fluctuating results from MD simulations, particularly when extrapolating to systems not seen in the training set. In Figure \ref{ensemble_illustration}a, we illustrate that even if the ensemble of MLFFs is well-trained and behaves consistently and accurately within the interpolation domain, the inherent randomness of neural networks might lead to greater variability in out-of-domain inference compared with in-domain inference~\cite{martius2016extrapolation}. Consequently, the ensemble of MLFFs may exhibit significantly different behaviors within the extrapolation domain.
In Figure \ref{ensemble_illustration}b, we propose a method to constrain the behavior of different MLFFs within the extrapolation domain by training them on the mean predictions. This approach not only mitigates differences among the ensemble of MLFFs within the extrapolation domain but also reduces MLFF errors by minimizing random errors.

We illustrate the reduction of random errors by expressing the predicted energy in terms of the true energy (or other quantities such as force and virial tensor), systematic error, and random error.
\begin{equation}
    E_{\text{pred}}^{\text{initial}} = E_{\text{true}} + \delta E_{\text{systematic}}^{\text{initial}} + \delta E_{\text{random}}^{\text{initial}},
\end{equation} 
where $\delta E$ denotes the error of energy. We can write the mean of the predicted energy as:
\begin{equation}
    \overline{E_{\text{pred}}^{\text{initial}}} = E_{\text{true}} + \overline{\delta E_{\text{systematic}}^{\text{initial}}} + \overline{\delta E_ {\text{random}}^{\text{initial}}}.
\end{equation} According to the law of large number, if the mean is taken over sufficient amount of predictions, then we have $\overline{\delta E_{\text{systematic}}^{\text{initial}}} \approx \delta E_{\text{systematic}}^{\text{initial}}$ and $\overline{\delta E_{\text{random}}^{\text{initial}}} \approx 0$. Therefore, we have:

\begin{equation}
    \overline{E_{\text{pred}}^{\text{initial}}} \approx E_{\text{true}} + \delta E_{\text{systematic}}^{\text{initial}},
\end{equation} 
which implies
\begin{equation}
    |\overline{E_{\text{pred}}^{\text{initial}}} - E_{\text{true}}| < |E_{\text{pred}}^{\text{initial}} - E_{\text{true}}|.
    \label{meanerror}
\end{equation} 

In ensemble knowledge distillation, since we use $\overline{E_{\text{pred}}^{\text{initial}}}$ as the label to train the MLFF, we can write the predicted energy after ensemble knowledge distillation as:

\begin{equation}
    \begin{split}
        E_{\text{pred}}^{\text{distilled}} &= \overline{E_{\text{pred}}^{\text{initial}}} + \delta E_{\text{systematic}}^{\text{distill}} + \delta E_{\text{random}}^{\text{distill}} \\
        &\approx E_{\text{true}} + \delta E_{\text{systematic}}^{\text{initial}} + \delta E_{\text{systematic}}^{\text{distill}} + \delta E_{\text{random}}^{\text{distill}}. \\
    \end{split}
    \label{distillerror}
\end{equation} Therefore, if we properly design the training process in ensemble knowledge distillation to minimize $\delta E_{\text{systematic}}^{\text{distill}}$ and $\delta E_{\text{random}}^{\text{distill}}$, we will achieve smaller difference between $E_{\text{true}}$ and $E_{\text{pred}}^{\text{distilled}}$ than $E_{\text{pred}}^{\text{initial}}$. In the case study of solid phase transformation, we will demonstrate that following ensemble knowledge distillation, the prediction error decreases.

\begin{figure}
    \centering
    \includegraphics[width=\textwidth]{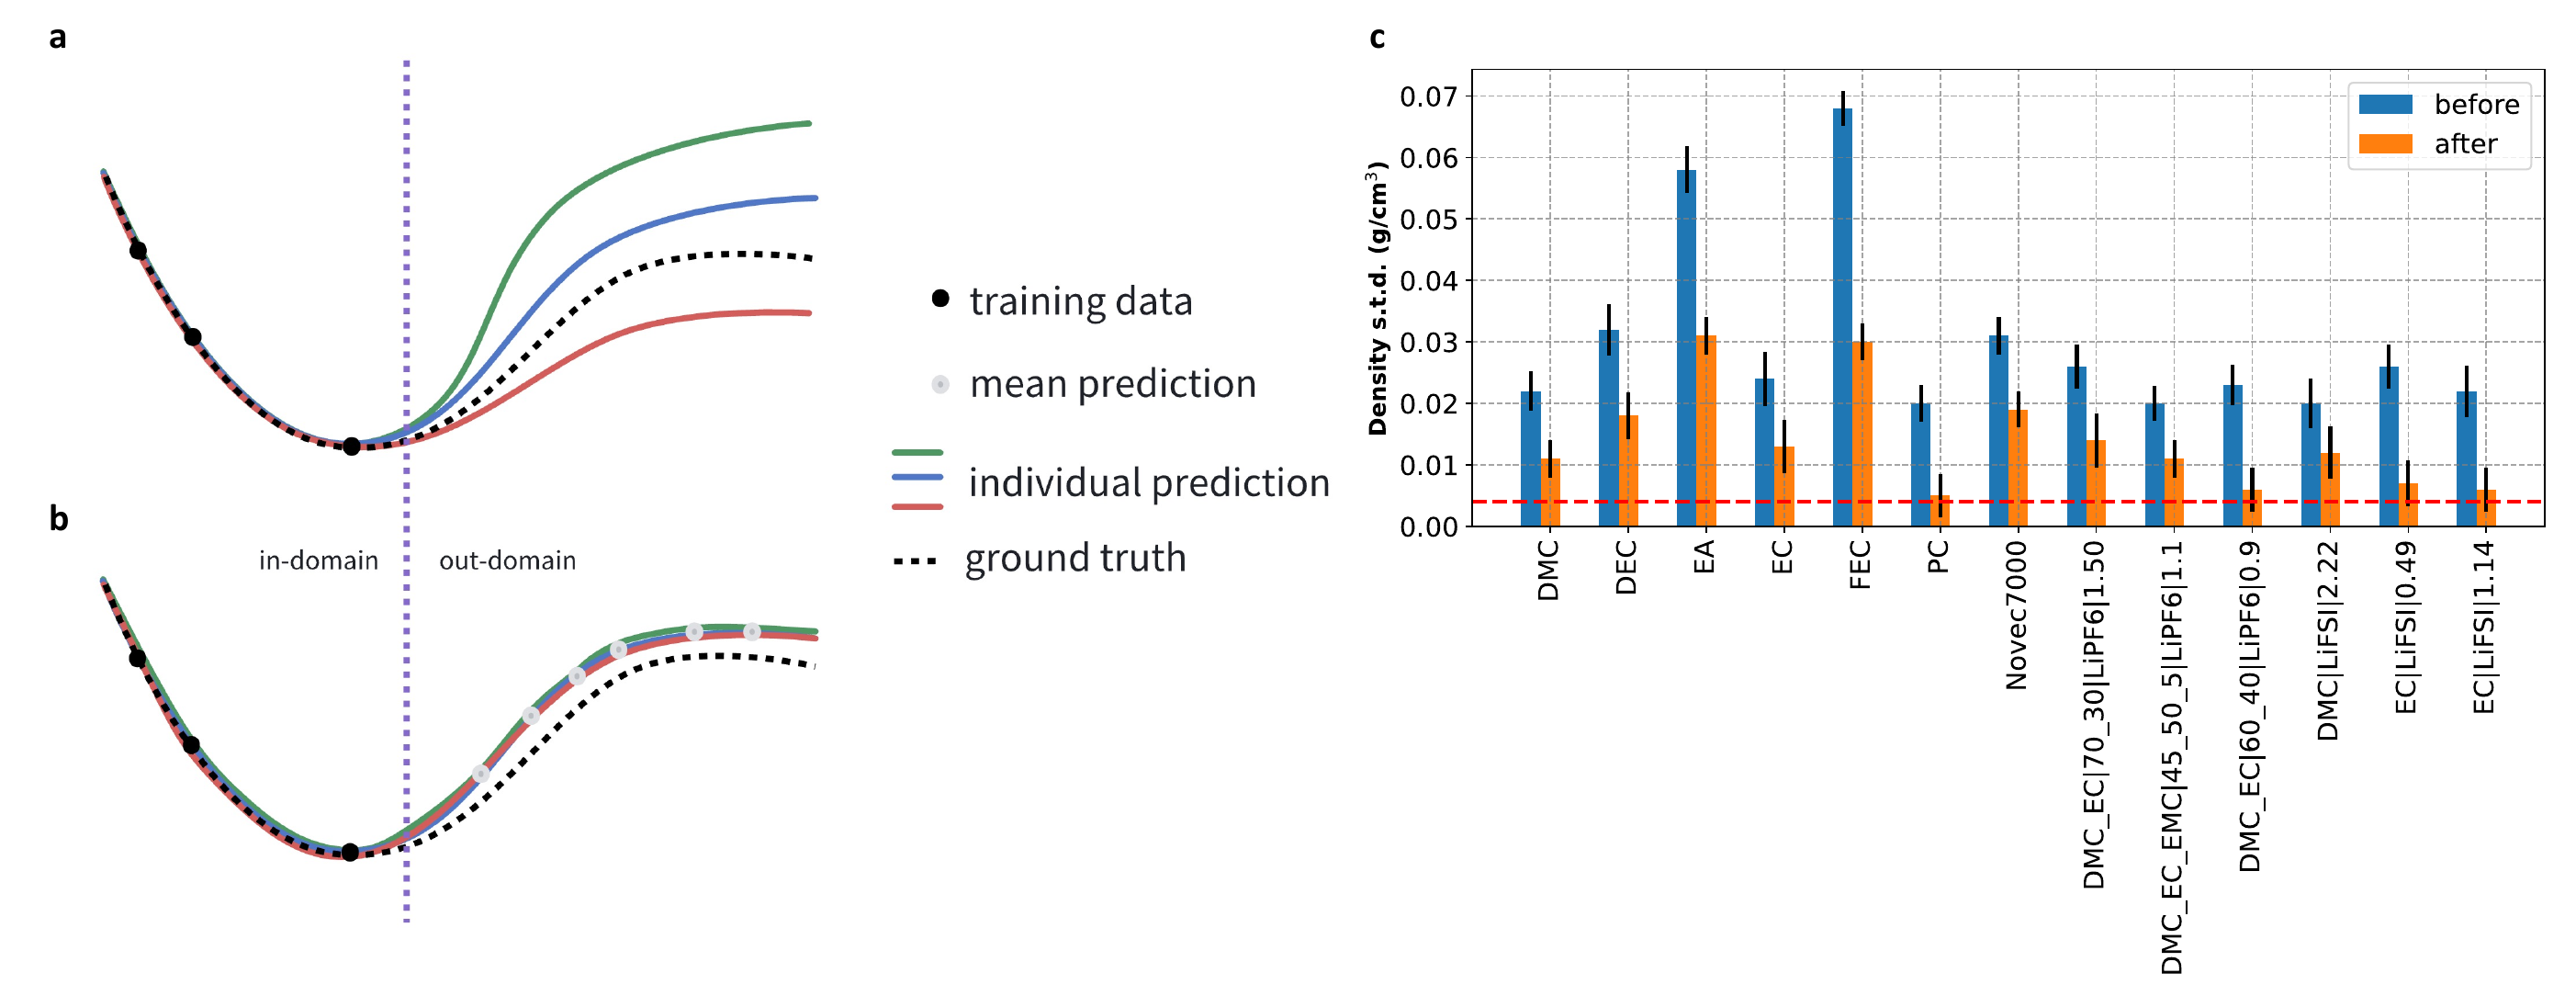}
    \caption{\textbf{\textbf{a}} and \textbf{\textbf{b}} Illustration of the interpolation and extrapolation behaviors before and after ensemble knowledge distillation, respectively. \textbf{\textbf{c}} Standard deviations of density from MD by five MLFFs before and after ensemble knowledge distillation.}
    \label{ensemble_illustration}
\end{figure}

\subsection{Case Study of Liquid Electrolytes} 
In this study, as we train MLFFs using DFT data of small gas-phase clusters and utilize them to predict properties of bulk liquid electrolytes, we essentially task MLFFs with extrapolation, which may introduce significant random noise into MD simulations. Hence, we adopt the following procedure to conduct ensemble knowledge distillation for liquid electrolytes:
\begin{enumerate}
\item Initially, we train five models purely by DFT data at random.
\item Subsequently, we randomly select one model to run 600 ps NPT MD simulations and 400 ps NVT MD simulations for all systems shown in Figure \ref{ensemble_illustration}c.
\item With the trajectories obtained from the MD simulations from the previous step, we employ all five models to predict the energy, forces, and virial tensor of 100 randomly selected frames from the trajectory of each system.
\item Finally, we use the mean predictions as the labels to finetune the randomly selected model by the following loss function:
\end{enumerate}

\begin{equation}
    \begin{split}
    L_{\text{distill}} = L_{\text{training}} + \frac{1}{N_{\text{frame}}} \sum_{k}^{N_{\text{frame}}}\sum_{i}^{N_{\text{atom}}}&\alpha_{\text{energy}}^{\text{distill}} (\overline{E_{k}^{\text{BAMBOO}}} - E_{k}^{\text{BAMBOO}})^{2} \\
         &+ \frac{1}{N_{\text{atom}}}\alpha_{\text{force}}^{\text{distill}} ||\overline{\Vec{f}_{ki}^{ \text{BAMBOO}}} - \Vec{f}_{ki}^{ \text{BAMBOO}}||^{2} \\
         &+ \alpha_{\text{virial}}^{\text{distill}} ||\overline{\textbf{T}_{k}^{ \text{BAMBOO}}} - \textbf{T}_{k}^{\text{BAMBOO}}||^{2}.
    \end{split}
    \label{ensembleloss}
\end{equation} 

Here, we incorporate $L_{\text{training}}$ into $L_{\text{distill}}$ to regulate the behavior of the distilled MLFF on DFT data. Specifically, in this study, we only fine-tune the weights of $\text{MLP}^{\text{energy}}$ of the MLFF, and we solely include the energy, forces, and virial terms in $L_{\text{training}}$ within equation~\eqref{ensembleloss}. This approach is adopted because we do not include $L_{\text{Qeq}}$ in $L_{\text{distill}}$, as it is challenging to compute $\partial E^{\text{elec}}/\partial r_{i}$ for periodic bulk systems. Consequently, we refrain from adjusting weights that would impact the prediction of charge to maintain the constraint of charge equilibrium introduced during the initial training. Note that, to compare the effect of ensemble distillation on reducing standard deviations of MD results from different models in Figure \ref{ensemble_illustration}c, we conduct distillation on all five models to calculate standard deviations from the five models. However, in the density alignment section below, we utilize only the randomly selected model to minimize computational costs.

As a result of ensemble knowledge distillation, we observe that the errors of predictions on DFT data remain almost unchanged (when $L_{\text{training}}$ is not included in $L_{\text{distill}}$, the increase in error can be up to 30\%). Additionally, we find that the deviation between predictions of the randomly selected model and ensemble mean predictions is nearly halved. For systems with 4,000 atoms, the root mean square error (RMSE) between $\overline{E_{k}^{\text{BAMBOO}}}$ and $E_{k}^{\text{BAMBOO}}$ decreases from approximately 0.41 kcal/mol/atom to 0.23 kcal/mol/atom, RMSE of forces decreases from 1.22 kcal/mol/\AA\ to 0.67 kcal/mol/\AA, and RMSE of the virial tensor decreases from 164 kcal/mol to 87 kcal/mol. Detailed information about the training process of ensemble knowledge distillation is provided in the open-source code~\cite{BAMBOOGITHUB}. In Figure \ref{Figure 2}e in the main text and Figure \ref{ensemble_illustration}c, we demonstrate that ensemble knowledge distillation can significantly reduce the variation of density from MD simulations by almost 50\%. Since density ($\rho$) correlates with the radial distribution function (RDF) as in equation~\eqref{rdf_density} where $M^{\text{avg}}$ is the average atomic mass of the system, $V_{\text{total}}$ is the total volume, and $r$ is the radius of the sphere to calculate RDF:

\begin{equation}
\rho = \frac{M^{\text{avg}}}{V_{\text{total}}}* \int_{0}^{\infty} \text{RDF}(r) 4\pi r^{2} \,dr = M^{\text{avg}}\langle \text{RDF}(r) \rangle,
\label{rdf_density}
\end{equation} the reduction of density fluctuation presented in this work also suggests the reduction of fluctuation of RDF. Therefore, the metric of density in this work is similar to the idea of using RDF to evaluate fluctuation of MD in Fu $et$ $al.$~\cite{fu2022forces}. This illustrates the efficacy of ensemble knowledge distillation in reducing the fluctuation of MD results in liquids.

\subsection{Case Study of Solid Phase Transformation}

\begin{figure}
    \centering
    \includegraphics[width=\textwidth]{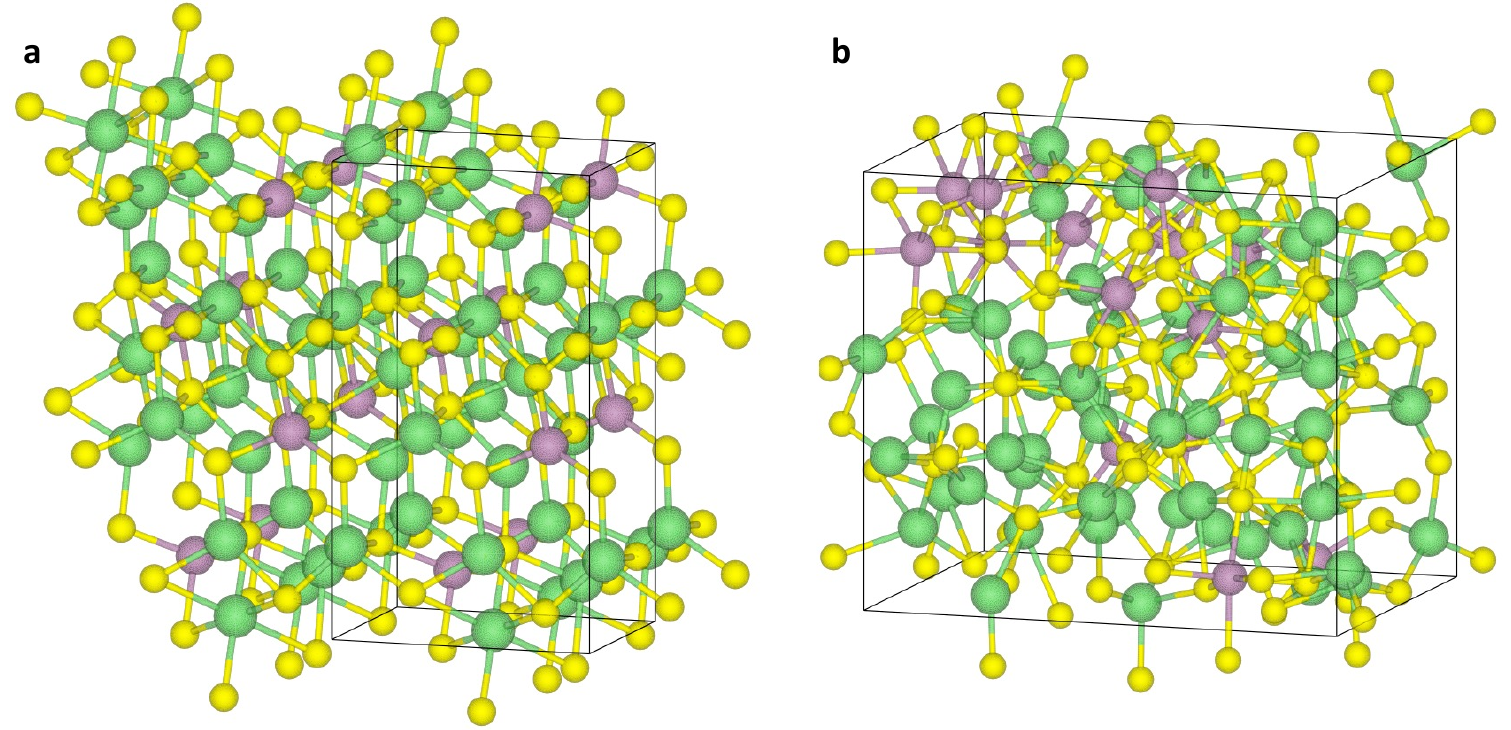}
    \caption{\textbf{\textbf{a}} and \textbf{\textbf{b}} structures of Li$_{4}$MoS$_4$ before and after the solid phase transformation (separation of the Mo rich phase and the Li rich phase), respectively. Green: Li, yellow: S, purple: Mo.}
    \label{lms}
\end{figure}

To demonstrate the broad applicability of ensemble knowledge distillation in improving the prediction performance and reducing fluctuations of results from MLFFs, we present another case study focusing on solid-phase transformation. Specifically, we investigate the system of Li${_4}$MoS$_4$, a composition similar to Li${_4}$Mo${_{0.5}}$Ti$_{0.5}$S$_4$, which is a potential cathode material for lithium-ion batteries~\cite{li4mos4}.
In this study, we explore the distribution of Mo atoms within the system. As depicted in Figure \ref{lms}a, we begin by substituting Ti atoms in the crystal structure of Li$_{4}$TiS$_4$ (mp-766540 in the Materials Project database~\cite{mp}, with the space group of Pnma) with Mo to create the Li${_4}$MoS$_4$ phase with evenly distributed Mo atoms. We subsequently optimize the crystal structure and conduct 50 ps NPT ab-initio molecular dynamics (AIMD) simulations on the initial structure.
As shown in Table \ref{behaviors}, our results indicate that while the Mo atoms remain evenly distributed at 700 K, they begin to accumulate in the upper-left corner of the simulation box at 800 K and 900 K, as illustrated in Figure \ref{lms}b. This accumulation suggests a phase transformation, specifically a phase separation between the Mo-rich phase and the Li-rich phase, during the AIMD simulations at 800 K and 900 K. The different behaviors at different temperatures might be related to the energy barrier associated with the phase transformation: the energy barrier might have the magnitude such that the thermal fluctuation at 700 K is hard to push the system through the barrier during the 50 ps MD simulation, while the thermal fluctuations at 800 K and 900 K are large enough to activate the system over the energy barrier.

In this case study, our objective is to utilize MLFFs to replicate the phase transformation and demonstrate how ensemble knowledge distillation can lower the fluctuation of reproducing the phase transformation. For this purpose, we select M3GNet, the first and one of the most widely used pretrained universal MLFFs for solids~\cite{m3gnet}.
We perform 20 ps NPT AIMD simulations with a time step of 1 fs at 300 K, 1000 K, and 10 ps at 2000 K. The initial structure for all MD simulations consists of a 2$\times$2$\times$1 supercell of crystalline Li$_{4}$MoS$_4$ with one random Li vacancy (totaling 143 atoms). Geometry optimization and AIMD are conducted using the Quantum Espresso package~\cite{qe} with the PBE functional~\cite{pbe}.
We utilize the first 10 ps trajectories of AIMD at 300 K and 1000 K as the training data to finetune the pretrained M3GNet, while the remaining 10 ps trajectories at 300 K, 1000 K, and 2000 K are used as the validation set. Employing stratified sampling with a frequency of 10 fs, we collect forces from a total of 2000 frames in AIMD trajectories as training data and 3000 frames as validation data. We optimize the pretrained M3GNet using 30 epochs with default hyperparameters as provided in the open-source code~\cite{m3gnet}. 
Here, we finetune the pretrained M3GNet with 10 different random seeds to form an ensemble of M3GNets. Using this ensemble, we predict forces for the 3000 frames in the validation set and further finetune the 10 M3GNets in the ensemble using the mean predicted forces of the validation set in conjunction with the DFT forces of the training set.
Finally, we employ all M3GNets to conduct 500 ps NPT MD simulations to observe whether phase transformation occurs. Since the Mo atoms in the initial structure are separated by 5.9 \AA\ from each other, we classify whether phase separation occurs by examining whether there is a pair of Mo atoms within 3 \AA\ of each other in the last frame of the simulation.

In Table \ref{force mae}, the data presented includes the average force error for the initial M3GNets, the distilled M3GNets' average force error, and the force error from the mean predictions of the initial M3GNet ensemble in comparison with DFT across the validation set frames. It is evident that across all three temperatures, the distilled M3GNets exhibit a reduced average error compared to the initial M3GNets, yet this error exceeds that of the ensemble's mean predictions. This finding aligns with our prior analysis, suggesting that by diminishing $\delta_{\text{random}}^{\text{initial}}$ and minimizing $\delta_{\text{systematic}}^{\text{distill}}$ and $\delta_{\text{random}}^{\text{distill}}$ as in equation~\eqref{distillerror}, we can achieve $||\overline{\Vec{f}_{\text{pred}}^{\text{initial}}} - \Vec{f}_{\text{true}}|| < ||\Vec{f}_{\text{pred}}^{\text{distilled}} - \Vec{f}_{\text{true}}|| < ||\Vec{f}_{\text{pred}}^{\text{initial}} - \Vec{f}_{\text{true}}||$. Moreover, the distilled M3GNets exhibit a significantly lower standard deviation in mean absolute error (MAE) compared to the initial M3GNets, indicating that employing ensemble knowledge distillation enhances the prediction error stability of M3GNets.

Table \ref{behaviors} illustrates that while both initial and distilled M3GNets reliably predict whether phase transformation will occur at 700K and 900K, there is a discrepancy at 800K. Here, 60\% of the initial M3GNet models predict a phase transformation, whereas the remaining 40\% do not. In contrast, post-ensemble knowledge distillation, 90\% of the distilled M3GNets anticipate a phase transformation, underscoring that distilled M3GNets offer a more unified and reliable prediction in MD simulations. It is important to acknowledge the inherent randomness in MD simulations; theoretically, with infinite simulation duration, all M3GNets should predict phase transformation. However, given that MD simulations are typically constrained by time, the limited simulation time results in the observed variability in simulation outcomes as shown in Table \ref{behaviors}. The presented case studies, encompassing both solid phase transformation and liquid electrolytes, demonstrate that ensemble knowledge distillation is an effective strategy for enhancing the reliability and consistency of MLFFs across different systems. 

It is important to note that, in this work, we primarily emphasize that the ensemble knowledge distillation algorithm can reduce the fluctuations of results obtained from MD simulations powered by MLFF, not that it could make unstable MD simulations more stable (here ``stable'' means robust against collapse due to the possible spurious reactions or nonphysical configurations in the simulations). To prevent the MLFF-based MD from collapse, one should carefully design the DFT datasets and loss function to make the potential energy surface physical, smooth, and conservative. Please refer to the section above for our efforts on making the BAMBOO MLFF stable.

\begin{table}[t]
\caption{Mean absolute error (MAE) of prediction of forces from M3GNets compared with DFT. Unit of force is eV/\AA.}
\label{force mae}
\vskip 0.15in
\begin{center}
\begin{small}
\begin{tabular}{lccc}
\toprule
Temperature & 300K & 1000K & 2000K \\
\midrule
Average MAE of initial M3GNets & 0.0749 $\pm$\ 0.008 & 0.1339 $\pm$\ 0.008 & 0.2149 $\pm$\ 0.035 \\
Average MAE of distilled M3GNets & 0.0745 $\pm$\ 2$\times10^{-5}$  & 0.1309 $\pm$\ 3$\times10^{-5}$ & 0.2036 $\pm$\ 0.0002 \\
MAE of mean predictions of initial M3GNets & 0.0740 & 0.1288 & 0.2031 \\
\bottomrule
\end{tabular}
\end{small}
\end{center}
\vskip -0.1in
\end{table}

\begin{table}[t]
\caption{Behaviors observed from AIMD, initial MLFFs, and distilled MLFFs under different temperatures for the system of Li$_{4}$MoS$_4$. ``Even'' refers to the state where Mo atoms are evenly distributed, and ``accumulated'' the state where Mo atoms are accumulated in a small region of the simulation box.}
\label{behaviors}
\vskip 0.15in
\begin{center}
\begin{tabular}{lccc}
\toprule
Temperature & AIMD, 50 ps & 10 initial MLFFs, 500 ps & 10 distilled MLFFs, 500 ps \\
\midrule
700K & Even & Even:Accumulated = 10:0 & Even:Accumulated = 10:0 \\
800K & Accumulated  & Even:Accumulated = 4:6 & Even:Accumulated = 1:9 \\
900K & Accumulated & Even:Accumulated = 0:10 & Even:Accumulated = 0:10 \\
\bottomrule
\end{tabular}
\end{center}
\vskip -0.1in
\end{table}
