# Supplementary material for: A predictive machine learning force field framework for liquid electrolyte development
Source: arXiv:2404.07181 source file (2025-04-01)
Supplement: Supplementary file 7 [file get.tex]

\subsection{Graph Equivariant Transformer}
\label{si:get}
Given atomic structures, we first initialize node scalar representation $x_{i}^{0}$ and node vector representation $\Vec{V}_{i}^{0}$ for atom $i$ based on the atom type $z_{i}$, and initialize edge scalar representation $d_{ij}$ and edge vector representation $\Vec{e}_{ij}$ based on the relative vector between atom $i$ and atom $j$ ($\Vec{r}_{ij}$) within a certain cut off radius $r_{\text{cut}}$ (5 \AA\ in this work):

\begin{equation}
x_{i}^{0}= \text{embeddingMLP} (z_{i}),
\label{node scalar representations initialization}
\end{equation}
\begin{equation}
\Vec{V}_{i}^{0}= \Vec{0},
\label{node vector representations initialization}
\end{equation}
\begin{equation}
\hat{r}_{ij}=\frac{\vec{r}_{ij}}{||r_{ij}||},
\end{equation}
\begin{equation}
d_{ij}= \text{SiLU} (W^{d}\text{RBF} (\cos{\frac{\pi||r_{ij}||}{r_{\text{cut}}}+1})),
\label{edge scalar representations initialization}
\end{equation}
\begin{equation}
\Vec{e}_{ij}= d_{ij}*\hat{r}_{ij}.
\label{edge vector representations initialization}
\end{equation} 

Here, embeddingMLP is a multi-layer perceptron (MLP) that maps discrete atom types into continuous embeddings implemented in the \textsc{nn.Embedding} class in PyTorch~\cite{pytorch}, $||\cdot||$ is the L2 norm of a vector, RBF is the radial distribution functions-based expansion as in Ref.~\cite{rbf} that expands distance into high-dimensional representations, and SiLU refers to the Sigmoid-Weighted Linear Units~\cite{silu} activation function. In equation~\eqref{edge scalar representations initialization}, $W^{d}$ refers to the weight matrix used to generate $d_{ij}$. In this work, we define ``$*$" as the following multiplication operation to combine a scalar $A \in R^{m}$ and a vector $\Vec{B} \in R^{n \times l}$, $n$ = 1 or $m$, which keeps equivariance of $\Vec{B}$.

\begin{align}
A*B &= \begin{bmatrix}
           A_{1} \\
           A_{2} \\
           \vdots \\
           A_{m}
         \end{bmatrix} * \begin{bmatrix}
           B_{11}, B_{12}, \hdots B_{1l} \\
           B_{21}, B_{22}, \hdots B_{2l} \\
           \vdots \\
           B_{n1}, B_{n2}, \hdots B_{nl}
         \end{bmatrix} = \begin{bmatrix}
           A_{1}B_{11}, A_{1}B_{12}, \hdots A_{1}B_{1l} \\
           A_{2}B_{21}, A_{2}B_{22}, \hdots A_{2}B_{2l} \\
           \vdots \\
           A_{m}B_{n1}, A_{m}B_{n2}, \hdots A_{m}B_{nl}
         \end{bmatrix}.
\label{* operation}
\end{align} 

After initialization, we input $x_{i}^{0}$, $\Vec{V}_{i}^{0}$, $d_{ij}$, $\Vec{e}_{ij}$ into the GET layers. In the n$^{th}$ layer, we first input $x_{i}^{n}$ into a LayerNorm~\cite{layernorm} layer, then we input $x_{i}^{n}$, $||r_{ij}||$, and $d_{ij}$ into the classic QKV-transformer shown in Figure \ref{Figure 1}e and described as below:

\begin{equation}
q_{i}^{n}=W^{q,n}x^{n}_{i}+b^{q,n},
\end{equation}
\begin{equation}
k_{i}^{n}=W^{k,n}x^{n}_{i}+b^{k,n},
\end{equation}
\begin{equation}
v_{i}^{n}=W^{v,n}x^{n}_{i}+b^{v,n}.
\label{qkv}
\end{equation}

Here $q_{i}^{n}$, $k_{i}^{n}$, and  $v_{i}^{n}$ are queries, keys and values in transformer~\cite{vaswani2017attention} (notice that capital $V$ stands for vector embedding whereas lowercase $v$ stands for ``values'' in QKV-attension). We further compute the attention weight $a_{ij}^{n}$ and the intermediate node scalar representation $y_{i}^{n}$. Furthermore, we build an intermediate vector representation $\Vec{u}_{i}^{ n}$ to incorporate edge vector representation $\Vec{e}_{ij}$ into the GET layer and sum contributions of neighboring atoms to the vector representation.
\begin{equation}
a_{ij}^{n}= \text{SiLU}(\langle q_{i}^{n}, k_{j}^{n}\rangle)(\cos{\frac{\pi||r_{ij}||}{r_{\text{cut}}}+1}),
\label{attention}
\end{equation}
\begin{equation}
y_{i}^{n}=\sum_{j}a_{ji}^{n}(v_{j}^{n}\odot d_{ij}),
\label{y}
\end{equation}
\begin{equation}
\vec u_{i}^{n}=\sum_{j} v_{j}^{n} * \Vec{e}_{ij}.
\label{u}
\end{equation}
Here, $\odot$ is element-wise multiplication. For the vector embeddings, we first update node vector representation $\vec V_{i}^{n}$ by linear projection:

\begin{equation}
\vec U_{i}^{1,n}=W^{U^{1},n}\vec V_{i}^{n},
\end{equation}
\begin{equation}
\vec U_{i}^{2,n}=W^{U^{2},n}\vec V_{i}^{n},
\end{equation}
\begin{equation}
\vec U_{i}^{3,n}=W^{U^{3},n}\vec V_{i}^{n}.
\end{equation} 
Then, we use inner product $\langle \cdot, \cdot \rangle$ to generate the scalar representation $w_{i}^{n} \in R^{m}$ from $\vec U_{i}^{1,n}$, $\vec U_{i}^{2,n} \in R^{m \times 3}$, which is consequently used to interact with the intermediate node scalar representation $y_{i}^{n}$:

\begin{equation}
w_{i}^{n}= \langle \vec U_{i}^{1,n},\vec U_{i}^{2,n}\rangle. 
\end{equation} 

Before final output, we further transform $y_{i}^{n}$ into three parts:

\begin{equation}
O_{i}^{1,n}=W^{O^{1},n}y_{i}^{n}+b^{O^{1},n},
\end{equation}
\begin{equation}
O_{i}^{2,n}=W^{O^{2},n}y_{i}^{n}+b^{O^{2},n},
\end{equation}
\begin{equation}
O_{i}^{3,n}=W^{O^{3},n}y_{i}^{n}+b^{O^{3},n}.
\end{equation} Finally, we output the updated node scalar representation $x_{i}^{n+1}$ and node vector representation $\Vec{V}_{i}^{n+1}$ for the $(n+1)^{th}$ layer:

\begin{equation}
    x_{i}^{n+1}=x_{i}^{n}+w_{i}^{n} \odot O_{i}^{2,n}+O_{i}^{3,n},
\end{equation}
\begin{equation}
    \vec V_{i}^{n+1} = \vec V_{i}^{n}+O_{i}^{1,n} *\vec U_{i}^{3,n}+\vec u_{i}^{n}.
\end{equation} As above, both of the node scalar and vector representations in the $(n+1)^{th}$ layer encode both scalar and vector information from both node and edge in the $n^{th}$ layer. The importance of the equivariant vector information and the transformer architecture is shown in Section~\ref{si:ablation} below.

\begin{figure}
    \centering
    \includegraphics[width=\textwidth]{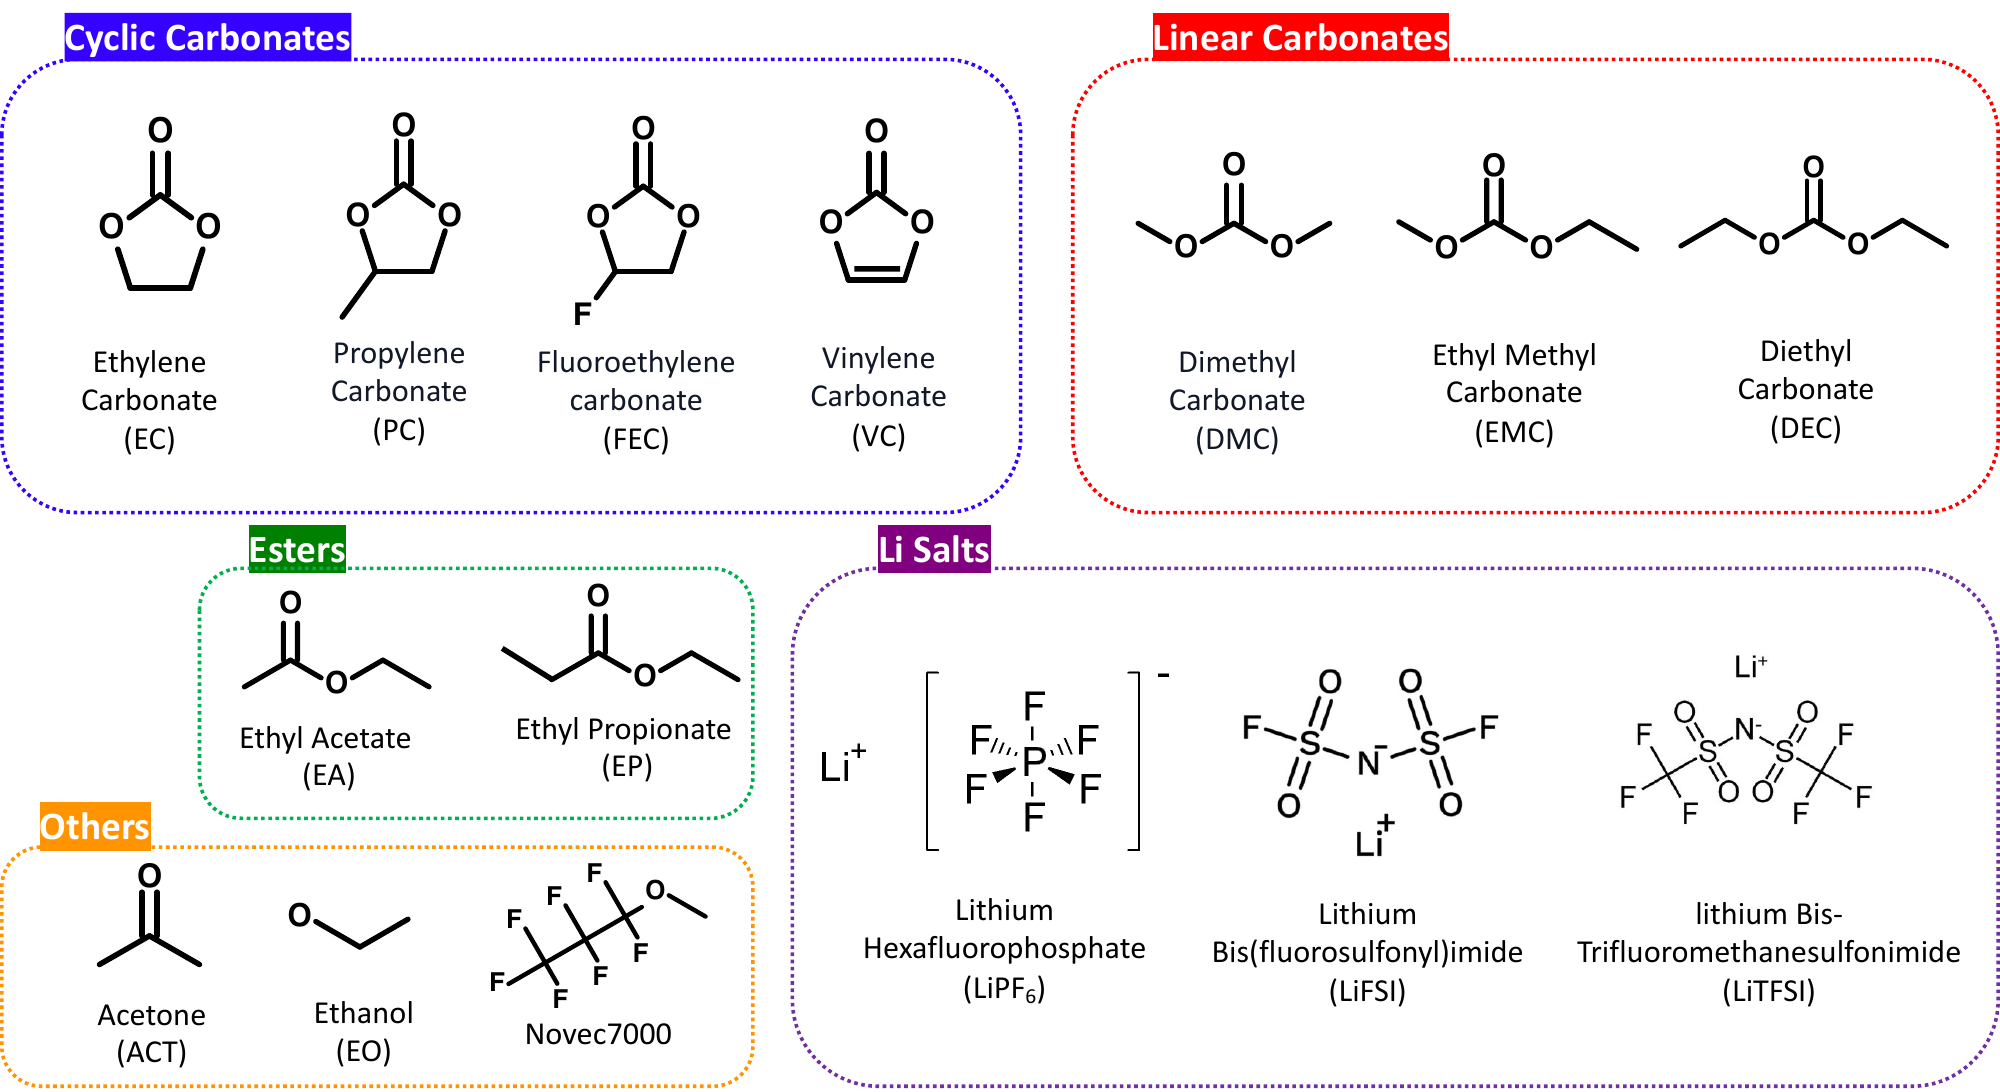}
    \caption{Schematic of the species included in the DFT dataset.}
    \label{fig:species}
\end{figure}

In this work, we refrain from calculating many-body features like bond angles and dihedral angles for two main reasons. Firstly, the GET layer in our model inherently captures all many-body effects~\cite{bodyorder} with its infinite body-order, as defined by the derivative-based understanding of many-body interactions. This means that the many-body interactions are implicitly represented. Secondly, referencing the findings from another study~\cite{matformer}, introducing explicit three-body terms into transformer-based graph neural networks does not significantly enhance the prediction of atomic structure properties, yet it substantially increases computational demand. Additionally, we avoid using tensor products to maintain fast inference speed, given that tensor products are known for their slow speed.
