# Supplementary material for: A predictive machine learning force field framework for liquid electrolyte development
Source: arXiv:2404.07181 source file (2025-04-01)
Supplement: Supplementary file 8 [file md.tex]

\section{Details of Molecular Dynamics}
\label{si:md}
We employ LAMMPS~\cite{lammps} to conduct the MD simulations for BAMBOO. For each system, an initial step involves energy minimization, which is constrained to a maximum of 1000 iterations and 100,000 evaluations. Following this, the liquid systems are subjected to equilibrium under the NPT ensemble for 1 ns, with a step size maintained at 1 fs. The density values presented in this paper represent the average measured during the final 50 ps of the NPT simulation. Subsequently, we carry out a 4 ns production run under the NVT ensemble to determine the viscosity, diffusivity, and ionic conductivity of the systems.

The viscosity ($\eta$) and diffusivity ($D$) of the pure solvents and various mixtures are computed from equilibrium simulations by applying an Einstein relation as described below: 

\begin{equation}
\eta = \cfrac{V}{2k_B T}\lim_{t\to\infty} \cfrac{d}{dt}\Biggl \langle \biggl( \int_{t_0}^{t_0+t} dt' P_{\alpha \beta}(t') \biggr)^2
 \Biggr \rangle_{t_0},
 \label{eq:vis}
\end{equation}

\begin{equation}
D = \frac{1}{6N} \lim_{t\to\infty} \cfrac{d}{dt}\Biggl \langle |\Vec{r}_{i, t+t_0} - \Vec{r}_{i, t_0}|^2 
 \Biggr \rangle_{i, t_0},
 \label{eq:diffu}
\end{equation}
where $V$ and $T$ represent the volume and the temperature of the simulations. $P_{\alpha \beta} (t')$ is the shear component of the stress tensor at the time step $t'$. $N$ represents the number of ions or molecules at interest, and $\Vec{r}_{i, t}$ the 3D coordinate of ion/molecule $i$ at time $t$, t$_0$ the starting time step, and $t$ the total number of time steps in the simulation trajectories used for viscosity or diffusivity analysis. 

Following the calculation of diffusion coefficients, we calculate transference number using the following equation: 

\begin{equation}
    t_+ = \cfrac{D_{+}}{D_{+}+D_{-}}.
\label{eq:transference}
\end{equation}

Two approaches are used to calculate ionic conductivities, that are the Nernst-Einstein method and a method described by Mistry $et$ $al$ \cite{mistry2023relative} that built on Stefan-Maxwell diffusivities. In this work, by default the ionic conductivity is calculated by Mistry $et$ $al$ \cite{mistry2023relative} unless specified. The Nernst-Einstein equation is described below: 

\begin{equation}
    \sigma_{NE} = \cfrac{e^2}{Vk_B T} (N_+z^2_+ \bar{D}_++N_-z^2_- \bar{D}_-),
\label{eq:NE}
\end{equation}
where $e$ is the elementary charge, $k_B$ the Boltzmann constant, and V and T are volume and temperature of the simulated system. $\bar{D}_{\pm}$, $z_{\pm}$, and $N_{\pm}$ are the self-diffusion coefficients, the charges, and the counts of the positive and negative ions, respectively. 

In our calculations for the diffusion coefficients and conductivities, we apply finite size correction factor (FSC) to account for the effect of simulation box sizes \cite{Maginn_Messerly_Carlson_Roe_Elliot_2018}. The FSC is calculated using the following equation: 
\begin{equation}
    \text{FSC} = \cfrac{2.837298\times k_B \times T}{6\pi \eta L},
\end{equation}
where $\eta$ is the estimated viscosity and $L$ is the simulation box length.
