# Supplementary material for: A predictive machine learning force field framework for liquid electrolyte development
Source: arXiv:2404.07181 source file (2025-04-01)
Supplement: Supplementary file 9 [file practical.tex]

\section{Results of More Practical Liquid Electrolytes}
\label{si:practical}

To demonstrate the ability of BAMBOO on simulating practical liquid electrolytes with multiple components, in this section we use the BAMBOO model after density alignment to simulate a four-component system with EC, DMC, PC, and LiPF$_{6}$ salt from Zhu $et$ $al.$~\cite{zhushang}. In Table~\ref{tab:zhushang}, we list the experimental conductivities from Zhu $et$ $al.$~\cite{zhushang} and predicted conductivities from BAMBOO and OPLS-AA. We can see that, for the four-component system, BAMBOO achieves a 25.8\% deviation compared with experiment, which is similar to the deviation of 26\% for simpler systems listed in Figure~\ref{fig:impact_of_alignment}c and lower than the 47.7\% deviation of OPLS-AA. %Moreover, BAMBOO can identify the two compositions with the highest conductivities, which demonstrates its ability on optimization of compositions of electrolytes.   

To further investigate the ability of BAMBOO on predicting properties of high-entropy liquid electrolytes, we conduct experimental measurements on some high-entropy electrolytes with 7 or 8 components as in Table~\ref{tab:highentropy}, and use BAMBOO and OPLS-AA to predict their properties. Here, DEC, EA, EC, EMC are purchased from SHINGHWA ADVANCED MATERIALS GROUP, DMC from Hi-Tech Spring, VC from JIANGSU HUAYI MACHINERY, LiPF$_{6}$ from HUNAN ZHONGLAN, and LiFSI from Do-Fluoride New Materials. All the chemicals are used as received. The electrolytes are prepared at the test environment with the cleanliness class 10,000 at the temperature 24.7 $^{\circ}$C. Density is measured by Anton Paar DMA 35 Density Meter, and viscosity is measured by Anton Paar ViscoQC-100L Viscometer.

In Table~\ref{tab:highentropy}, we show the experimentally measured and BAMBOO and OPLS-AA simulated density and viscosity of five high-entropy electrolytes composed of DEC, DMC, EA, EC, EMC, and VC as solvents and LiPF$_{6}$ and/or LiFSI as salts. We can see that, the density MAE of BAMBOO is 0.019 g/cm$^{3}$, which is higher than that (0.011 g/cm$^{3}$) in Figure S10a for simple solvents and electrolytes. The higher density error of high-entropy electrolytes is expected as the density alignment is performed only on pure solvents and simple electrolytes with one or two solvents and one salt. Despite the increase, the density error of BAMBOO (0.019 g/cm$^{3}$) for high-entropy electrolytes is still much lower than that of OPLS-AA (0.043 g/cm$^{3}$). As for viscosity of the high-entropy electrolytes, BAMBOO achieves the mean deviation of 10.1\%, which is lower than that (17\%) in Figure S10b for simple solvents and electrolytes and that of OPLS-AA (29.4\%) for the same high-entropy electrolytes. The lower density and viscosity error of BAMBOO over OPLS-AA shows the potential of BAMBOO for replacing classic force field with machine learning force field to study high-entropy electrolytes.

To further improve the performance of BAMBOO on predicting properties of high-entropy electrolytes, we propose to add their densities into the density alignment algorithm and sample more relevant atomistic structures with DFT labels to supplement the DFT dataset. Due to the exponential complexity of high-entropy electrolytes, when preparing relevant density and DFT data, sampling strategies with higher efficiency should be considered. For example, for density, one might use a surrogate model to predict the output of MD simulations by BAMBOO and evaluate prediction uncertainty, and conduct experimental measurements on the most uncertain compositions. For sampling more DFT data, compared with sampling solvation structures from MD trajectories of electrolytes as in this work, manually constructing dimer structures might be more efficient to ensure that DFT labels of all the pairs of components are included in the DFT dataset. 

\begin{table}[hbt!]
\caption{The simulated conductivities ($\sigma$) of the four component system with EC, DMC, PC, and LiPF$_{6}$ salt from Zhu $et$ $al.$~\cite{zhushang} by the BAMBOO MLFF and the OPLS-AA force field~\cite{oplsaa}. The electrolytes are presented in ``solvents$|$solvent weight $\%$$|$salt$|$salt molality'' format.} %The two compositions with the two with the highest conductivities are \underline{underscored}.}
\label{tab:zhushang}
\vskip 0.15in
\begin{center}
\begin{tabular}{lcccccr}
\toprule
\small
Compositions & $\sigma_{\text{BAMBOO}}$& $\sigma_{\text{OPLS-AA}}$ & $\sigma_{\text{Expt}}$ \\

\midrule
DMC\_EC\_PC$|$9\_9\_82$|$LiPF$_{6}$$|$0.87 & 4.04$\pm$0.08 & 4.87$\pm$0.15 & 7.63$\pm$0.02 \\
DMC\_EC\_PC$|$70\_15\_15$|$LiPF$_{6}$$|$0.96 & 10.87$\pm$0.21 & 6.64$\pm$0.97 & 13.41$\pm$0.08 \\
DMC\_EC\_PC$|$39\_29\_33$|$LiPF$_{6}$$|$0.94 & 6.47$\pm$0.12 & 6.24$\pm$0.66 & 11.52$\pm$0.05 \\
DMC\_EC\_PC$|$75\_18\_7$|$LiPF$_{6}$$|$0.96 & 11.67$\pm$0.15 & 7.02$\pm$0.21 & 13.62$\pm$0.01 \\
DMC\_EC\_PC$|$70\_8\_22$|$LiPF$_{6}$$|$0.95 & 10.74$\pm$0.26 & 6.26$\pm$0.23 & 13.4$\pm$0.01 \\
DMC\_EC\_PC$|$70\_14\_16$|$LiPF$_{6}$$|$0.95 & 11.60$\pm$0.32 & 6.48$\pm$0.12 & 13.41$\pm$0.08 \\
DMC\_EC\_PC$|$71\_21\_8$|$LiPF$_{6}$$|$0.97 & 11.64$\pm$0.54 & 7.45$\pm$0.49 & 13.69$\pm$0.08 \\
DMC\_EC\_PC$|$40\_49\_11$|$LiPF$_{6}$$|$0.96 & 7.46$\pm$0.12 & 6.28$\pm$0.43 & 11.62$\pm$0.08 \\
DMC\_EC\_PC$|$67\_3\_29$|$LiPF$_{6}$$|$0.92 & 9.99$\pm$0.39 & 6.45$\pm$0.62 & 12.65$\pm$0.05 \\
DMC\_EC\_PC$|$70\_9\_21$|$LiPF$_{6}$$|$0.95 & 10.06$\pm$0.25 & 6.66$\pm$0.31 & 13.40$\pm$0.01 \\
\bottomrule

\end{tabular}
\end{center}
\vskip -0.1in
\end{table}

\begin{table}[hbt!]
\caption{The simulated density ($\rho$, in g/cm$^{3}$) and viscosity ($\eta$, in cP) of the high-entropy liquid electrolytes. In this table, the compositions are described by eight-component tuples, with the first to the sixth elements denote the weight percentage of DEC, DMC, EA, EC, EMC, and VC, repsectively, and the last two elements molality of LiPF$_{6}$ and LiFSI, respectively. The uncertainty for the density calculated using BAMBOO and OPLS-AA ranges from 0.001 to 0.001 g/cm$^{3}$. The uncertainty for the viscosity from BAMBOO ranges from 0.018 to 0.244 cP, while that from OPLS-AA ranges from 0.076 to 0.463 cP.}
\label{tab:highentropy}
\vskip 0.15in
\begin{center}
\begin{tabular}{lcccccr}
\toprule
\small
Compositions & $\rho_{\text{BAMBOO}}$& $\rho_{\text{OPLS-AA}}$ & $\rho_{\text{Expt}}$ & $\eta_{\text{BAMBOO}}$& $\eta_{\text{OPLS-AA}}$ & $\eta_{\text{Expt}}$ \\

\midrule
(8, 6, 6, 67, 7, 6, 0.69, 0) & 1.290 & 1.268 & 1.317 & 3.746 & 5.036 & 4.409 \\
(8, 6, 12, 61, 7, 6, 0, 0.68) & 1.283 & 1.246 & 1.295 & 3.707 & 4.684 & 3.931 \\
(8, 6, 6, 67, 7, 6, 0.68, 0.68) & 1.349 & 1.327 & 1.364 & 8.467 & 12.771 & 9.764 \\
(16, 12, 12, 35, 14, 11, 0.67, 0) & 1.207 & 1.194 & 1.234 & 3.046 & 4.828 & 3.390 \\
(16, 12, 12, 35, 14, 11, 0, 0.67) & 1.220 & 1.198 & 1.235 & 3.223 & 4.264 & 3.035 \\
\bottomrule

\end{tabular}
\end{center}
\vskip -0.1in
\end{table}
