# Supplementary material for: A predictive machine learning force field framework for liquid electrolyte development
Source: arXiv:2404.07181 source file (2025-04-01)
Supplement: Supplementary file 10 [file qeq.tex]

\subsection{Charge Equilibrium}
\label{si:qeq} 

%The rationale for developing the charge equilibrium-based electrostatic energy model is to address the issue of charge dependency on atomic positions during the computation of electrostatic forces. 
It has been well-known that a fixed-charge model may impose serious restrictions on the fidelity and transferability of force fields.
However, allowing charges to vary throughout a molecular dynamics simulation is non-trivial.
Partial charge is an abstraction of electron density and should reflect the fact that electron density is at electrostatic equilibrium at any moment.
If we arbitrarily change the charge in a MD simulation, we are actually pumping energy into (or dissipating energy from) the system and violating the basic energy conservation law that is necessary to collect correct statistical results from the simulations. 
Therefore, the charges should be allowed to change to reflect the necessary physics but also restricted to obey the physical laws.
This is the central topic of polarizable force fields, and many different approaches have been developed in the past decades for different systems \cite{Polarizable_Force_Fields_for_Biomolecular_Simulations,Molecular_Dynamics_Simulations_of_Ionic_Liquids_and_Electrolytes_Using_Polarizable_Force_Fields}.

In this work, we incorporate the charge equilibrium model (Qeq here after) into our MLFF for its efficiency. 
We further use a strong regularization strategy to make our GNN model directly outputs the Qeq charges such that an expensive iterative equilibrium solver per MD timestep is completely removed.
By definition, the force (exact energy derivative) associated with the electrostatic energy should be:

\begin{equation}
    \Vec{f}_{i}^{\text{elec*}}=-\frac{\partial E^{\text{elec}}}{\partial r_{i}} = -\sum_{j}\frac{q_{i}q_{j}}{r_{ij}^{2}}\hat{r}_{ij} + \sum_{i}\chi_{i}\frac{\partial q_{i}}{\partial r_{i}} + \frac{1}{2}\sum_{i,j}\frac{1}{r_{ij}}\frac{\partial (q_{i}q_{j})}{\partial r_{i}} +  \frac{1}{2}\sum_{i}J_{i} \frac{\partial q_{i}^{2}}{\partial r_{i}}.
\label{inprinciple}
\end{equation} 

Although for non-periodic systems, $\partial E^{\text{elec}}/\partial r_{i}$ is straightforward to compute by auto-differentiation in PyTorch~\cite{pytorch}, for periodic boxes in MD simulations, most MD engines such as LAMMPS~\cite{lammps}, can only compute Ewald summation~\cite{ewald} for the long-range electrostatic force defined as below:

\begin{equation}
    \Vec{f}_{i}^{\text{elec}}=-\sum_{j}\frac{q_{i}q_{j}}{r_{ij}^{2}}\hat{r}_{ij}.
\label{elecforce}
\end{equation} 

Technically, it is difficult to explicitly compute the remaining terms in equation~\eqref{inprinciple} as it is expensive to compute $\partial q_{j} / \partial r_{i}$ for all the pairs of atoms. To bypass such difficulty, we refer to the charge equilibrium theory~\cite{Poier2019}. 

In the following, we demonstrate that, under charge equilibrium, $\Vec{f}_{i}^{\text{elec}} = \Vec{f}_{i}^{\text{elec*}}$. To simplify the notations in the proof, in the following we introduce vector $\textbf{x}=\{\chi_1, \dots \chi_N\}, \textbf{x} \in R^{N}$, and matrix $\textbf{J}:J_{ij}=1/r_{ij},J_{ii}=J_i, J \in R^{N \times N}$. We prove the following two theorems. 

\begin{theorem}
If $\textbf{q}=\{q_1,\dots,q_N\}, q \in R^{N}$, such that 
    \begin{equation}
    \textbf{q}=\arg\min_{\textbf{q}}(E(\textbf{q})-\lambda(\sum_i q_i - q_{total})),
    \label{qeqmin}
    \end{equation} where $\lambda$ is the Lagrange multiplier to ensure that $\sum_iq_i=q_{total}$, then 
\begin{equation}
    \Vec{f}_{i}^{\text{elec}}=-\frac{\partial E^{\text{elec}}}{\partial r_{i}}=-\sum_{j}\frac{q_{i}q_{j}}{r_{ij}^{2}}\hat{r}_{ij}.
\end{equation}
\label{qeqtheorem}
\end{theorem}

\textbf{Proof of Theorem A.1}
We first define the target of minimization: 
    \begin{equation}
        L(\textbf{q},\lambda)=\textbf{x}^T\textbf{q}+\frac{1}{2}\textbf{q}^T\textbf{J}\textbf{q}-\lambda(\textbf{1}^T\textbf{q}-q_{total}),
    \label{mintarget}
    \end{equation} where $\textbf{1}$ is an all-one vector. If $\textbf{q}$ is a minimizer of $L$, then
    \begin{equation}
        0=\frac{\partial L}{\partial \textbf{q}}=\textbf{x}+\frac{1}{2}\textbf{J}^T\textbf{q}+\frac{1}{2}\textbf{J}\textbf{q}-\lambda\textbf{1}=\textbf{x}+\textbf{J}\textbf{q}-\lambda\textbf{1},
    \label{qderivative}
    \end{equation} where the second ``=" is because $\textbf{J}$ is symmetric. Similarly, we also have:
    \begin{equation}
        0=\frac{\partial L}{\partial \lambda}=q_{total}-\textbf{1}^T \textbf{q}.
    \label{lambdaderivative}
    \end{equation} Now we calculate $-\partial E^{\text{elec}}/\partial r_{i}$. To simplify the writing by avoiding 3-dimensional tensors, here we consider just one dimension of $\Vec{r}_{i}$, for example, $z_{i}$, 
    \begin{equation}
        \frac{\partial E}{\partial z_i}=\frac{\partial}{\partial z_i}(\textbf{x}^T \textbf{q} + \frac{1}{2}\textbf{q}^T\textbf{J}\textbf{q})=\frac{\partial\textbf{x}^T}{\partial z_i}\textbf{q}+\textbf{x}^T\frac{\partial\textbf{q}}{dz_i}+\frac{1}{2}\frac{\partial\textbf{q}^T}{\partial z_i}\textbf{J}\textbf{q}+\frac{1}{2}\textbf{q}^T\frac{\partial\textbf{J}}{\partial z_i}\textbf{q}+\frac{1}{2}\textbf{q}^T\textbf{J}\frac{\partial\textbf{q}}{\partial z_i}.
    \label{dedr}
    \end{equation} 
Here, the term $\frac{\partial \textbf{x}^T}{\partial z_i}\textbf{q}=0$, because $\chi$ does not depend on structures. The terms $\frac{1}{2}\frac{\partial\textbf{q}^T}{\partial z_i}\textbf{J}\textbf{q}$ and $\frac{1}{2}\textbf{q}^T\textbf{J}\frac{\partial\textbf{q}}{\partial z_i}$ can be combined into $\textbf{q}^T\textbf{J}\frac{\partial\textbf{q}}{\partial z_i}$ due to the symmetry of $\textbf{J}$. The fourth term $\frac{1}{2}\textbf{q}^T\frac{\partial\textbf{J}}{\partial z_i}\textbf{q}$ is the desired expression of $\Vec{f}_{i}^{\text{elec}}$. For the remaining terms, we have:
    \begin{equation}
        \textbf{x}^T\frac{\partial\textbf{q}}{\partial z_i}+\textbf{q}^T\textbf{J}\frac{\partial\textbf{q}}{\partial z_i} =(\textbf{x} + \textbf{J} \textbf{q})^T\frac{\partial\textbf{q}}{\partial z_i} = \lambda\textbf{1}^T\frac{\partial\textbf{q}}{\partial z_i}=\lambda\frac{\partial (\textbf{1}^T \textbf{q})}{\partial z_i}=\lambda\frac{\partial q_{total}}{\partial r_i} = 0.
    \end{equation} where the second ``$=$" is from equation~\eqref{qderivative}, the fourth ``$=$" is from equation~\eqref{lambdaderivative}, and the last ``$=$" is because $q_{total}$ is a constant for a given system. Therefore, we have proved that:
    \begin{equation}
        \Vec{f}_{i}^{\text{elec}} = -\frac{\partial E}{\partial z_i} = -\frac{1}{2}\textbf{q}^T\frac{\partial\textbf{J}}{\partial z_i}\textbf{q}.
    \label{elecforceproof}
    \end{equation}

Then, we prove the reverse theorem:

\begin{theorem}
    If $\textbf{q}=\{q_1,\dots,q_N\}, q \in R^{N}$ such that it satisfies equation~\eqref{elecforceproof}, and $rank(\frac{\partial \textbf{q}}{\partial \textbf{c}})=N-1, c_i\in\{x_1,y_1,z_1,\dots x_N,y_N,z_N\}$, then there exists $\lambda$ such that $\textbf{q}=\arg\min_{\textbf{q}}(E(\textbf{q})-\lambda(\sum_i q_i - q_{total}))$.
    \label{reverseqeq}
\end{theorem}

\textbf{Proof of Theorem A.2}
    Combining equation~\eqref{dedr},~\eqref{elecforceproof} and the fact that $\frac{\partial \textbf{x}^T}{\partial z_i}\textbf{q}=0$, we have:
    \begin{equation}
        \textbf{x}^T\frac{\partial\textbf{q}}{\partial z_i}+\textbf{q}^T\textbf{J}\frac{\partial\textbf{q}}{\partial z_i} =(\textbf{x} + \textbf{J} \textbf{q})^T\frac{\partial\textbf{q}}{\partial z_i} = 0,
    \label{linearspace}
    \end{equation} which can extend to all $c_i\in\{x_1,y_1,z_1,\dots x_N,y_N,z_N\}$. We then combine all $\frac{\partial \textbf{q}}{\partial c_i}$ into a matrix with the dimensions of $3N \times N$, denoted as $\frac{\partial \textbf{q}}{\partial \textbf{c}}$. Because $\sum_i q_i = q_{total}$, therefore for all $c_i$, we have $\textbf{1}^T\frac{\partial \textbf{q}}{\partial c_i}=0$, and consequently $\frac{\partial \textbf{q}}{\partial \textbf{c}}^T \textbf{1}=\textbf{0}$. As a result, the rank of $\frac{\partial \textbf{q}}{\partial \textbf{c}}$ is at most $N-1$. If $rank(\frac{\partial \textbf{q}}{\partial \textbf{c}})=N-1$ as in the theorem, then due to equation~\eqref{linearspace}, $\textbf{x}+\textbf{J}\textbf{q}$ is in the linear space spanned by ${\textbf{1}}$. Therefore, there exists $\lambda$ such that $\textbf{x}+\textbf{J}\textbf{q}=\lambda\textbf{1}$, which also means $\frac{\partial L(\textbf{q})}{\partial\textbf{q}}=0$ where $L$ is defined in equation~\eqref{mintarget}. Because $\frac{\partial^2 L(\textbf{q})}{\partial \textbf{q}^2}=\textbf{J}$, where $J$ is a diagonally-dominant matrix with all positive diagonal elements, $\frac{\partial^2 L(\textbf{q})}{\partial \textbf{q}^2}$ is a positive-definite matrix, therefore $L(\textbf{q})$ is a positive definite quadratic form of $\textbf{q}$, and $\textbf{q}$ is the global minimizer of $L(\textbf{q})$. 

%Note that the requirement of $rank(\frac{\partial \textbf{q}}{\partial \textbf{c}})=N-1$ is not theoretically guaranteed. If $\textbf{q}$ is predicted by a "fully-connected" graph neural network, and if the gradients of the weight matrix and the activation function in the GNN are full-rank, then $rank(\frac{\partial \textbf{q}}{\partial \textbf{c}})=N-1$ is guaranteed. In practice, most of neural networks would satisfy the rank requirement.

From theorem \ref{qeqtheorem}, we know that the predicted charge $\textbf{q}$ should satisfy equation~\eqref{qeqmin} to ensure that $\Vec{f}_{i}^{\text{elec}}$ is strictly conservative. However, in practice, to satisfy equation~\eqref{qeqmin}, the time complexity to compute matrix $\textbf{J}$ is $\mathcal{O}(N^2)$, and the time complexity to compute the inverse of $\textbf{J}$ is $\mathcal{O}(N^3)$. Since the time complexity of the GET layers is $\mathcal{O}(N)$, computing $\textbf{J}$ and $\textbf{J}^{-1}$ would largely slow down the MD simulation for large systems with thousands of atoms. For example, in the very recent work by Hu $et$ $al.$~\cite{fullqeq}, it is shown that the cost of calculating the full Qeq for a system with 5,000 atoms is around 1 second per step per GPU, which equals to 90 ps per day per 5,000 atoms (with the time step of 1 fs as this work). We can see that the speed of calculating full Qeq is much slower than the BAMBOO model (5 ns per day per 5,000 atoms) and not practical for simulating liquid electrolytes where thousands of atoms and nanoseconds of MD simulation are required. Moreover, since there is energy dissipation in the NPT and NVT ensembles used for studying liquid electrolyte in MD, small energy drift by non-conservative force would not affect results from MD simulations. In Ref.~\cite{qrnnmethod}, the authors use a recursive method to approximate equation~\eqref{qeqmin} with the time complexity of $\mathcal{O}(N)$. However, this recursive method would also slow down the inference speed, the degree of which depends on the number of iterations: the closer approximation, the more iterations, and the slower inference speed.

In this work, we design a method to approximate charge equilibrium in equation~\eqref{qeqmin} with the minimum increase of inference speed, in which we decouple the inference speed with the degree of approximation. Instead of additional operations at inference, we move the approximation to the training process by adding a loss term in equation~\eqref{trainingloss} to minimize the difference between $\Vec{f}_{i}^{\text{elec}}$ and $\Vec{f}_{i}^{\text{elec*}}$, which is an approximation to charge equilibrium as in Theorem \ref{reverseqeq}:

\begin{equation}
    L_{\text{Qeq}} = ||\Vec{f}_{i}^{ \text{elec}} - \Vec{f}_{i}^{ \text{elec*}}||^{2}.
    \label{qeqloss}
\end{equation} Although this method seems straightforward as it directly minimizes the difference between the electrostatic force we can compute and the derivative of the electrostatic energy with respect to coordinates, equation~\eqref{qeqloss} actually has the physical meaning of charge equilibrium as in the Theorems \ref{qeqtheorem} and \ref{reverseqeq}. The degree of approximation depends on the magnitude of the weight factor of $\alpha_{Qeq}$ in the total loss as below. We show the importance of $\alpha_{Qeq}$ in Figure \ref{nve}a, where smaller weight factors results in significant energy drift, while the largest weight factor only leads to 0.02 kcal/mol/atom energy increase in the 800 ps NVE simulation. This degree of energy drift is negligible in MD simulations with the NVT and NPT ensemble, as there is energy dissipation in this two ensembles. In Figure \ref{nve}b and c, we show that the temperature of 1 ns NVT MD simulation and 4 ns NPT simulation slightly fluctuates around the set temperature of the simulation (303 K), and pressure around one atmosphere, which demonstrates the stability of the MD simulation. This method of charge equilibrium regularization minimally increases the inference speed by adding two summation over atoms as in equation~\eqref{qeq}. 

\begin{figure}
    \centering
    \includegraphics[width=\textwidth]{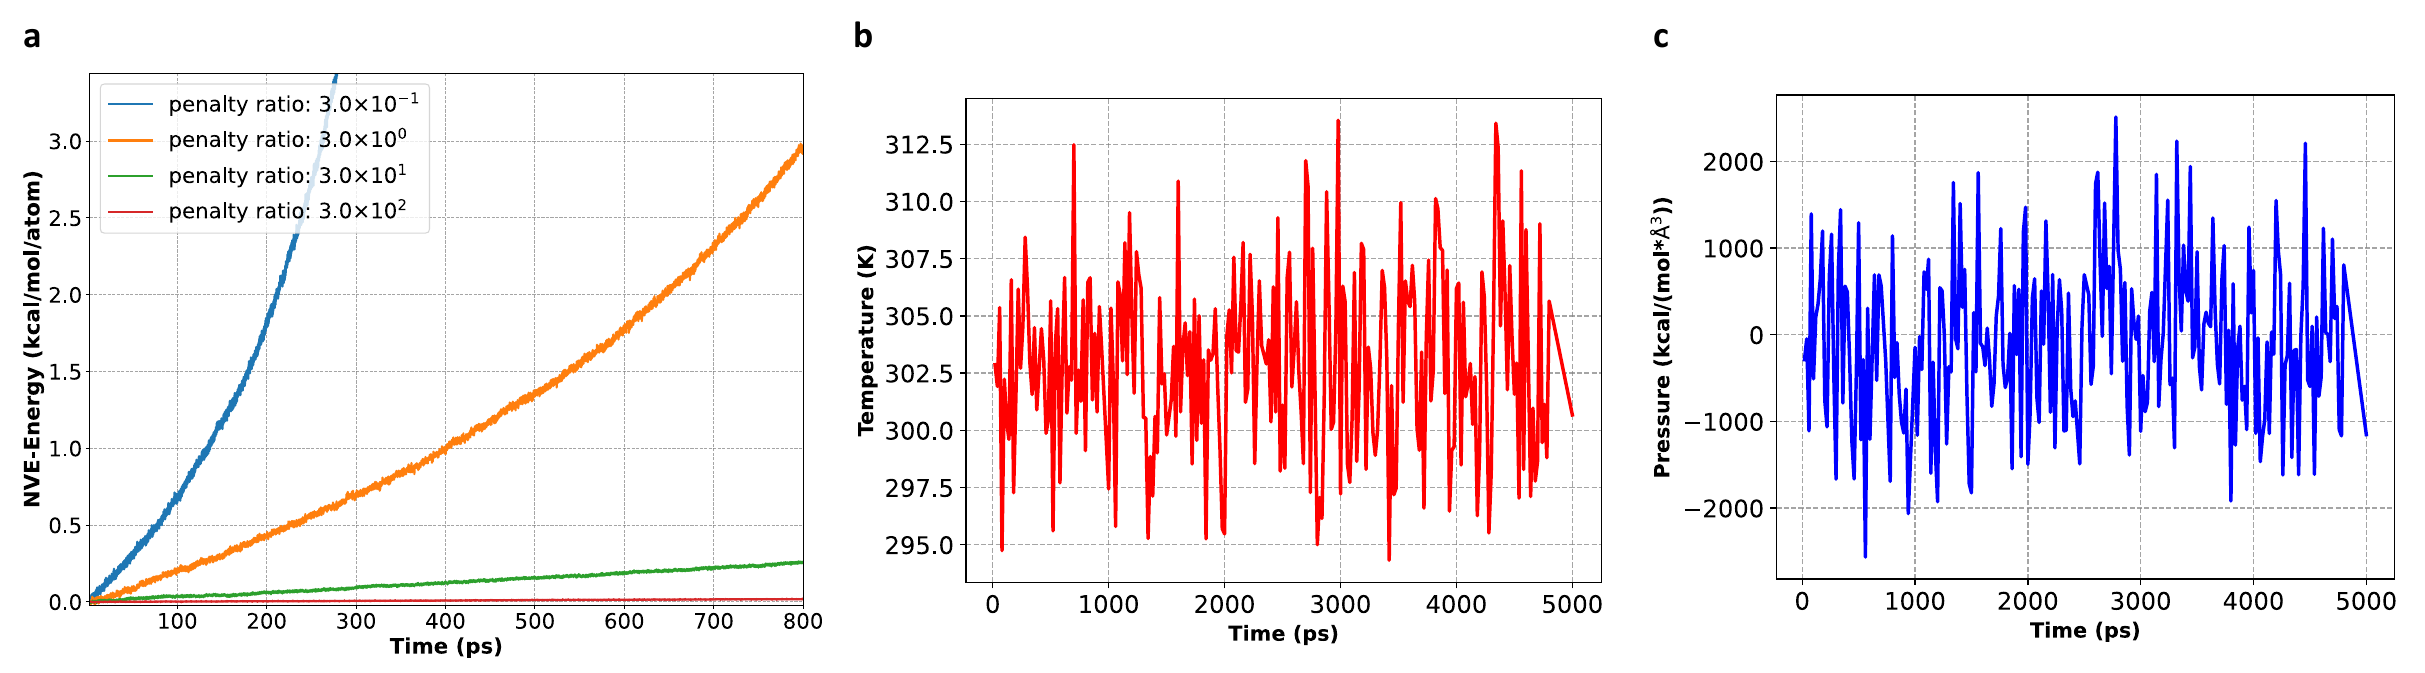}
    \caption{\textbf{a} Energy drift in molecular dynamics simulations by NVE ensemble. The simulated system is EC$|$LiPF6$|$0.95. \textbf{b} and \textbf{c} Temperature and pressure versus simulation time of DMC$\_$EC$|$51$\_$49$|$LiFSI$|$0.49, respectively.}
    \label{nve}
\end{figure}

To more clearly demonstrate the role of $L_{\text{Qeq}}$ on approximating energy derivative, we further compare the difference between $\Vec{f}_{i}^{ \text{elec}}$ and $\Vec{f}_{i}^{ \text{elec*}}$ and the different microscopic behavior and bulk observables from MLFFs with different $\alpha_{Qeq}$. At the beginning of this project, we did not consider $L_{\text{Qeq}}$ ($\alpha_{Qeq}$ = 0), because we thought that if we train the MLFF well, then the predicted force should be close to DFT force and everything would be fine. However, we found that MD simulations containing DMC and Li salts might randomly crash because of the spurious C-H bond breaking event at the methyl group of DMC. This phenomenon is not trivial because the energy landscape of the C-H bond from the MLFF is reasonable as in Figure~\ref{fig:smooth}b. After analyzing the MD trajectory, we realized that the C-H bond breaking was a result of randomly happened fast spin of the methyl group that is close to a Li ion, as illustrated in Figure~\ref{fig:smooth}a.

With the background, we show the effect of including $\alpha_{Qeq}L_{\text{Qeq}}$ in the loss term on the cluster in Figure~\ref{fig:smooth}a. We first directly compare $\Vec{f}_{i}^{ \text{elec}}$ and $\Vec{f}_{i}^{ \text{elec*}}$. From Table~\ref{tab:qeqcoef}, we can see that larger $\alpha_{Qeq}$, smaller $||\Vec{f}_{i}^{ \text{elec}} - \Vec{f}_{i}^{ \text{elec*}}||$, which clearly demonstrates the effectiveness of approximating the exact energy derivative. Then, we consider two quantities related to the rotation of the methyl H atom, accumulated work $W_{\text{circle}}$ and momentum $M_{\text{circle}}$ from one circle of rotation:

\begin{equation}
    W_{\text{circle}} = \int_{circle} \Vec{f}_{i}^{ \text{elec}} \cdot d\Vec{r},
\label{circlework}
\end{equation}

\begin{equation}
    M_{\text{circle}} = \int_{circle} \Vec{f}_{i}^{ \text{elec}} \times \Vec{r}_{C-H}.
\label{circlework}
\end{equation} In principle, $W_{\text{circle}}$ and $M_{\text{circle}}$ should be zero if the force is the exact derivative of the electrostatic energy. If not, then the accumulated energy and momentum might drive the H atom to spin. As in Table~\ref{tab:qeqcoef}, larger $\alpha_{Qeq}$, smaller $W_{\text{circle}}$ and $M_{\text{circle}}$, and consequently, when $\alpha_{Qeq}$ reaches 30 and 300, we do not observe spin of the methyl group and C-H bond breaking during the 5 ns MD simulations. Out of an abundance of caution, in this work we set $\alpha_{Qeq}$ to be 300, and during all the production MD simulations in this work, there is no spin of methyl group and spurious bond breaking event. 

As for the bulk properties from MLFFs trained with different $\alpha_{Qeq}$, from Table~\ref{tab:qeqcoef} we do not observe a clear trend between $\alpha_{Qeq}$ and density $\rho$ and Li diffusivity D$_{\text{Li}}$, although we can see that smaller $\alpha_{Qeq}$, larger fluctuation of bulk properties. Since we calculate $\rho$ and D$_{\text{Li}}$ by trajectories before C-H bond breaking, intuitively the shortening of trajectories introduces additional noise into the computation of $\rho$ and D$_{\text{Li}}$. The independence of the mean of bulk properties on $\alpha_{Qeq}$ might be because, the predicted force does not largely depend on $\alpha_{Qeq}$ as force itself is a label included in the training and finetuning process. In other words, the performance of prediction of force and downstream observables is mainly determined by whether the MLFF learns DFT labels and experimental labels well. As in Table~\ref{tab:qeqcoef}, even when $\alpha_{Qeq} = 0$, $||\Vec{f}_{i}^{ \text{elec}} - \Vec{f}_{i}^{ \text{elec*}}||$ is just 0.178 kcal/(mol*\AA), which is 8.1\% of the force prediction RMSE (2.19 kcal/(mol*\AA)), and 4.7\% of the magnitude of DFT force of the H atom (3.76 kcal/(mol*\AA)). We can also see that, $||\Vec{f}_{i}^{ \text{elec}}-\Vec{f}_{i}^{ \text{elec*}}||$ is smaller than $||\Vec{f}_{i}^{ \text{BAMBOO}}-\Vec{f}_{i}^{ \text{DFT}}||$, except when $\alpha_{Qeq} = 0$ where the two quantities are comparable. Therefore, we argue that the degree of approximating exact energy derivative does not largely affect the downstream observables, because the difference between predicted force and exact energy derivative is smaller than the difference between predicted force and target force label.

\begin{table}[hbt!]
\caption{Comparison between behaviors of MLFFs trained with different $\alpha_{Qeq}$. Forces, work, and momentum are calculated for the methyl H atom marked in Figure~\ref{fig:smooth}a. Spin of methyl group, C-H bond breaking, density, and Li diffusivity are measured from the 5 ns MD simulations of the DMC\_EC$|$70\_30$|$LiPF6$|$1.0 system, and density $\rho$ and Li diffusivity D$_{\text{Li}}$ are calculated by trajectories before C-H bond breaking. Units: $f$: (kcal/(mol*\AA)); $W$ and $M$: (kcal/mol); $\rho$: (g/cm$^3$); D$_{\text{Li}}$: ($10^{-10}$ m$^2$/s).}
\label{tab:qeqcoef}
\vskip 0.15in
\begin{center}
\begin{tabular}{lcccccr}
\toprule
Behaviors & $\alpha_{Qeq}=0$ & $0.3$ & $3$ & $30$ & $300$ \\

\midrule
$||\Vec{f}_{i}^{ \text{elec}}-\Vec{f}_{i}^{ \text{elec*}}||$& 0.178 & 0.107 & 0.054 & 0.020 & 0.007\\
$||\Vec{f}_{i}^{ \text{BAMBOO}}-\Vec{f}_{i}^{ \text{DFT}}||$& 0.180 & 0.290 & 0.240 & 0.302 & 0.139\\
$W_{\text{circle}}$& $8.9*10^{-3}$ & $2.8*10^{-3}$ & $2.1*10^{-3}$ & $1.0*10^{-3}$ & $5.5*10^{-4}$ \\
$M_{\text{circle}}$& 0.105 & 0.036 & 0.022 & 0.007 & 0.001 \\
Spin of methyl group& Yes & Yes & Yes & No & No \\
C-H bond breaking& Yes & Yes & Yes & No & No \\
$\rho$& 1.219$\pm$0.021 & 1.228$\pm$0.015 & 1.217$\pm$0.009 & 1.216$\pm$0.004 & 1.221$\pm$0.003 \\
D$_{\text{Li}}$& 2.401$\pm$0.246 & 2.378$\pm$0.155 & 2.523$\pm$0.132 & 2.542$\pm$0.073 & 2.435$\pm$0.061 \\
 
\bottomrule
\end{tabular}
\end{center}
\vskip -0.1in
\end{table}
