# Supplementary material for: A predictive machine learning force field framework for liquid electrolyte development
Source: arXiv:2404.07181 source file (2025-04-01)
Supplement: Supplementary file 11 [file separation.tex]

\subsection{Separation of Interactions}
\label{si:separation}
Once we reach the final GET layer (n$^{th}$ layer as below, and n=3 in this work), we compute NN-based per atom energy $E_{i}^{\text{NN}}$ and atomic partial charges $q_{i}$ based on $x_{i}^{n}$ by two MLPs:

\begin{equation}
    E_{i}^{\text{NN}} = \text{MLP}^{\text{energy}}(x_{i}^{n}),
\label{energymlp}
\end{equation} 
\begin{equation}
    q_{i} = \text{MLP}^{\text{charge}}(x_{i}^{n}),
\label{chargemlp} 
\end{equation} and we compute NN-based forces by:

\begin{equation}
    \Vec{f}_{ij}^{\text{ NN}} = -\frac{\partial E^{\text{NN}}}{\partial r_{ij}}+\frac{\partial E^{\text{NN}}}{\partial r_{ji}},
    \Vec{f}_{i}^{\text{ NN}}=\sum_{j\neq i}\Vec{f}_{ji}^{\text{ NN}}.
    \label{nnfij}
\end{equation}

Then, we define the electrostatic energy model based on the charge equilibrium theory~\cite{Poier2019}:

\begin{equation}
    E^{\text{elec}} = \sum_{i} \chi_{i} q_{i} + \frac{1}{2}\sum_{i,j} \frac{q_{i}q_{j}}{r_{ij}} + \frac{1}{2}\sum_{i}J_{i}q_{i}^{2}. 
\label{qeq}
\end{equation} Here, $\chi_{i}$ is the element-wise electronegativity, and $J_{i}$ is the element-wise electronic hardness. The reason behind why we do not predict $\chi$ and $J$ based on structures is stated in the proof of Theorem~\ref{qeqtheorem} in the next section. In this work, both of the two quantities only depend on atomic types and are learned and predicted by MLPs:

\begin{equation}
\chi_{i} = (\text{MLP}^{\chi}(x_{i}^{0}))^{2},
\label{chi}
\end{equation}
\begin{equation}
J_{i} = (\text{MLP}^{\text{J}}(x_{i}^{0}))^{2}.
\label{j}
\end{equation} Here we use the square of the outputs of the two MLPs to ensure that both of the two quantities are positive. More discussion about charge equilibrium is provided in the next section.

In addition, given atomic structures, we can directly compute dispersion interaction ($E_{i}^{\text{disp}}$ and $\Vec{f}_{i}^{\text{ disp}}$) by the D3 correction~\cite{2015_Schröder}. Note that we do not include dispersion correction in the DFT training data and therefore do not consider $E_{i}^{\text{disp}}$ and $\Vec{f}_{i}^{\text{ disp}}$ in the whole training process. We only incorporate dispersion correction in BAMBOO during MD simulations. Finally, we combine NN, electrostatic, and dispersion interactions to compute the total energy and force of each atom: 

\begin{equation}
    E_{i}^{\text{total}} = E_{i}^{\text{NN}} + E_{i}^{\text{elec}} + E_{i}^{\text{disp}},
\end{equation}

\begin{equation}
     \Vec{f}_{i}^{ \text{total}} = \Vec{f}_{i}^{ \text{NN}} + \Vec{f}_{i}^{ \text{elec}} + \Vec{f}_{i}^{ \text{disp}}.
\end{equation} We further compute the virial tensor $\textbf{T}$ based on pairwise forces:

\begin{equation}
    \Vec{f}_{ij} = \Vec{f}_{ij}^{ \text{NN}} + \Vec{f}_{ij}^{ \text{elec}} + \Vec{f}_{ij}^{ \text{disp}},
\end{equation}

\begin{equation}
    \textbf{T} = \sum_{i}^{N} \sum_{j}^{N} \Vec{f}_{ij} \otimes \Vec{r}_{ij}, 
    \label{virial}
\end{equation} where $\otimes$ is the outer product between the two 3-dimensional vectors. Here, according to equation \eqref{nnfij} and \eqref{elecforce} and the nature of $\Vec{f}_{ij}^{ \text{disp}}$, $\Vec{f}_{ij} = - \Vec{f}_{ji}$, which satisfies the Newton's Third Law of opposite forces for computing the microscopic stress~\cite{TORRESSANCHEZ2016224}, and since we compute $\Vec{r}_{ij}$ across periodic boundary, we do not need additional correction for computing $\textbf{T}$ of periodic systems. We also compute the dipole moment as $\Vec{D} = \sum_{i=1}^{N} q_{i} \Vec{r}_{i}$ for training the machine learning model.

In this work, we use a cosine cutoff function as in equation~\eqref{edge scalar representations initialization} and equation~\eqref{attention} to ensure that the expanded distance feature $d_{ij}$ and the attention score $a_{ij}^{n}$ smoothly decay to zero at the cutoff distance $r_{\text{cut}}$. Since all mathematical operations used in this work are smooth and differentiable, the outputs of the model should also be smooth and differentiable. To demonstrate smoothness of the potential energy surface, we plot the energy change of C-H bond stretching in a cluster with a Li ion and a DMC molecule as in Figure~\ref{fig:smooth}a. As we can see in in Figure~\ref{fig:smooth}b, the energy of the cluster changes smoothly from less than 1\AA\ to 7\AA\, which demonstrates the smoothness of potential energy surface from a unphysically small distance to a unphysically large distance. 

\begin{figure}
    \centering   \includegraphics[width=1.0\textwidth]{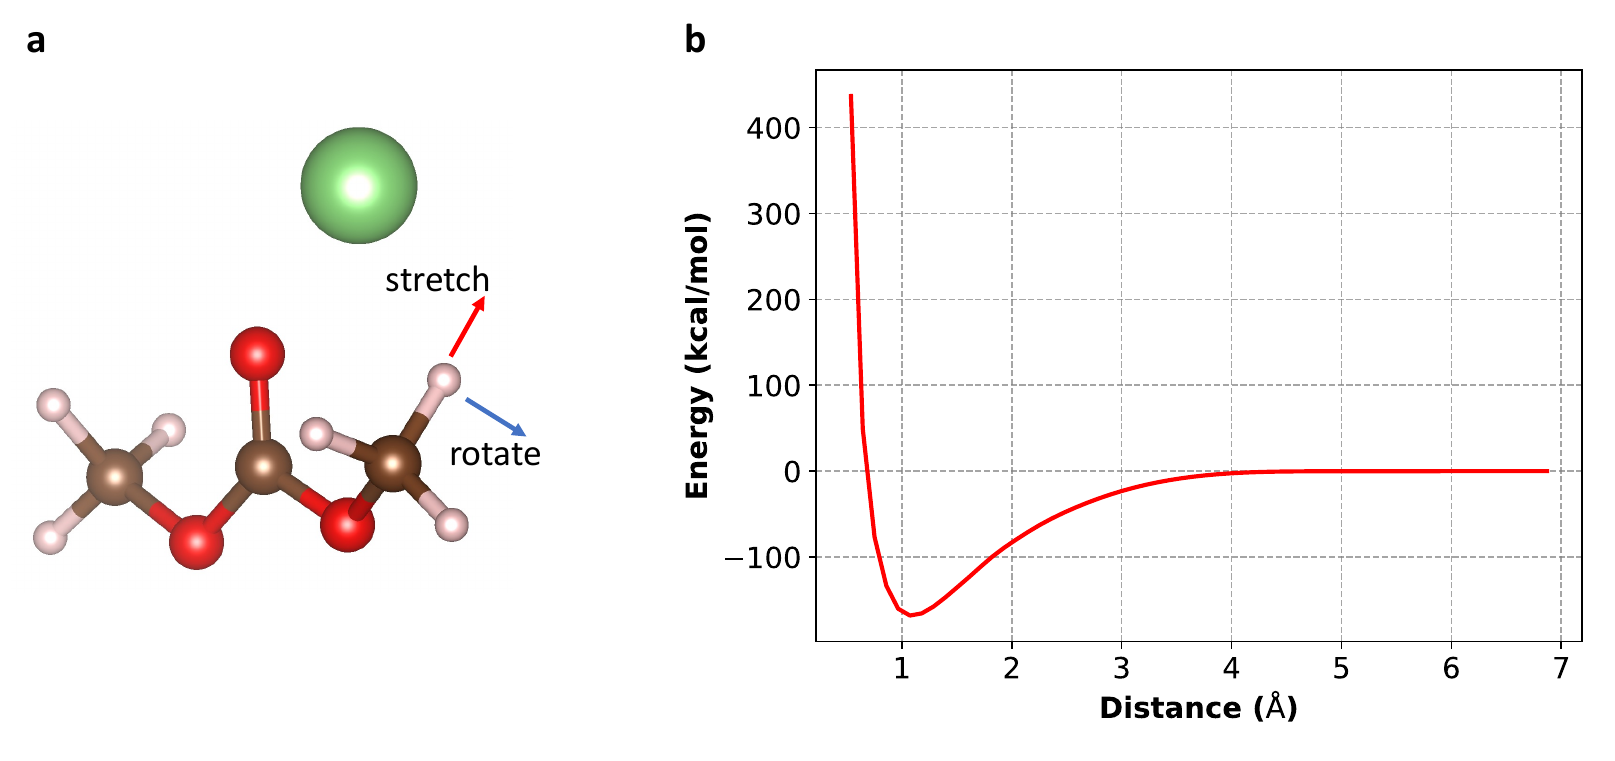}
    \caption{\textbf{Smoothness of the potential energy surface.} \textbf{a} Illustration of a cluster with a Li ion and a DMC molecule. Color coding: Li: green; C: brown; O: red; H: pink. \textbf{b.} Predicted energy versus distance between the stretched H atom and the closest C atom. The stretching direction is along the bond vector between C and H as in \textbf{a}.}
    \label{fig:smooth}
\end{figure}
