# Supplementary material for: A predictive machine learning force field framework for liquid electrolyte development
Source: arXiv:2404.07181 source file (2025-04-01)
Supplement: Supplementary file 12 [file simple.tex]

\section{Properties of Simple Liquid Electrolytes}
\label{si:simpe_system}

\begin{figure}
    \centering
    \includegraphics[width=1.0\textwidth]{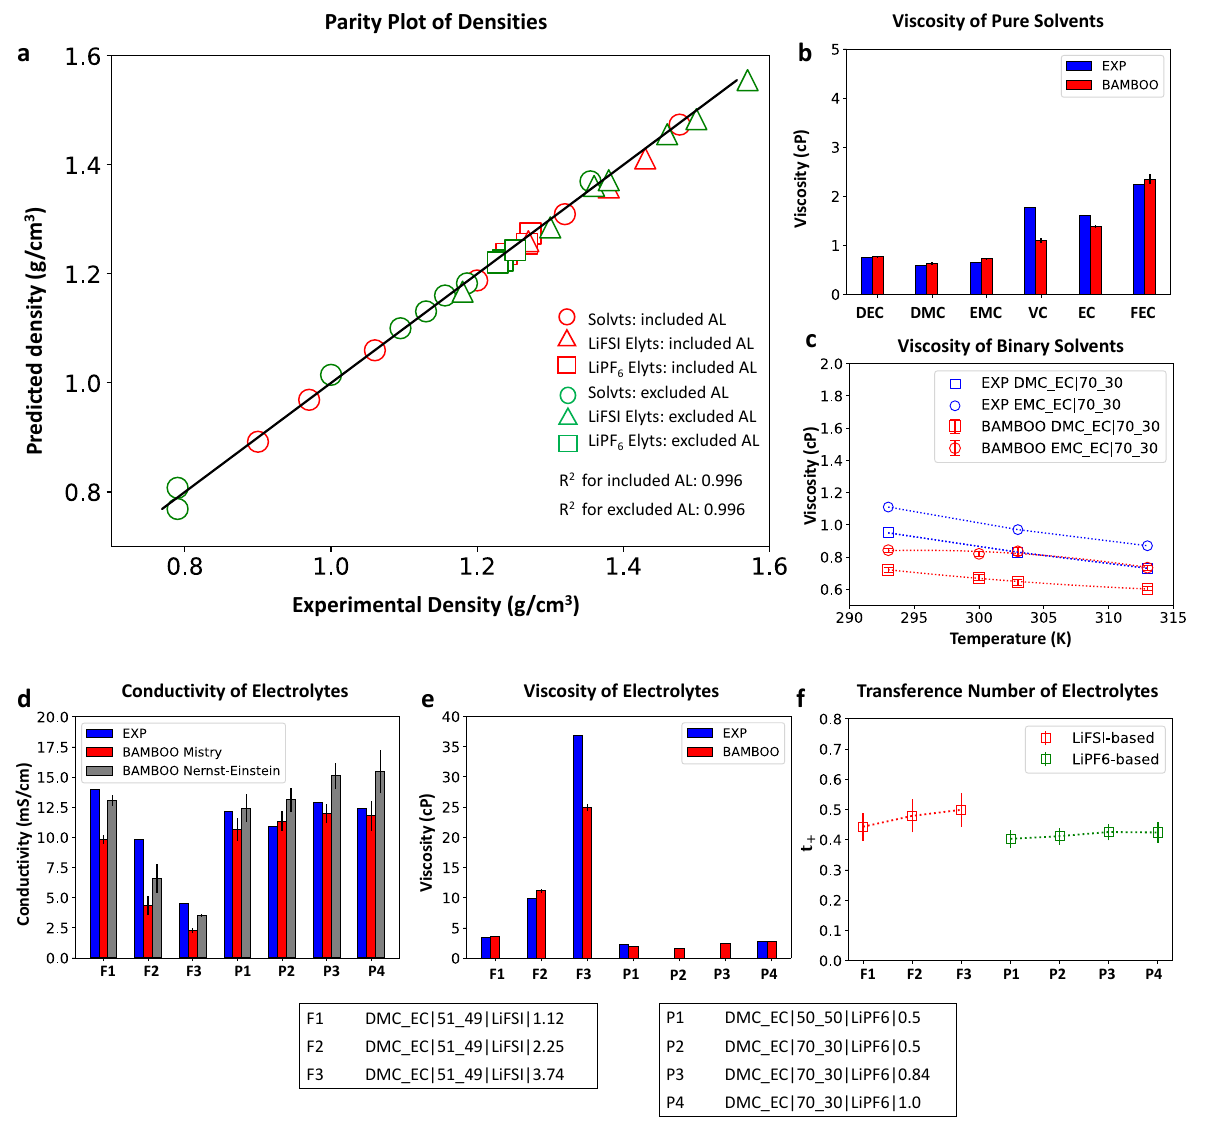}
    \caption{\textbf{The predicted solvents and liquid electrolytes' properties using BAMBOO.} \textbf{a.} The parity plot comparing the predicted and experimentally measured densities of pure solvents, solvent mixtures, LiPF$_6$ and LiFSI containing electrolytes. ``AL'' in the legend represents the density ``alignment'' treatment. \textbf{b.} The predicted viscosity of common solvents compared to experimental measurements. \textbf{c.} Comparing the predicted viscosity of DMC-EC and EMC-EC solvent mixtures as a function of temperature to experimental results. \textbf{d.} Comparing the predicted and experimental conductivity of 7 common liquid electrolytes. The conductivity values presented are obtained by analysing the simulated trajectories using Mistry's method \cite{mistry2023relative} and Nernst-Einstein equation, denoted as ``BAMBOO Mistry'' and ``BAMBOO Nernst-Einsten'', respectively. \textbf{e.} The predicted and experimental viscosity of the 7 electrolytes presented. \textbf{f.} The predicted cation transference number calculated using self-diffusion coefficients of Li$^+$ and anions of the 7 electrolytes. The tables below panels d-f describe the electrolyte composition in ``solvents$|$solvent weight $\%$$|$salt$|$salt molality'' format. All data are tabulated in Table \ref{tab:den_finetune}-\ref{tab:diff_trans_elyt}.}
    \label{fig: liq_prop}
\end{figure}

In Figure \ref{fig: liq_prop}, we present the predicted physical properties of simple solvents and electrolytes using BAMBOO compared with available experimental measurements. Figure \ref{fig: liq_prop}a displays a parity plot between the experimental and predicted densities.  
To differentiate the alignment treatment, we use red and green markers in Figure \ref{fig: liq_prop}a to indicate the systems that are included and excluded from the density alignment process, respectively. Despite the different treatment, both sets of data exhibit high R$^2$ values of 0.996, indicating excellent agreement between the predicted and experimental values. We observe that the densities of most linear solvents cluster below 1.2 g/cm$^3$, whereas those of cyclic solvent species typically register higher values. Notably, the presence of the ``C-F'' functional group leads to an increase in solvent density. This density trend by solvent category follows chemical intuition. 
The densities of LiPF$_6$-based electrolytes aggregate between 1.2 g/cm$^3$ to 1.3 g/cm$^3$, reflecting the consistent presence of roughly 1m salt (molality, in mol/kg) in these electrolytes for which experimental values are available. In contrast, experimental records of LiFSI-based electrolytes span a wider concentration range, from 0.49m to 3.74m, resulting in a broader spread of densities from 1.2 g/cm$^3$ to 1.6 g/cm$^3$. Furthermore, our model predicts the densities of EO (CH$_3$CH$_2$OH) and ACT (CH$_3$-CO-CH$_3$) with good accuracy despite their structural differences from those included in density alignment. This results may be attributed to the transferability of the alignment process using ethyl acetate (EA, CH$_3$COOC$_2$H$_5$) and other linear solvent species, underscoring the transferability of the density alignment algorithm.

Figure \ref{fig: liq_prop}b and \ref{fig: liq_prop}c illustrate the predicted viscosity values for both pure solvents and binary solvent mixtures, respectively. We specially selected these solvents to address the broader interests of the Li battery electrolyte community. In examining pure solvents, we observe good agreements between the predicted viscosity values for linear solvents (DEC, DMC, and EMC) and experimental measurements. However, some discrepancies are apparent for cyclic carbonates, particularly VC, where the MLFF underestimates its viscosity by 0.67 cP. 
It's important to acknowledge that experimental viscosity values reported in the literature for the same solvent can vary significantly. For instance, the reported viscosities for FEC at 40$^{\circ}$C range from 2.24 cP to 4.1 cP \cite{sasaki2005physical,hagiyama2008physical, janes2014fluoroethylen}. Therefore, while discrepancies exist, it remains uncertain whether the performance of BAMBOO on some carbonates is accurately assessed using the available experimental results.
Nevertheless, we can confidently assert that the differences in viscosity stemming from the categories of solvents are accurately captured by BAMBOO. Specifically, linear carbonates consistently exhibit lower viscosity compared with cyclic carbonates.

In Figure \ref{fig: liq_prop}c, we showcase the predicted binary solvent viscosity (red markers) for DMC:EC 70:30 wt$\%$ and EMC:EC 70:30 wt$\%$ as a function of temperature, contrasted with experimental results (blue markers) reported by Logan $et$ $al.$~\cite{logan2018study}. Notably, the decreasing trend depicted by the predicted values mirrors the experimental measurements. However, a consistent underestimation of viscosity by 0.2 cP is evident. Nonetheless, despite the underestimation, BAMBOO describes the trend such that EMC-EC viscosity exceeds DMC-EC.

Figure \ref{fig: liq_prop}d and \ref{fig: liq_prop}e show the conductivity and viscosity of 7 selected LiFSI- and LiPF$_6$-based electrolyte blends. Among these, the three LiFSI based electrolytes are selected to demonstrate the variations in properties with salt concentration. Meanwhile, the inclusion of four LiPF$_6$-based electrolytes aims to emphasize changes resulting from different solvents while maintaining a fixed salt concentration, as well as variations arising from different salt concentrations while keeping the solvent constant. This design is to emphasize trends and correlations in transport properties. 
It is known that conductivity and viscosity have strong correlation, such that, the lower the viscosity, the higher the conductivity. This correlation is also widely used in designing fast charging liquid electrolytes \cite{hall2018exploring,logan2018study,ma2018study}. Two methods are used to calculate conductivity, a method described by Mistry $et$ $al.$~\cite{mistry2023relative} that uses Stefan-Maxwell diffusivities, and the well-known Nernst-Einstein (NE) relation in equation \ref{eq:NE} that uses self-diffusivities of the positive and the negative ions and ignores ion-pairing and molecules' correlated motion in simulation. Due to the nature of diffusivity calculations, the conductivity via Mistry's method for a typical liquid electrolyte is always lower than the results from NE, but converges to NE at extremely low salt concentration. Therefore, the consistent lower results by Mistry's method manifest the fact that ion-pairing and correlated motion exist in the simulated electrolytes, consistent with our solvation structure analysis in Figure \ref{fig: charge} in the main text. 

In Figure \ref{fig: liq_prop}d, moving from left to right, we observe a decrease in the experimental conductivity of LiFSI-based electrolytes (F1, F2, and F3) with increasing salt concentration. This trend is effectively captured by conductivities calculated using both methods; however, Mistry's method exhibits a larger underestimation compared to NE. The associated atomic charge distributions for these three electrolytes are presented in Figure~\ref{fig: charge} to illustrate charge evolution as a function of concentration. 
Regarding LiPF$_6$-based electrolytes (P1-P4), Mistry's method yields considerably more accurate results than NE. When considering error bars, the predicted results align well with the experiments. In contrast, NE estimated-conductivities of P3 and P4 are much higher than P1 and P2, though the differences across all four blends (P1-P4) are not significant. 

Figure \ref{fig: liq_prop}e shows the predicted viscosities of electrolyte blends F1-F3 and P1-P4. Despite discrepancies in the calculated conductivities of F1-F3 compared with experimental results, the predicted viscosities generally align well with experiments, with the exception of F3. Nonetheless, BAMBOO effectively captures the increasing viscosity trend as the salt concentration rises. Although experimental records of viscosity for P1-P4 are limited, the available results indicate that BAMBOO successfully reproduces experimental viscosities for P1 and P4, consistent with its conductivity performance. 

We extract self-diffusivities ($D_{\pm, \text{self}}$) of Li$^+$ and anions from the simulated MD trajectories and subsequently compute the cation's transference number. The results are tabulated in Table \ref{tab:diff_trans_elyt}. The transference number is defined as the ratio of $D_{+,\text{self}}$ over the summation of $D_{+,\text{self}}$ and $D_{-,\text{self}}$ as shown in equation \ref{eq:diffu}. As in Figure~\ref{fig: liq_prop}f, our calculation shows that the t$_{\text{Li}^+}$ for LiPF$_6$-based electrolytes are consistent around 0.4. This finding is in line with existing literature, which reports t$_{\text{Li}^+}$ between 0.3 and 0.4 when measured using Bruce-Vincent or pfg-NMR techniques for carbonate-based electrolytes \cite{xu2022navigating}. For LiFSI-based electrolytes, we observed that the t$_{\text{Li}^+}$s are slightly higher than those in LiPF$_6$-based electrolytes, consistent with prior research comparing LiPF$_6$ and LiFSI in carbonate solvents \cite{li2010transport,takekawa2015physicochemical}. 
Furthermore, we note an increase in $t_{\text{Li}^+}$ for LiFSI-based electrolytes as the concentration rises from 1.12m to 3.74m. This observation aligns with the increasing formation of CIPs and AGGs, as illustrated in Figure \ref{fig: charge}. As the fraction of paired ions increases, the self-diffusivities of cations and anions become more correlated and similar, leading the calculated t$_{\text{Li}^+}$ to approach 0.5.
