# Supplementary material for: A predictive machine learning force field framework for liquid electrolyte development
Source: arXiv:2404.07181 source file (2025-04-01)
Supplement: Supplementary file 13 [file solvation.tex]

\section{More Solvation Structure Analyses}
\label{si:solvation}

\begin{figure}[hbt!]
    \centering
    \includegraphics[width=\textwidth]{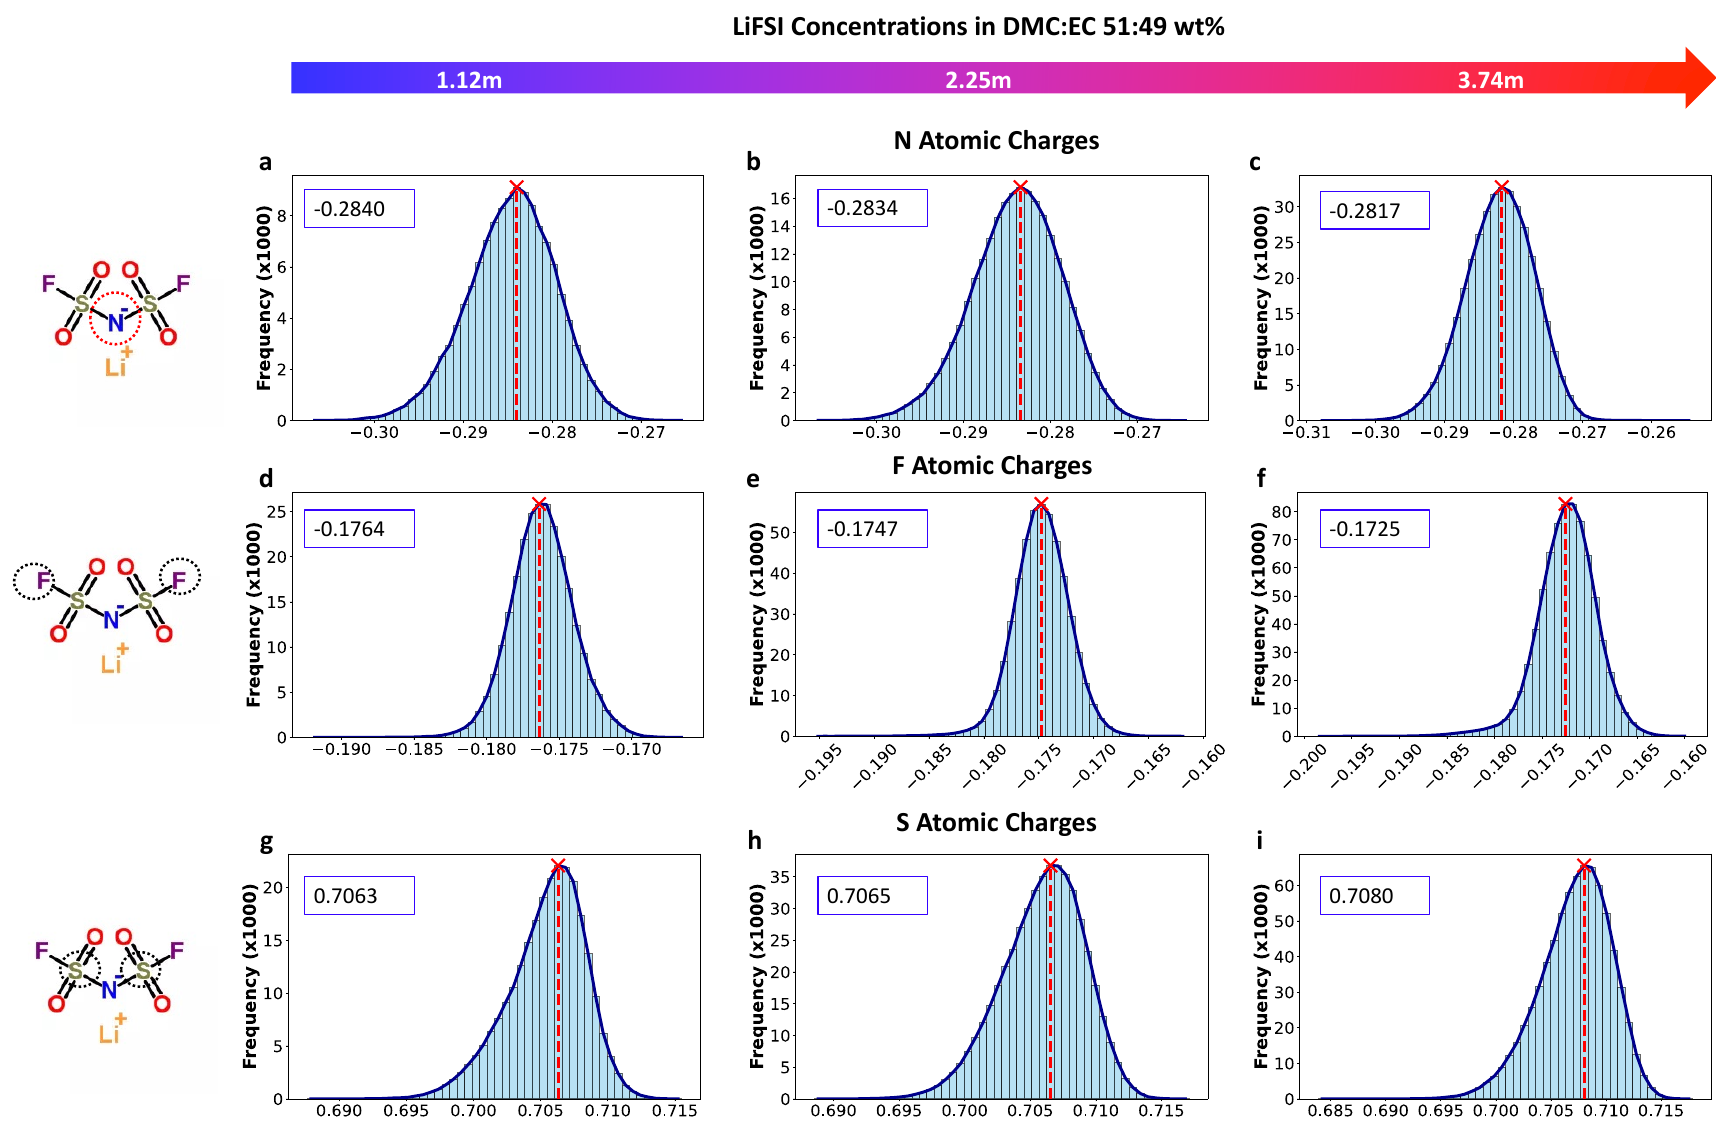}
    \caption{The atomic charge distributions of N, S, and F of the three simulated LiFSI electrolytes using BAMBOO MLFF. The electrolytes analyzed are the same systems as those shown in Figure \ref{fig: charge} and F1-F3 electrolytes shown in Figure \ref{fig: liq_prop}.}
    \label{fig:charge_N_S_F}
\end{figure}

\begin{figure}[hbt!]
    \centering
    \includegraphics[width=\textwidth]{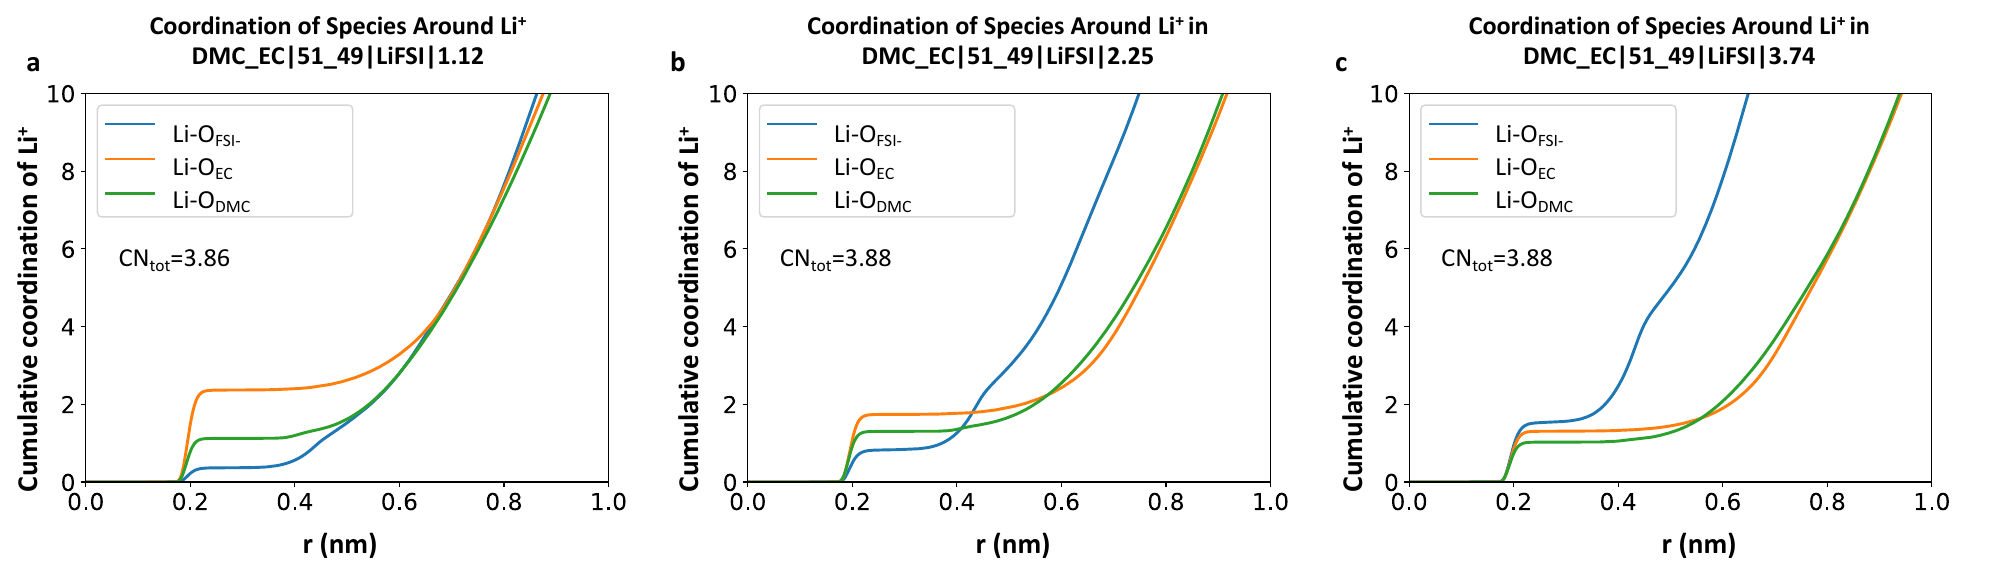}
    \caption{The cumulative coordination of solvent and anion species around Li$^+$. \textbf{a-c} show the results of electrolytes 1.12m, 2.25m, and 3.74m LiFSI in DMC:EC 51:49 wt$\%$, respectively. The total coordination numbers for each simulated system is presented in each figure panel. The legends indicate the coordination is obtained by analyzing the atomise interactions between Li$^+$ and the Os of surrounding solvents and anion molecules. The electrolytes analyzed are the same systems as those shown in Figure \ref{fig: charge} and F1-F3 electrolytes shown in Figure \ref{fig: liq_prop}.}
    \label{fig:cn_Li}
\end{figure}

The charge histograms shown in Figure~\ref{fig: charge} and Figure \ref{fig:charge_N_S_F} are derived by first collecting atomic partial charges from each frame of a 4ns simulation, totalling 4,000 frames, followed by histogram analyses. The peaks corresponding to each normal distribution in the figure panels are identified using the \textit{find-peaks} function as implemented in \textit{scipy.signal} module. The solvation structures were determined by extracting Li clusters using \textit{MDAnalysis} \cite{michaud2011mdanalysis} with radius cut-off 2.2\AA~determined from Li-FSI radial distribution functions. This information can be read from the cumulative coordination around Li$^+$ presented in Figure \ref{fig:cn_Li}. The frames involved in the cluster extraction are in consistent with the charge histograms. 

In Figure~\ref{fig: charge} in the main text, we observe that with increasing concentration, there is a rise in the fraction of Li ions with lower atomic charges. O$_{\text{FSI}^-}$ also shows such a trend. This observation may initially appear counter-intuitive, as it suggests the Li charge decreases did not end up being taken by O$_{\text{FSI}^-}$s. Upon analyzing the charge histograms of N, F, and S in Figure~\ref{fig:charge_N_S_F}, we observe consistent shifts in the distribution peaks from more negative to more positive values. These shifts, totaling 0.014, likely indicate that atomic charges moved away from Li ions being compensated by N, F, and S, along with other solvent molecules.

The results presented in this work show that the charges of Li$^+$ and other atomic species are not fixed, rather, they changes as electrolyte compositions. In liquid electrolyte simulations, accurately capturing polarizability is crucial for describing Li$^+$ transport properties. However, classical force fields often fall short in this aspect. A typical treatment in classical MD using a non-polarizable force field is to scaling the ions' and solvents' charges \cite{chen2016polymer, gudla2020effects} to match experimental properties, such as self-diffusivities for specific systems of interest. The goal is to provide a mean-field representation of charge screening \cite{mistry2022toward}. However, different scaling factors are required when investigating different electrolyte chemistries or compositions, leading to limited generalizability. Determining the optimal charge scaling scheme typically relies on Li$^+$ self-diffusivity data obtained from Nuclear Magnetic Resonance Spectroscopy (NMR) \cite{gudla2020effects}, which can be costly and time-consuming, and sometimes defeat the purpose of novel liquid electrolyte exploration. Therefore, given the generalizability and flexibility of BAMBOO in providing solvation insights, there exists an unique opportunity for MLFF to participate in ``bottom-up'' understanding \cite{mistry2022toward} and design of liquid electrolytes.

% Figure \ref{fig:charge_N_S_F} represents the atomic partial charges of N, F, and S of FSI$^-$ anions in LiFSI-based electrolytes that have 1.12m, 2.25m, and 3.74m salt in DMC:EC 51:49 wt$\%$ solvent. These results, together with the partial charge distributions of Li$^+$ and O$_{\text{FSI}^-}$ presented in Figure \ref{fig: charge} demonstrate the partial charge variations as a function of salt concentrations, and the correlation to the solvation structures. The dotted red lines in figure panels indicate the partial charge values that are associated with the distribution peaks. These values are included in each panel as the legend. We find the peak partial charge values shift slightly to more positive as salt concentration increases. The positive shifts may compensate the increased fractions of Li$^+$ and O$_{\text{FSI}^-}$ with lower partial charge values. 
