# Supplementary material for: A predictive machine learning force field framework for liquid electrolyte development
Source: arXiv:2404.07181 source file (2025-04-01)
Supplement: Supplementary file 14 [file training.tex]

\subsection{Initial Training of BAMBOO}
\label{si:training}
Given the design of the GET architecture and the prediction of energy, force, virial and dipole, we use the following loss function to train the neural networks in BAMBOO:

\begin{equation}
    \begin{split}
    L_{\text{training}} = \frac{1}{N_{\text{cluster}}} \sum_{k}^{N_{\text{cluster}}}\sum_{i}^{N_{\text{atom}}}&(\alpha_{\text{energy}}^{\text{training}} (E_{k}^{\text{DFT}} - E_{k}^{\text{BAMBOO}})^{2} \\
         &+ \frac{1}{N_{\text{atom}}}\alpha_{\text{force}}^{\text{training}} ||\Vec{f}_{k,i}^{ \text{DFT}} - \Vec{f}_{k,i}^{ \text{BAMBOO}}||^{2} \\
         &+ \alpha_{\text{virial}}^{\text{training}} ||\textbf{T}_{k}^{\text{DFT}} - \textbf{T}_{k}^{\text{BAMBOO}}||^{2} \\
         &+ \frac{1}{N_{\text{atom}}}\alpha_{\text{charge}}^{\text{training}} (q_{k,i}^{\text{DFT}} - q_{k,i}^{\text{BAMBOO}})^{2} \\
         &+ \alpha_{\text{dipole}}^{\text{training}} ||\Vec{D}_{k}^{ \text{DFT}} - \Vec{D}_{k}^{ \text{BAMBOO}}||^{2}  \\
         &+ \frac{1}{N_{\text{atom}}}\alpha_{\text{Qeq}} ||\Vec{f}_{k,i}^{ \text{elec, BAMBOO}} - \Vec{f}_{k,i}^{ \text{elec*, BAMBOO}}||^{2} ),
    \end{split}
    \label{trainingloss}
\end{equation} where $\alpha_{\text{energy}}$ is the weight associated with energy in the loss function, and so on. Here, $q^{\text{DFT}}$ is the CHELPG~\cite{chelpg}, which is a partial charge that is fitted to the electrostatic potential outside the cluster. From equation~\eqref{trainingloss}, we can see that the charge learned by BAMBOO is determined by four aspects: the first is to fit energy, force, and virial together with the contribution from the neural network; the second is to fit the electrostatic potential by fitting CHELPG; the third is to fit dipole moment, a macroscopic observable derived from charge densities by density functional theory (DFT); and the fourth is to approximate charge equilibrium as in equation~\eqref{qeqloss}. In Figure \ref{dft_parity}a, b, and c, we show that BAMBOO can learn and predict DFT computed energy, force, and virial very accurately with $R^{2}$ scores higher than 0.99. As in Figure~\ref{fig:dipole_esp}, we can see that both dipole moment and electrostatic potential, two observables largely affect inter-molecular interactions, can be accurately predicted with R$^2$ scores higher than 0.98. For dipole moment, we observe some outliers in Figure \ref{fig:dipole_esp}a, which are mostly clusters with delocalized electrons, such as those with Li clusters. Since the concept of atomic partial charge cannot well capture delocalized charge density distribution, in future works we will try to tackle this issue through more sophisticated representations of charge density, and the concept of Wannier functions\cite{wannier} might be an option. 

\begin{figure}
    \centering
    \includegraphics[width=\textwidth]{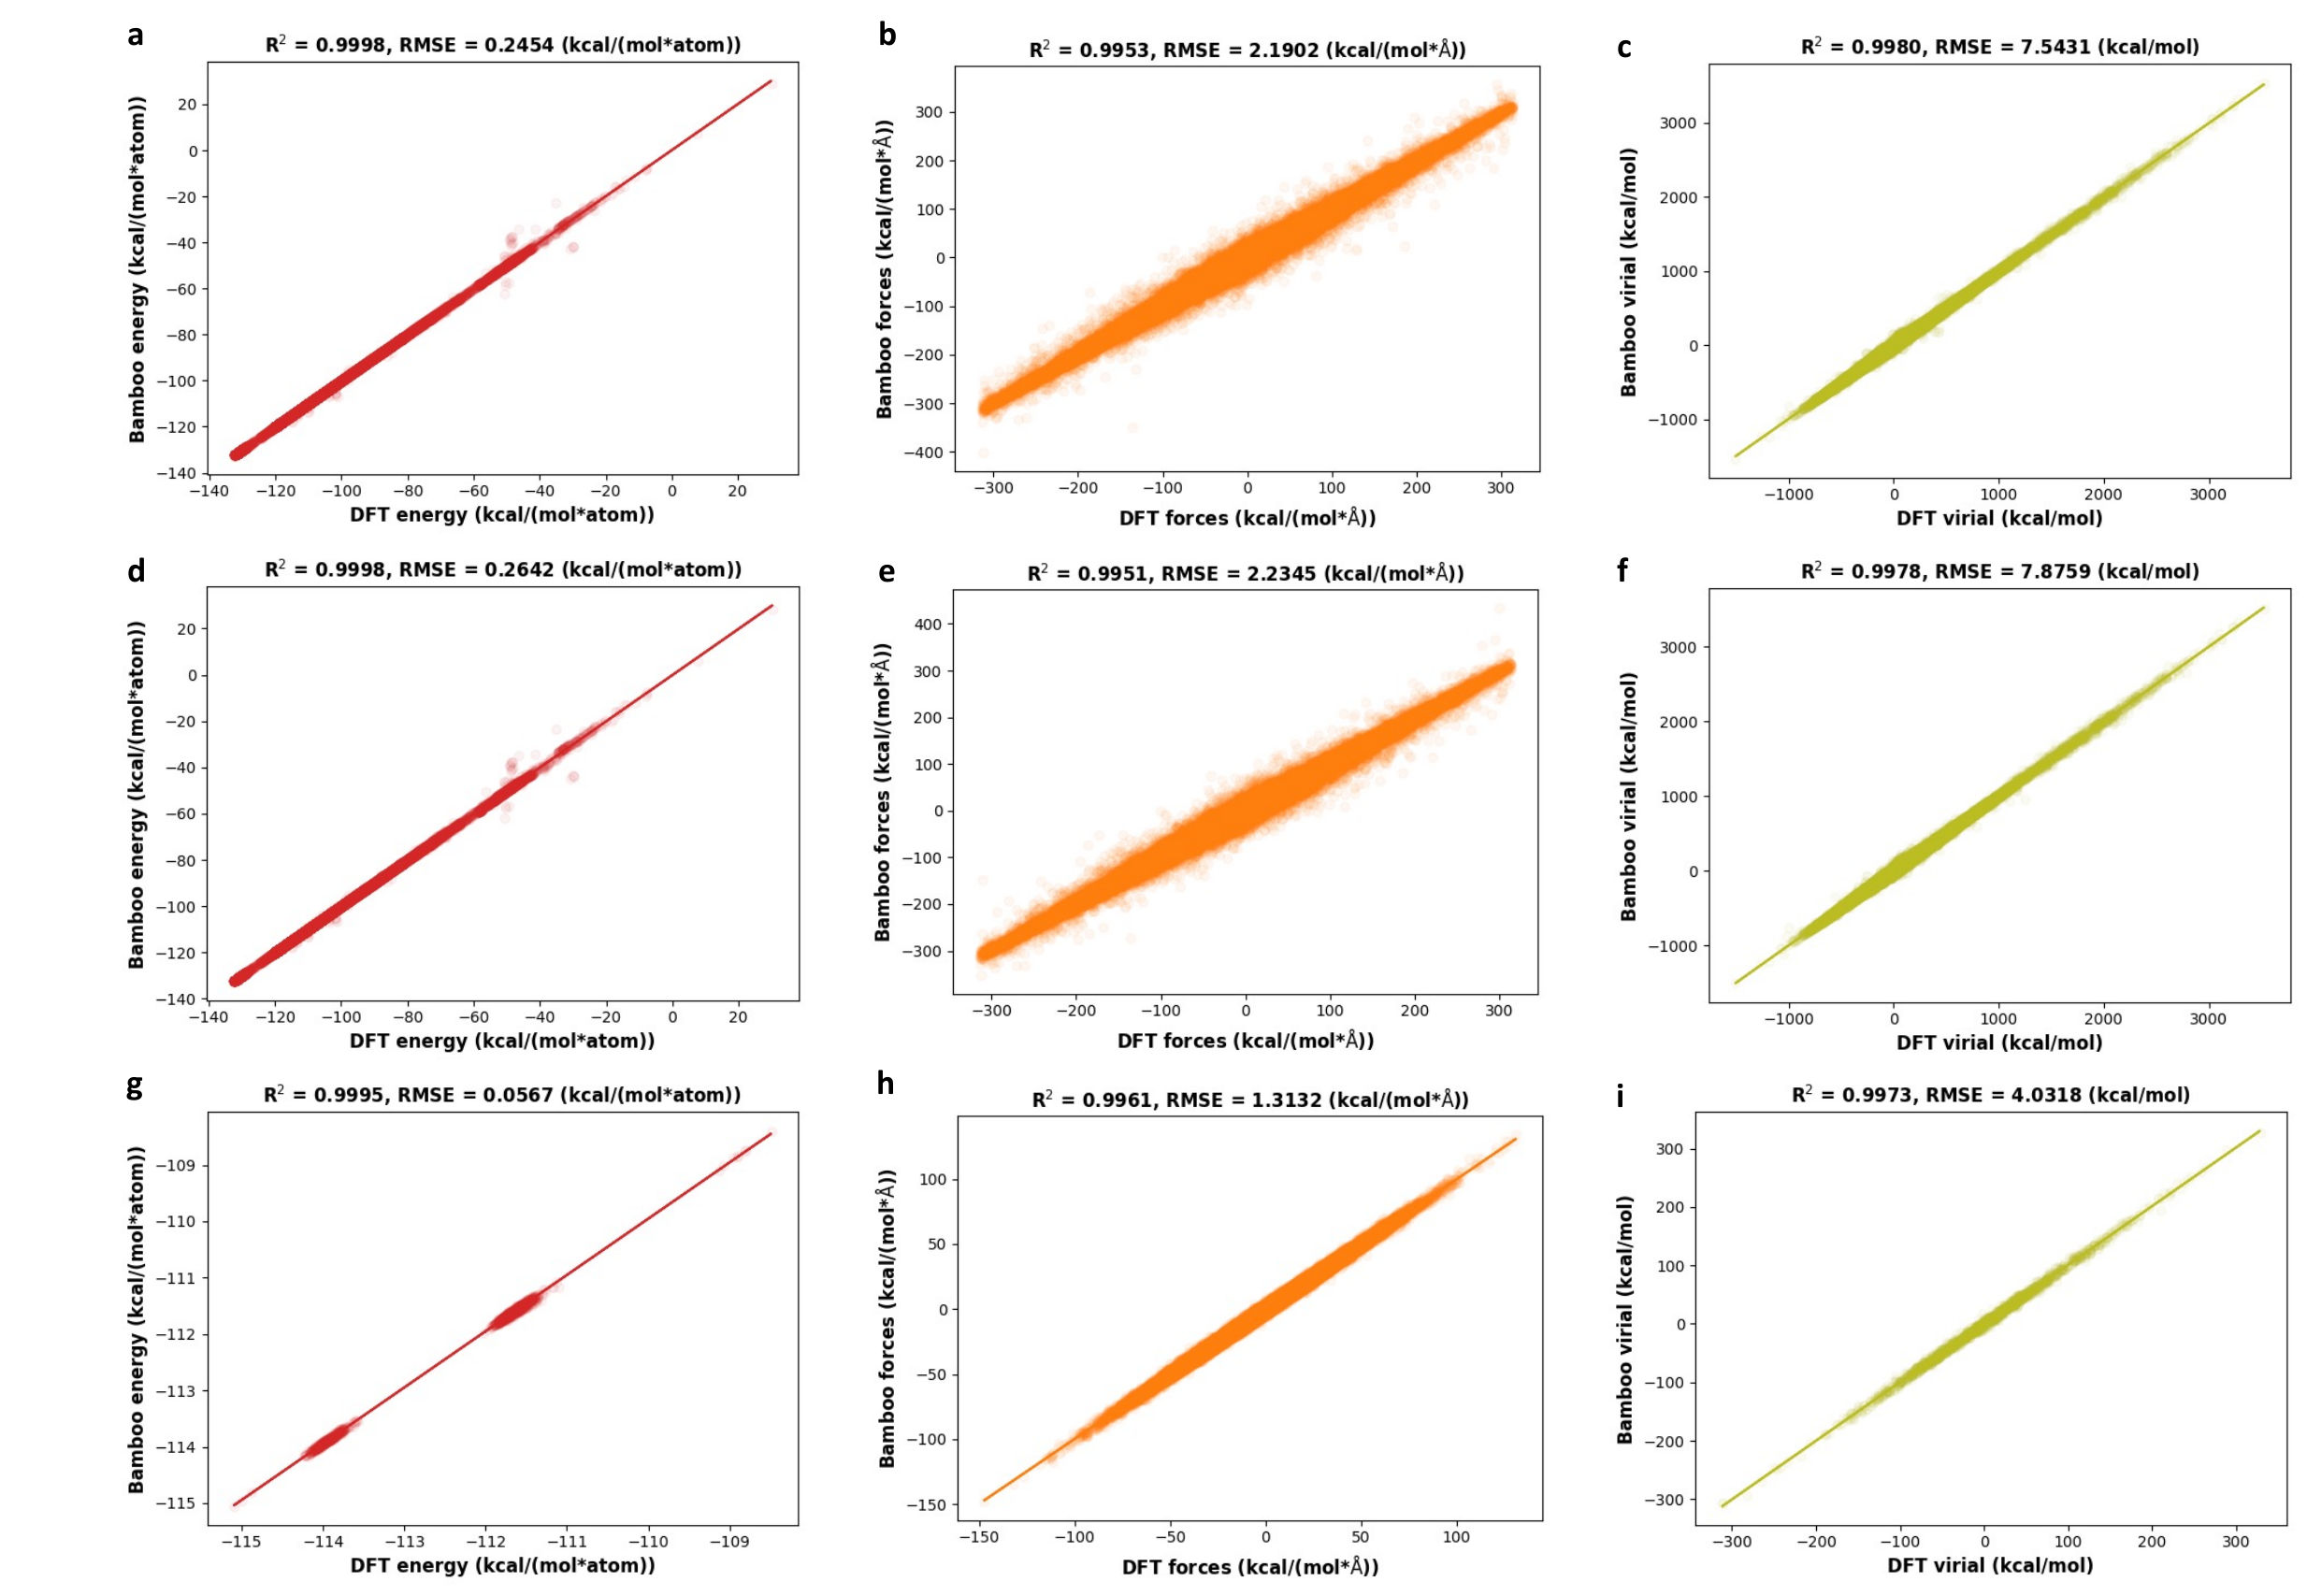}
    \caption{Fitting performance of BAMBOO before and after ensemble knowledge distillation and density calibration. \textbf{a, b, c.} DFT computed energy, force, and virial versus BAMBOO predicted quantities before ensemble knowledge distillation and density calibration, respectively. \textbf{d, e, f.} DFT computed energy, force, and virial versus BAMBOO predicted quantities after ensemble knowledge distillation and density calibration, respectively. The results are based on the validation set. \textbf{g, h, i.} DFT computed energy, force, and virial versus BAMBOO predicted quantities for the test set sampled from the production MD simulations, respectively.}
    \label{dft_parity}
\end{figure}

\begin{figure}
    \centering   \includegraphics[width=1.0\textwidth]{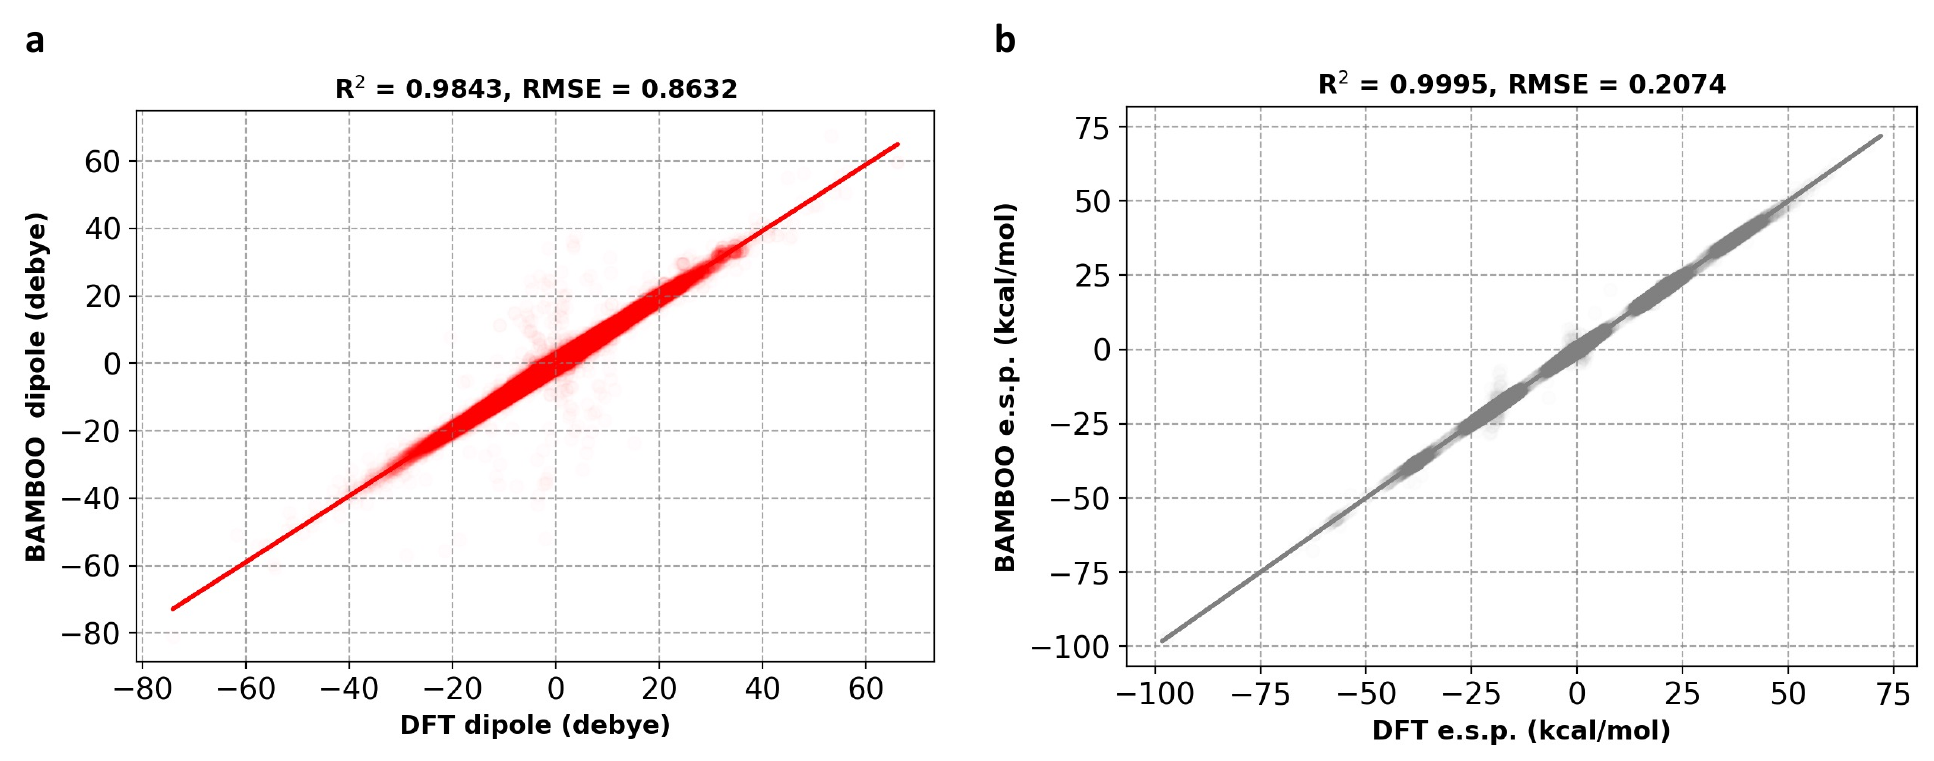}
    \caption{\textbf{Dipole moment and electrostatic potential by DFT and BAMBOO} \textbf{a}, \textbf{b.} DFT computed dipole moment and electrostatic potential (abbreviated as "e.s.p.") versus BAMBOO predicted quantities, respectively. The results are based on the DFT validation set. Electrostatic potential is sampled at grid points 10\AA\ away from the geometric center of the cluster.}
    \label{fig:dipole_esp}
\end{figure}

Here, we build the neural networks in BAMBOO by PyTorch~\cite{pytorch}, and we use the AdamX optimizer~\cite{kingma2017adam} with the learning rate of $10^{-2}$. In the training process, weight decay is set to 0.001, while the learning rate decreases at a rate of 0.99. The batch size is 128 for both training and validating. The training process is composed of 750 training epochs. The model consists of 3 layers, with 32 radial basis functions for edges and an embedding dimension of 64 for nodes. It features 16 attention heads, employs a cutoff radius of 5.0 \AA~for each message passing layer, and includes the MLP with two layers for predicting energy and charge. The loss weights $\alpha$'s in equation~\eqref{trainingloss}  are provided as the default in the open source codes at~\cite{BAMBOOGITHUB} and listed in Table~\ref{tab:hyper-parameters}. 

\begin{table}[h!]
  \centering
  \caption{Table of loss weights.}
  \label{tab:hyper-parameters}
  \vskip 0.1in
  \begin{tabular}{ccccccc} 
    \toprule
    Loss weights & $\alpha_{\text{energy}}^{\text{training}}$ & $\alpha_{\text{force}}^{\text{training}}$ & $\alpha_{\text{virial}}^{\text{training}}$ &
    $\alpha_{\text{charge}}^{\text{training}}$ &
    $\alpha_{\text{dipole}}^{\text{training}}$ &
    $\alpha_{\text{Qeq}}$ \\
    \midrule
     Value & 0.01 & 0.3 & 0.01 & 10.0 & 10.0 & 300.0  \\
    \bottomrule
  \end{tabular}
\end{table}
