# Supplementary material for: A predictive machine learning force field framework for liquid electrolyte development
Source: arXiv:2404.07181 source file (2025-04-01)
Supplement: Supplementary file 15 [file transferability.tex]

\section{Transferability to Unseen Molecules}
\label{si:transferability}

\begin{figure}
    \centering   \includegraphics[width=1.0\textwidth]{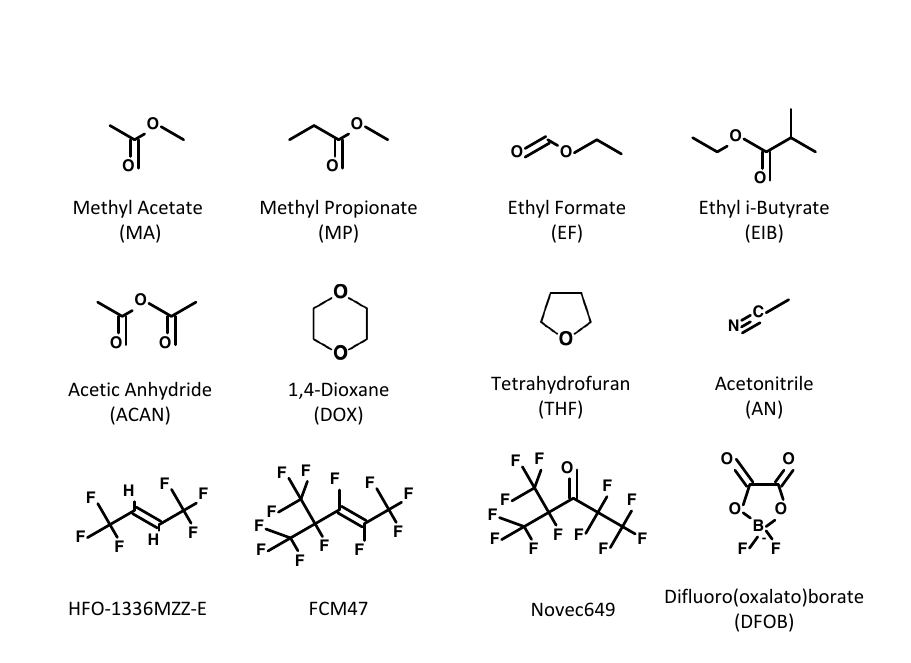}
    \caption{Schematic of the unseen species used for testing the transferability of BAMBOO.}
    \label{fig:new_molecules}
\end{figure}

\begin{table}[hbt!]
\caption{The stability, density ($\rho$, in g/cm$^{3}$), and viscosity ($\eta$, in cP) of new unseen molecules/salt in Figure~\ref{fig:new_molecules} from MD simulations powered by BAMBOO and OPLS-AA. The uncertainty for the density calculated using BAMBOO and OPLS-AA ranges from 0.001 to 0.004 g/cm$^{3}$. The uncertainty for the viscosities calculated using BAMBOO and OPLS-AA ranges from 0.008 to 0.176 cP. For clarity, we do not show simulated properties which cannot be stably simulated by BAMBOO or do not have corresponding experimental values to compare.}
\label{tab:newmolecules}
\vskip 0.15in
\begin{center}
\begin{tabular}{lcccccccr}
\toprule
\small

Molecule&Stable&$\rho_{\text{BAMBOO}}$&$\rho_{\text{OPLS-AA}}$&$\rho_{\text{Exp}}$&$\eta_{\text{BAMBOO}}$&$\eta_{\text{OPLS-AA}}$&$\sigma_{\text{Exp}}$\\

\midrule
MA & Yes & 1.02 & 0.953 & 0.938~\cite{MA} & 0.831 & 0.610 & 0.385~\cite{MA} \\
MP & Yes & 0.984 & 0.922 & 0.915~\cite{MP} & NA & NA & NA \\
EF & Yes & 0.924 & 0.946 & 0.922, 0.917~\cite{EF} & 0.649 & 0.637 & 0.49~\cite{schrodinger_viscosity} \\
EIB & Yes & 0.829 & 0.890 & 0.865~\cite{crchandbook} & 0.524 & 0.839 & 0.56~\cite{schrodinger_viscosity} \\
ACAN & Yes & 1.014 & 1.077 & 1.080~\cite{crchandbook} & 0.880 & 1.777 & 0.85~\cite{ACAN} \\
DOX & Yes & 1.021 & 0.981 & 1.030~\cite{crchandbook} & 0.673 & 0.667 & 1.20~\cite{DOX} \\
THF & No & NA & NA & NA & NA & NA & NA \\
AN & No & NA & NA & NA & NA & NA & NA \\
HFO-1336MZZ-E & Yes & 1.488 & 1.346 & 1.413~\cite{crchandbook} & NA & NA & NA \\
FCM47 & Yes & 1.571 & 1.674 & 1.601~\cite{FCM47} & NA & NA & NA \\
Novec649 & Yes & 1.670 & 1.746 & 1.600~\cite{novec649} & 1.381 & 0.666 & 0.64~\cite{novec649} \\
EC$|$LiDFOB$|$0.25 & No & NA & NA & NA & NA & NA & NA \\
\bottomrule

\end{tabular}
\end{center}
\vskip -0.1in
\end{table}

To satisfy the potential interest in exploring novel solvent derivatives completely \textit{in silico}, in this section we assess the generalizability of the current BAMBOO model to unseen molecules not included in the DFT dataset, probing its capability limitations and providing guidance for further improvement. 

We first conduct MD simulations on 12 new unseen molecules/salt as in Figure~\ref{fig:new_molecules}. In Table~\ref{tab:newmolecules}, we list whether the BAMBOO-based MD simulations for each specie is stable without spurious reactions, and the simulated density and viscosity from BAMBOO and OPLS-AA~\cite{oplsaa}. We can see that, BAMBOO can stably simulate unseen molecules with bonding types similar to those included in the training set in Figure S1 in the Supplementary Information. However, we find that for species with unseen element (such as B in DFOB) and unseen bond types (such as the triple bond in AN and the dihedral of four carbon atoms in THF), BAMBOO cannot achieve long-time stable MD simulations. For the remaining molecules that can be stably simulated by BAMBOO, we can see that BAMBOO has the density MAE of 0.0495 g/cm$^{3}$ and the mean viscosity deviation of 52.4\%, which is higher than that of systems included in the training set (0.011 g/cm$^{3}$ and 16.7\%). As comparison, for the same systems in Table~\ref{tab:newmolecules}, the density MAE of OPLS-AA is 0.0454 g/cm$^{3}$ and the mean viscosity deviation of OPLS-AA is 49.3\%. In practice, we recommend that for unseen species, people should first use classic force fields such as OPLS-AA to obtain rough estimation of bulk properties as OPLS-AA restricts bond-breaking from happening, then construct DFT datasets and train machine learning force fields such as BAMBOO to more accurately study molecules of interest.

In Figure~\ref{fig:density_versus_vis_cond}, we show the strong linear dependence of viscosity and ionic conductivity on density: a denser liquid exhibits stronger inter-molecular interactions, resulting in higher viscosity and lower conductivity. From Table~\ref{tab:newmolecules}, we observe that, for systems where BAMBOO considerably overestimates densities compared with OPLS-AA and experiment, such as MA and Novec649, we also observe overestimated viscosities from BAMBOO. The simultaneous overestimation of density and viscosity aligns with the relation between density and viscosity, which also implies that, for unseen molecules, the tendency of BAMBOO to overestimate or underestimate viscosity could be speculated by the behavior of density prediction. 
As for ionic conductivity, we can also speculate its transferability from the behaviors of density and viscosity predictions. For example, since BAMBOO overestimates the density and viscosity of MA, we expect that the ionic conductivity of electrolytes containing MA would be underestimated. For example, for the system DMC\_EC\_MA$|$30\_40\_30$|$LiPF$_{6}$$|$0.50, its experimental viscosity and conductivity are 1.09 cP and 12.83 mS/cm, respectively~\cite{logan2018study}. As anticipated, BAMBOO overestimates its viscosity (1.80 $\pm$ 0.02 cP) and underestimates its conductivity (10.45 $\pm$ 0.35 mS/cm). 

To further reveal the trend of density prediction on unseen molecules, we further conduct MD simulations on fluorinated solvent molecules.
In advanced electrolytes, fluorination of a base solvent is a commonly used strategy \cite{yu2022tuning,zhao2023electrolyte} to enhance electrochemical performance \cite{yue2018synthesis}, LiF-rich SEI formation \cite{zhu2018fluoroethylene}, and fire-resisting property \cite{an2021design}. Despite the popularity and effectiveness of fluorination, the exact relationship of the location and the degree of fluorination to the liquid electrolyte performances are not clear. This underscores the importance to incorporate MLFF in structural-based electrolyte design. 
The parent molecules, EC, DMC, and EA and their derived child molecular structures are shown in Figure \ref{fig:transferability}a, c, and e. All child molecules are excluded from training or alignment, except FEC. 
The same BAMBOO model used for generating the liquid electrolyte properties shown in Figure \ref{fig: liq_prop} is used in the transferability study. 
We find all simulations of the child solvents remain stable during the 5 ns MD simulations within a broad temperature range of 283-343 K, demonstrating the high transferability of the model. 

In Figure \ref{fig:transferability}b, d, and f, we present the simulated densities of the fluorinated derivatives from BAMBOO MD simulations and experiments as a function of temperatures. Qualitatively, we find that, except for the fluorinated EAs (FEA, EFA), which have very similar structures and experimental densities, BAMBOO can correctly predict the density trends of fluorinated ECs and DMCs. To be specific, the trend cis-DFEC $>$ DFEC $>$ trans-DEFC, and the trend FDMC $>$ DFDMC $>$ MFDMC are reproduced. The trend for DMC derivatives follows the intuition that as the fluorination increases, density increases.
In addition, we find that the more structural-alike the unseen child molecule compared with the parent molecule, the more accurate the prediction of density from BAMBOO is. Furthermore, the inclusion of the functional group of interest in training data is crucial for accuracy. For instance, since FEC is already included in the DFT dataset, the density discrepancy of other fluorinated derivatives of EC from BAMBOO are within 0.03 g/cm$^3$ compared with that from experiments. As a comparison, since there is no fluorinated derivative of EA and DMC in the DFT dataset, the density errors of the simulated results for fluorinated EA and DMC are generally at the order of 0.1 g/cm$^3$, which is larger than that of fluorinated EC. Specifically, with higher degree of fluorination, we can see that the density error of DMC's child molecules becomes larger, from around 0.05 g/cm$^3$ for MFDMC, 0.08 g/cm$^3$ for DFDMC, to 0.20 g/cm$^3$ for TFDMC. The comparison between EC and DMC derived molecules indicate that BAMBOO has the potential to transfer to unseen molecules in terms of calculating density but requires small amount of DFT training data describing the specific functional groups and types of molecular backbone. Here, we speculate the accuracy of density predictions to the fluorinated EAs and DMCs can be improved by including ``-CH$_2$F'' and ``-CHF$_2$'' functional groups in the DFT dataset, which will be incorporated in a later version of BAMBOO. 

To make machine learning force field more transferable to out-of-sample systems, we need constant effort to improve the MLFFs. In general, there are two approaches to elevate the transferability of MLFFs. The first approach is to conduct large scale pretraining on datasets with diverse molecules, such as the MACE-OFF23~\cite{maceoff23} which is trained on nearly a million molecules. Although the strategy of large scale pretraining is very popular in the recent wave of universal force fields~\cite{m3gnet, chgnet, genome, dpa2, macemp, aimnet, maceoff23}, it requires careful design of the dataset for the trade-off between effectiveness and efficiency, and it is not proved to guarantee stable MD simulations for all molecules. The other approach is to combine machine learning model with strong physical restrictions, such as our latest work that employs machine learning models to parameterize force fields with classic functional forms~\cite{byteff}, which ensures that the force field can stably simulate any molecule without spurious reaction during the MD simulation. However, such restrictions also limit the usage of machine learning force field on cases where bond breaking happens. Therefore, we think it is important to further develop machine learning force field that can stably simulate as much molecules as possible while preserve the ability to model bond breaking events when necessary. In the very recent work by Niblett $et$ $al.$~\cite{niblett2024transferability}, it is shown that the GNN based model is more transferable to new molecules than local descriptors-based model, which we hope can inspire further development of machine learning architecture for higher transferability of force fields. 

\begin{figure}
    \centering   \includegraphics[width=1.0\textwidth]{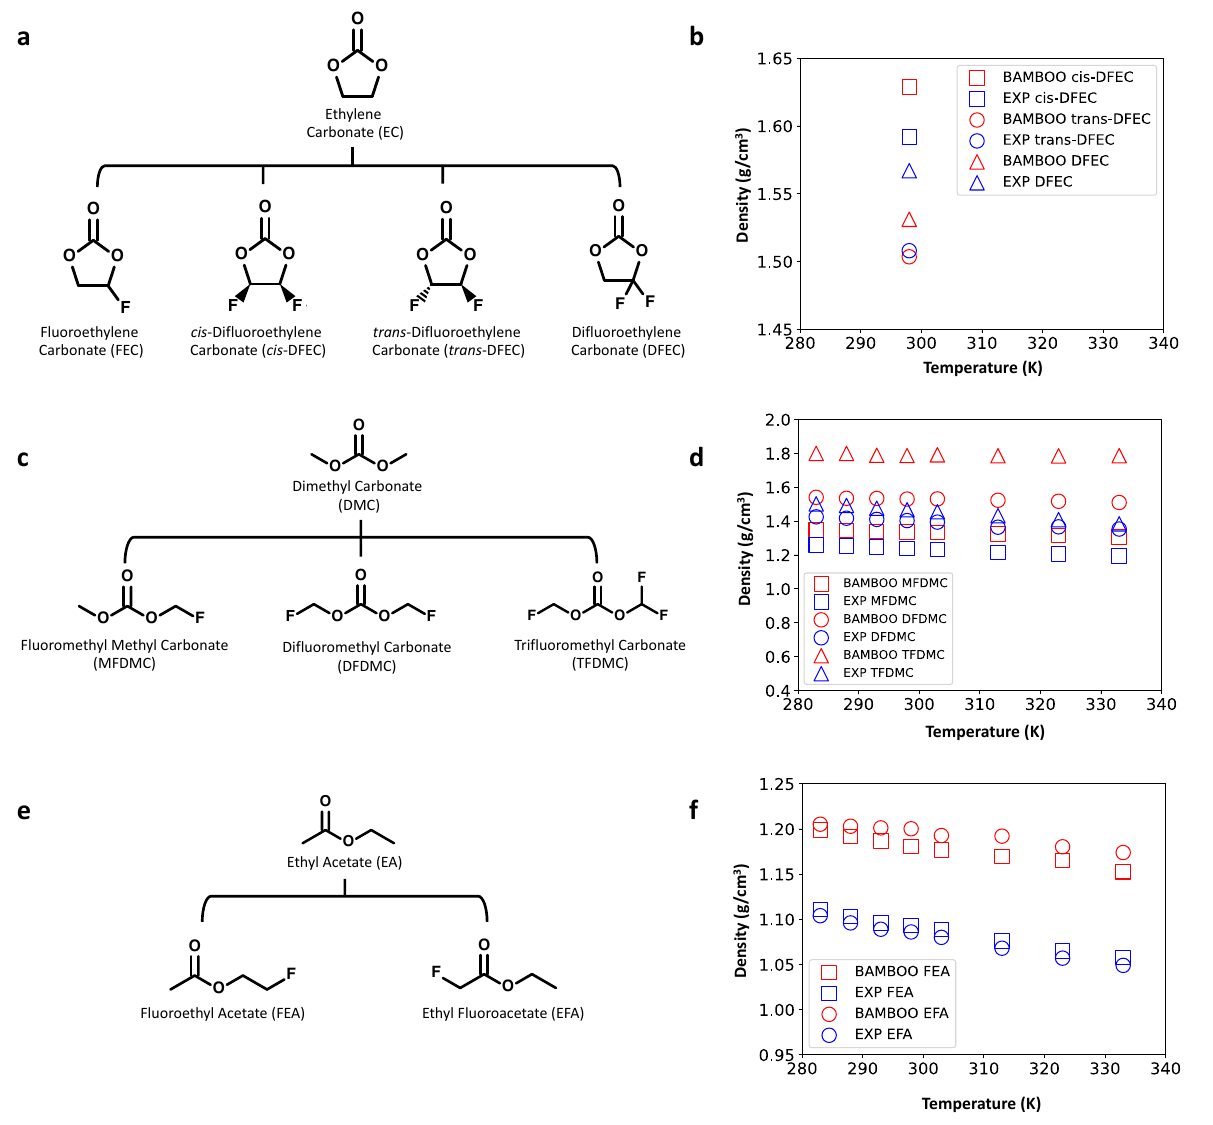}
    \caption{\textbf{Transferability of BAMBOO to unseen fluorinated molecules.} \textbf{a}, \textbf{b.} Illustration of fluorinated EC molecules and densities of the EC derivatives from BAMBOO and experiment, respectively. \textbf{c}, \textbf{d.} Illustration of fluorinated DMC molecules and densities of the DMC derivatives from BAMBOO and experiment, respectively. \textbf{e}, \textbf{f.} Illustration of fluorinated EA molecules and densities of the EA derivatives from BAMBOO and experiment, respectively.}
    \label{fig:transferability}
\end{figure}
